# Supplementary material for: A Latent Fingerprint in the Wild Database
Source: arXiv:2304.00979 source file (2023-04-03)
Supplement: Supplementary file 1 [file SUPPLEMENTARY_MATERIAL.pdf]

# Supplementary Material

## A. Supplementary results for the overall comparison experiments

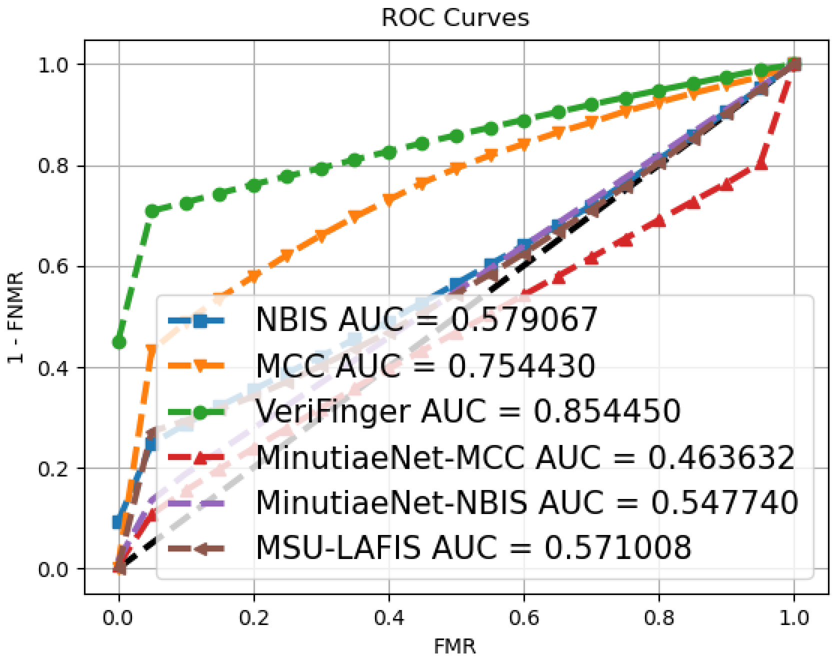


Fig. 13: ROC curve of the overall comparison experiments for the 'Latent in the Wild' database

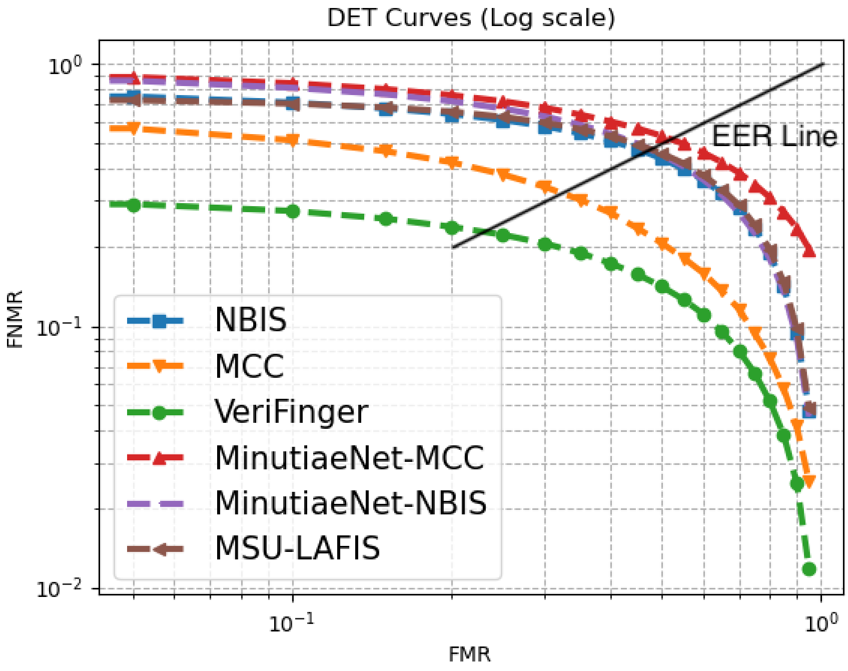


Fig. 14: DET curve of the overall comparison experiments for the 'Latent in the Wild' database

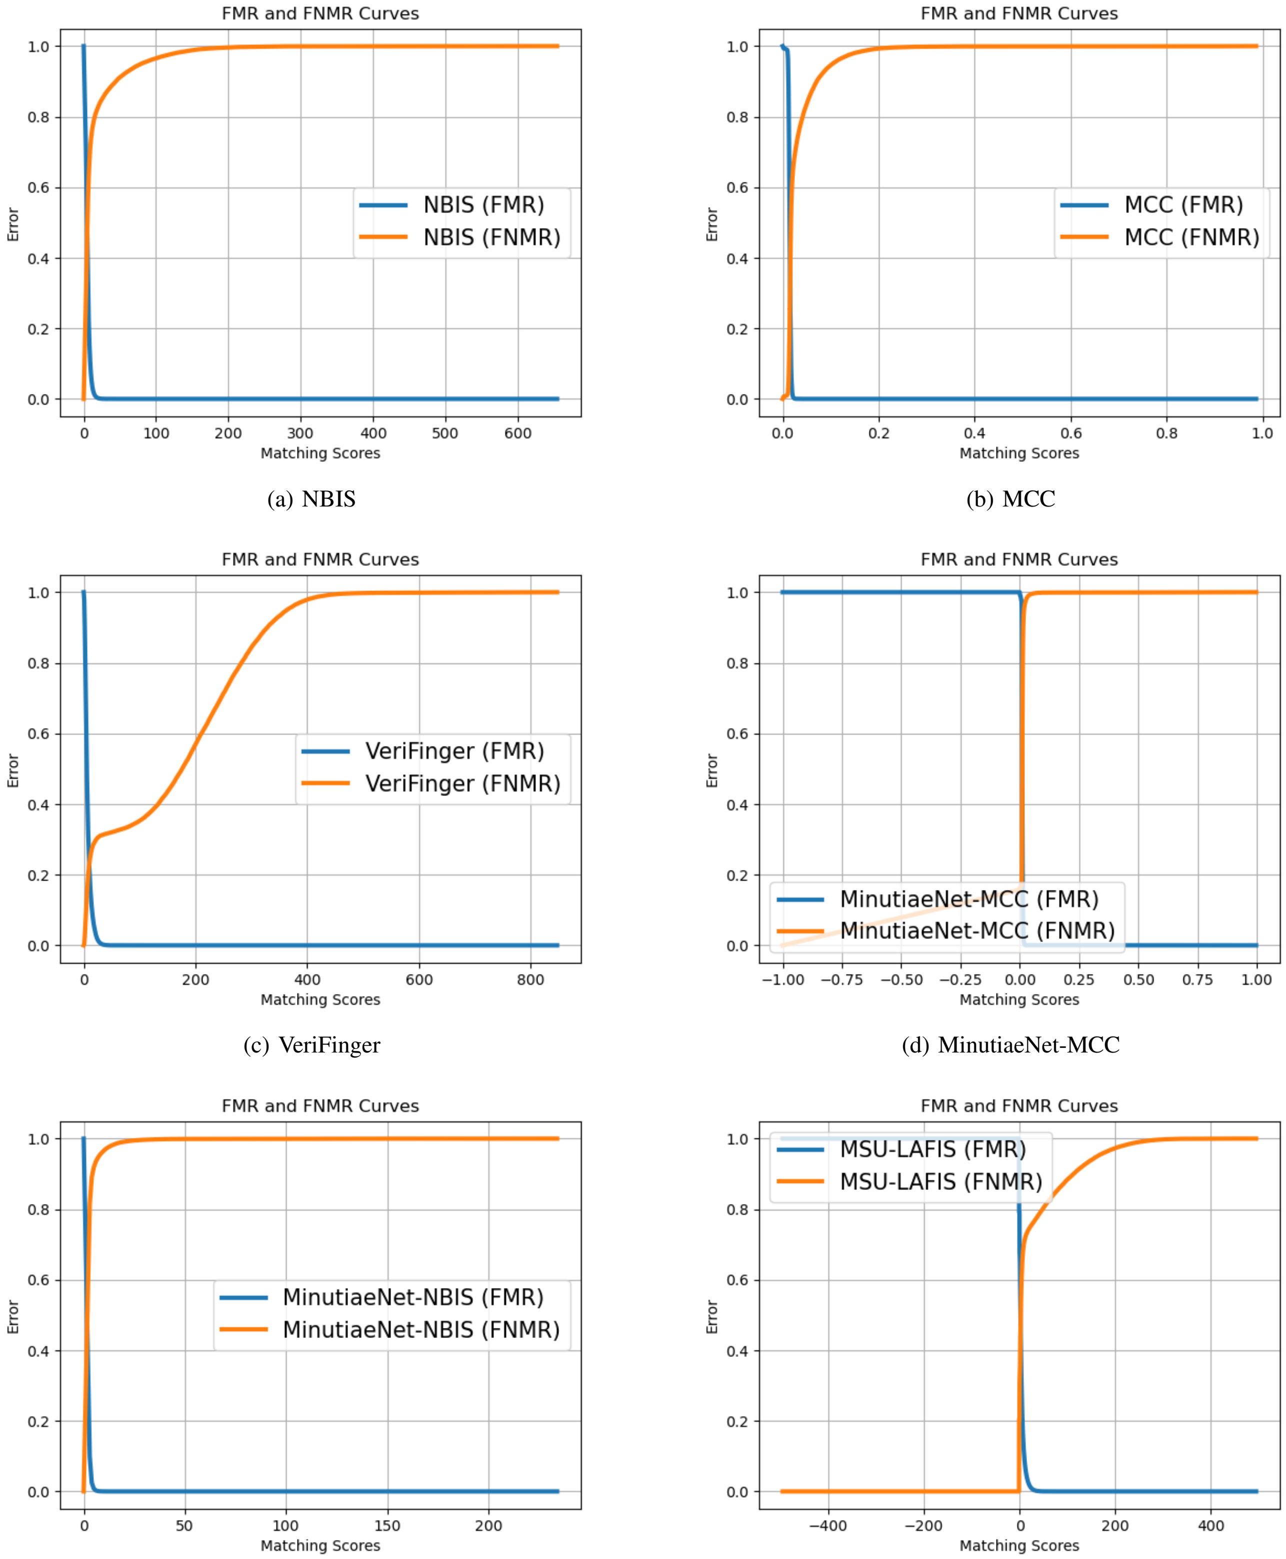


(a) NBIS

(b) MCC

(c) VeriFinger

(d) MinutiaeNet-MCC

(e) MinutiaeNet-NBIS

(f) MSU-LAFIS

Fig. 15: FMR and FNMR curves of the overall comparison scores in the 'Latent in the Wild' database

TABLE XII: Performance indicators measured on the 'Latent in the Wild' database for the overall comparison experiments.

| Algorithm | GMean | GSTD | IMean | ISTD | SI | AUC | JI | JI_TH | MCC |
|---|---|---|---|---|---|---|---|---|---|
| NBIS | 15.207 | 32.128 | 4.222 | 3.594 | 0.481 | 0.579 | 0.198 | 12.000 | 0.371 |
| MCC | 0.032 | 0.043 | 0.015 | 0.003 | 0.592 | 0.754 | 0.389 | 0.017 | 0.447 |
| VeriFinger | 162.662 | 128.209 | 6.788 | 5.728 | 1.718 | 0.854 | 0.685 | 33.000 | 0.810 |
| MinutiaeNet-MCC | -0.146 | 0.370 | 0.011 | 0.002 | 0.603 | 0.464 | 0.058 | 0.015 | 0.139 |
| MinutiaeNet-NBIS | 1.305 | 5.109 | 0.336 | 1.042 | 0.263 | 0.548 | 0.088 | 3.000 | 0.200 |
| MSU-LAFIS | 28.867 | 56.745 | 3.550 | 5.340 | 0.628 | 0.571 | 0.237 | 22.147 | 0.395 |
| | | | | | | | | | |
| Algorithm | MCC_TH | EERL | EERH | EER | 0FMR | FMR1000 | FMR100 | FMR20 | FMR10 |
| NBIS | 21.000 | 0.444 | 0.478 | 0.461 | 0.908 | 0.842 | 0.806 | 0.753 | 0.709 |
| MCC | 0.036 | 0.323 | 0.323 | 0.323 | 0.998 | 0.689 | 0.636 | 0.568 | 0.512 |
| VeriFinger | 47.000 | 0.226 | 0.230 | 0.228 | 0.551 | 0.315 | 0.308 | 0.291 | 0.275 |
| MinutiaeNet-MCC | 0.022 | 0.519 | 0.519 | 0.519 | 0.994 | 0.970 | 0.943 | 0.892 | 0.846 |
| MinutiaeNet-NBIS | 7.000 | 0.099 | 0.813 | 0.456 | 0.986 | 0.945 | 0.919 | 0.891 | 0.813 |
| MSU-LAFIS | 65.715 | 0.475 | 0.475 | 0.475 | 1.000 | 0.781 | 0.754 | 0.728 | 0.707 |
| | | | | | | | | | |
| Algorithm | 0FNMR | EER_TH | 0FMR_TH | FMR1000_TH | FMR100_TH | FMR20_TH | FMR10_TH | 0FNMR_TH | |
| NBIS | 1.000 | 5.000 | 48.000 | 23.000 | 16.000 | 11.000 | 9.000 | 0.000 | |
| MCC | 1.000 | 0.016 | 0.286 | 0.025 | 0.021 | 0.018 | 0.017 | 0.000 | |
| VeriFinger | 1.000 | 10.000 | 194.000 | 39.000 | 27.000 | 19.000 | 15.000 | 0.000 | |
| MinutiaeNet-MCC | 1.000 | 0.011 | 0.047 | 0.023 | 0.017 | 0.015 | 0.014 | -1.000 | |
| MinutiaeNet-NBIS | 1.000 | 3.000 | 16.000 | 7.000 | 5.000 | 4.000 | 3.000 | 0.000 | |
| MSU-LAFIS | 1.000 | 2.310 | 494.986 | 38.390 | 24.308 | 14.037 | 9.843 | -1.000 | |

*Note: **GMean:** Genuine scores distribution mean; **GSTD:** Genuine scores distribution standard deviation; **IMean:** Impostor scores distribution mean; **ISTD:** Impostor scores distribution standard deviation; **AUC:** Area under the ROC curve; **SI:** Sensitivity Index; **JI:** Youden's J Index; **TH:** THreshold; **MCC:** Matthews Correlation Coefficient; **EER:** Equal Error Rate; **EERL:** EER low; **EERH:** EER high.*

### *B. Supplementary results for the NBIS comparison experiments*

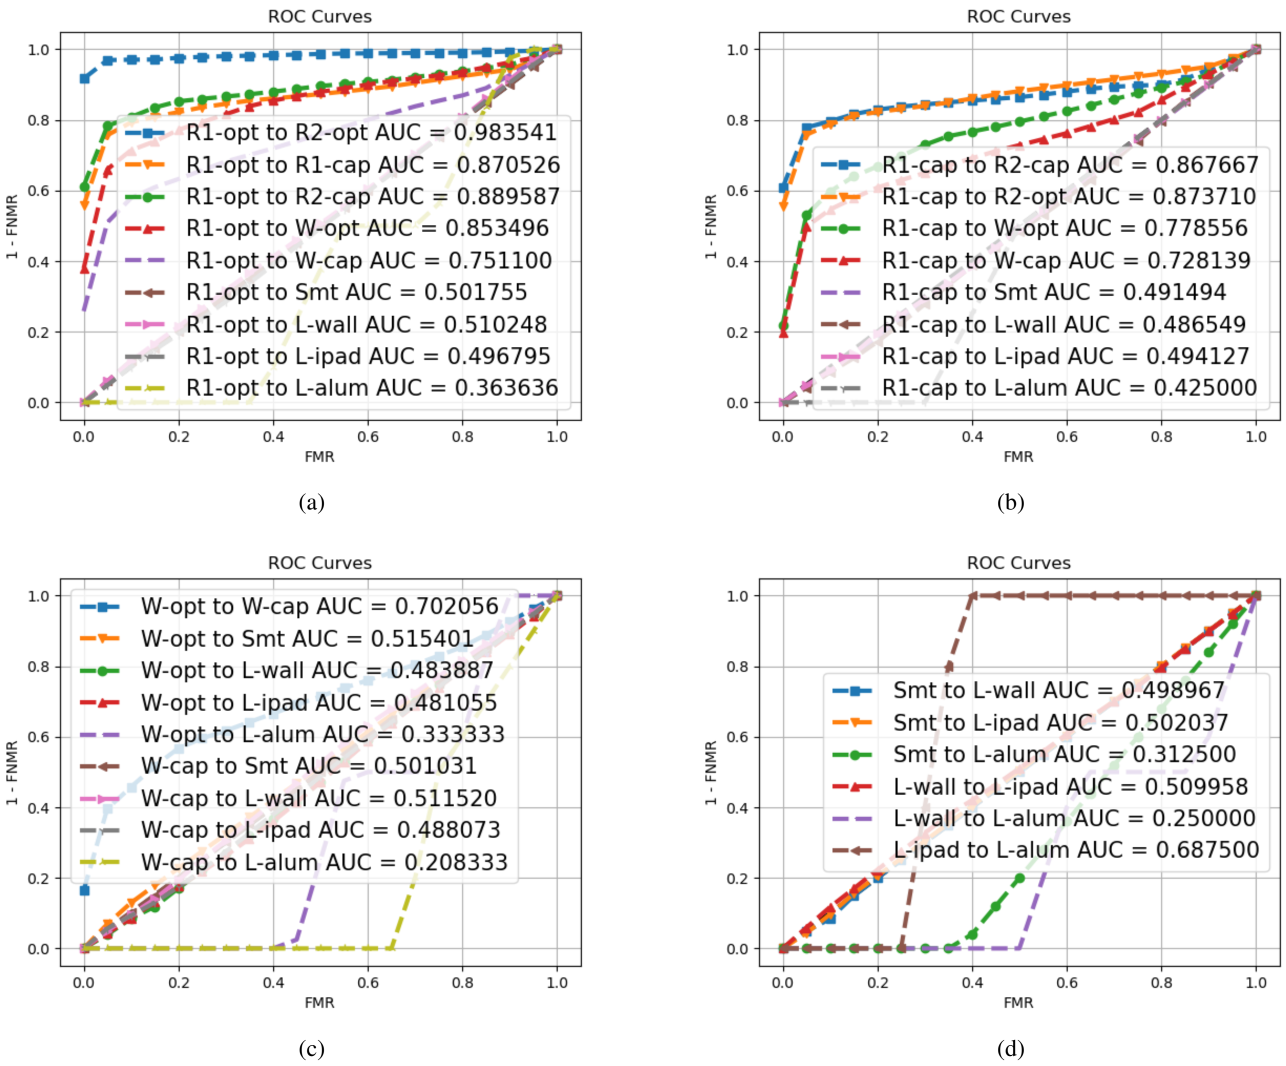


Fig. 16: ROC curve of the NBIS comparison experiments for the 'Latent in the Wild' database

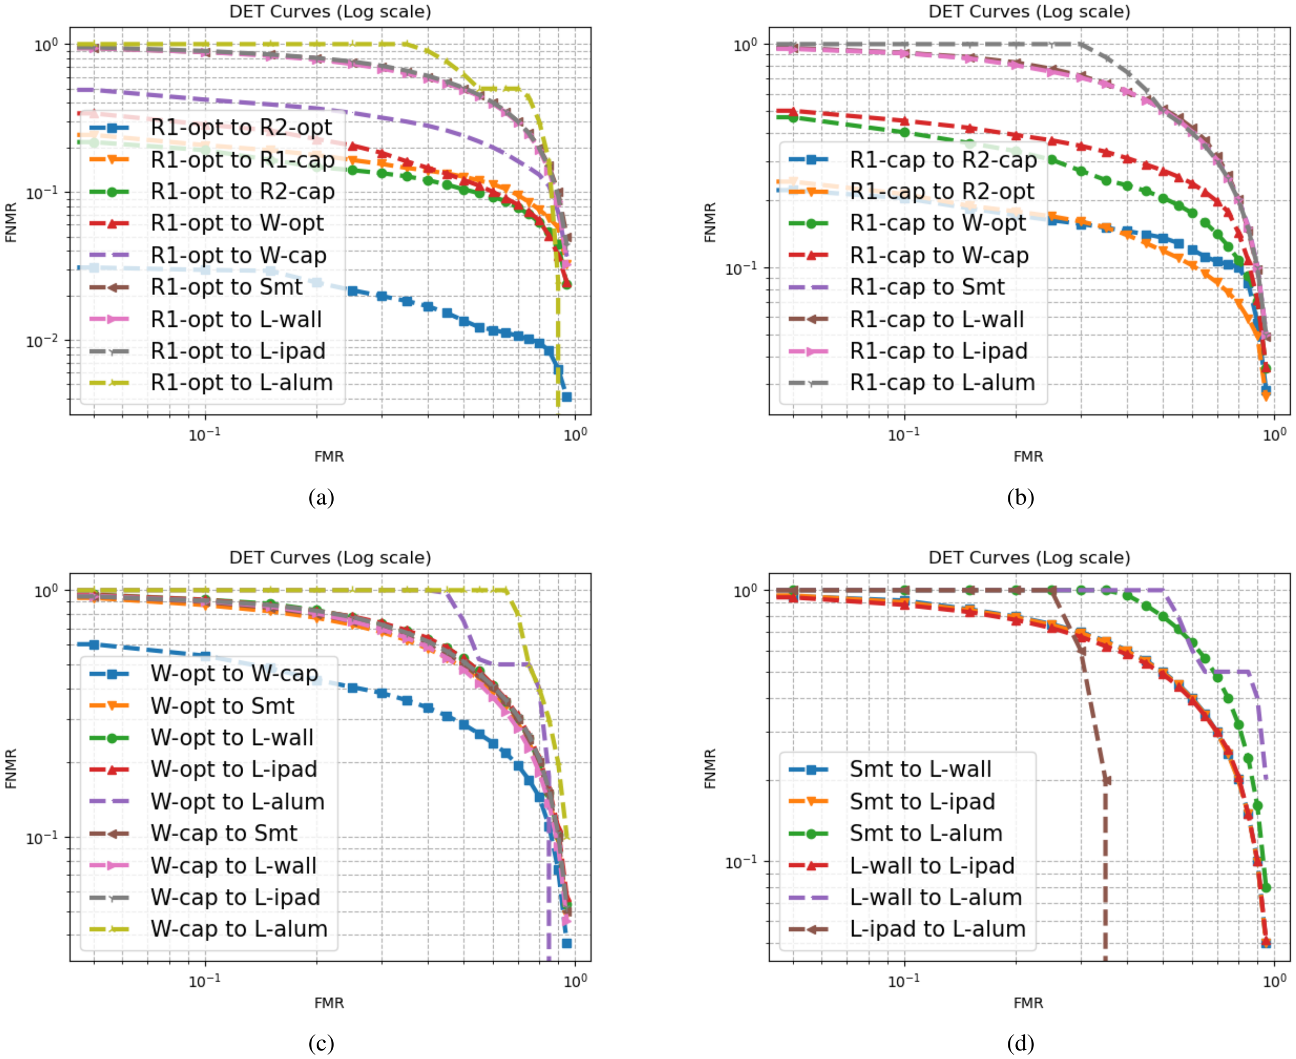


Fig. 17: DET curve of the NBIS comparison experiments for the 'Latent in the Wild' database

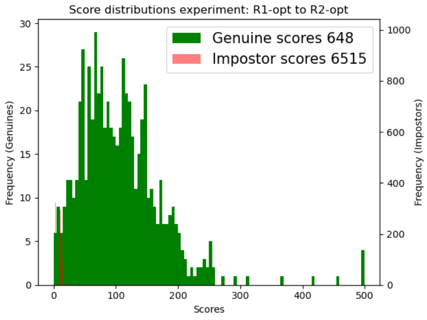


(a) R1-opt to R2-opt

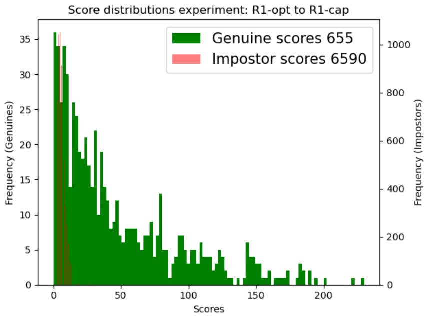


(b) R1-opt to R1-cap

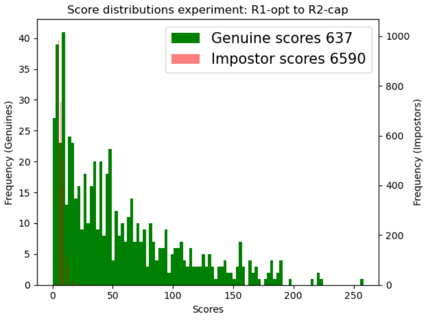


(c) R1-opt to R2-cap

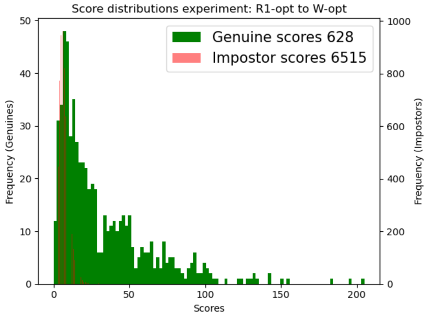


(d) R1-opt to W-opt

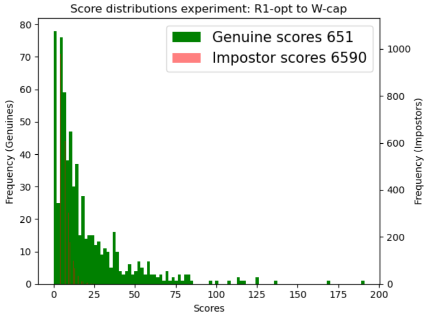


(e) R1-opt to W-cap

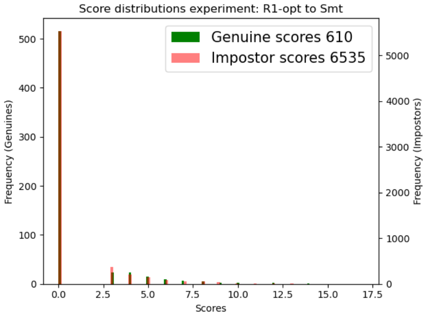


(f) R1-opt to Smt

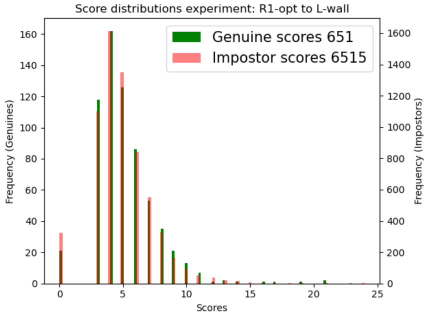


(g) R1-opt to L-wall

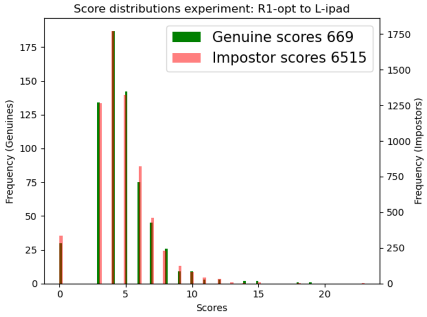


(h) R1-opt to L-ipad

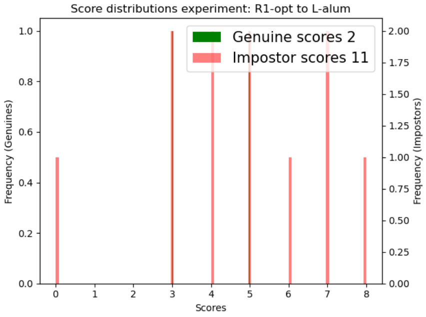


(i) R1-opt to L-alum

Fig. 18: Distributions of the NBIS (part 1/4) comparison scores in the 'Latent in the Wild' database

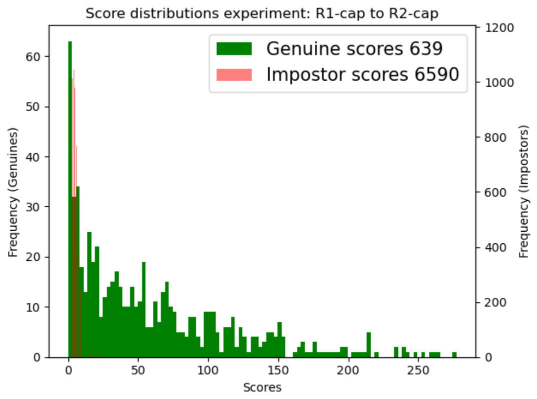


(a) R1-cap to R2-cap

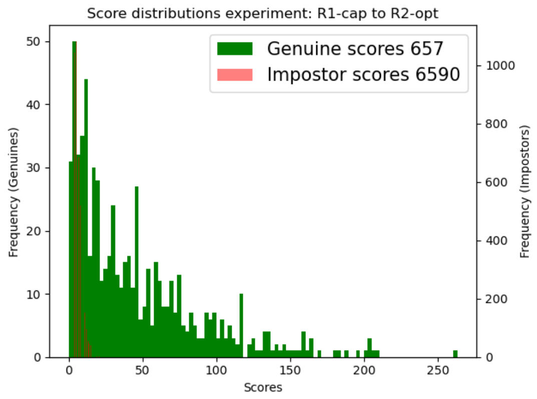


(b) R1-cap to R2-opt

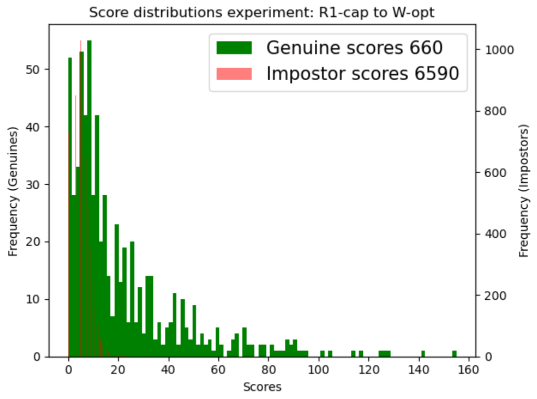


(c) R1-cap to W-opt

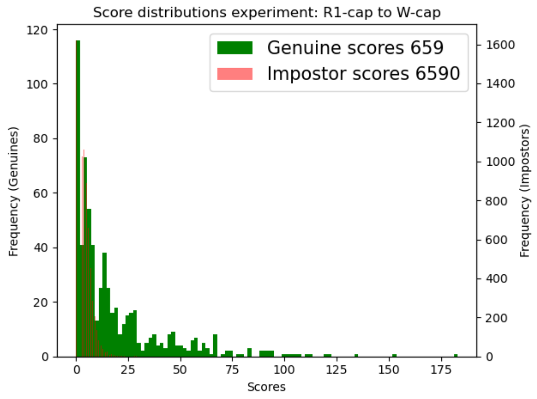


(d) R1-cap to W-cap

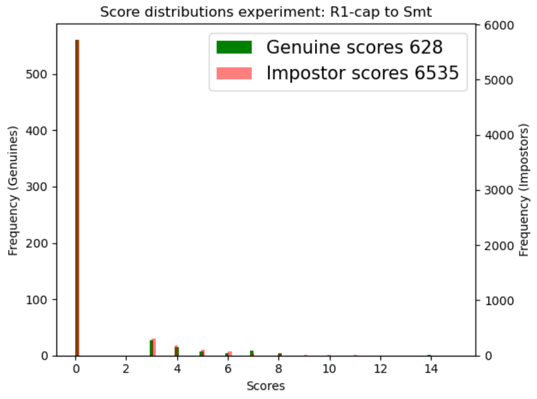


(e) R1-cap to Smt

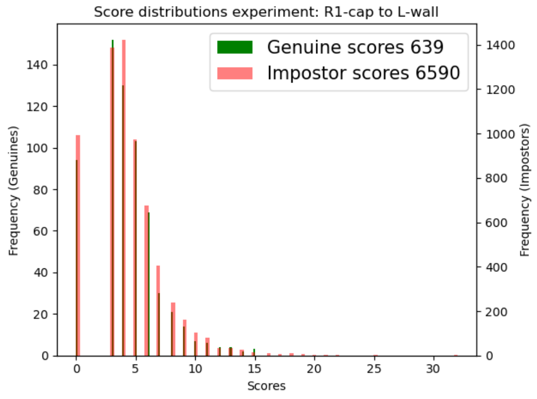


(f) R1-cap to L-wall

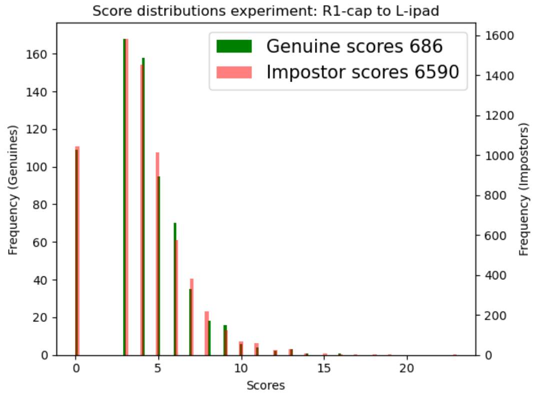


(g) R1-cap to L-ipad

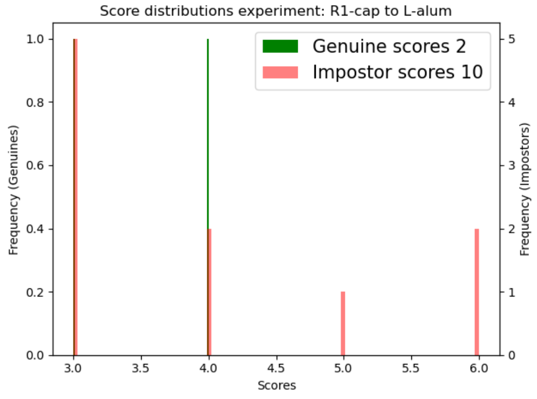


(h) R1-cap to L-alum

Fig. 19: Distributions of the NBIS (part 2/4) comparison scores in the 'Latent in the Wild' database

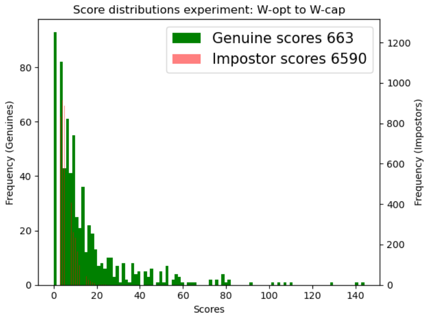


(a) W-opt to W-cap

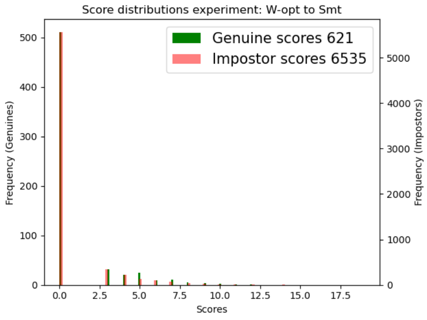


(b) W-opt to Smt

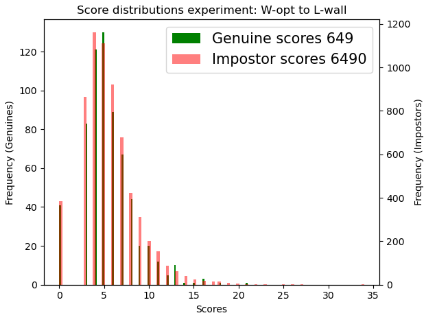


(c) W-opt to L-wall

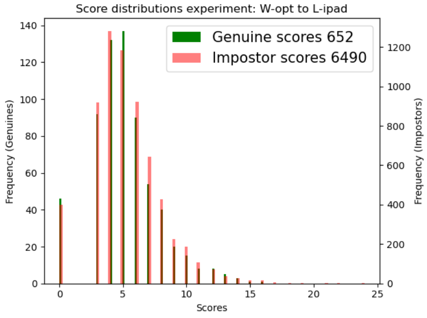


(d) W-opt to L-ipad

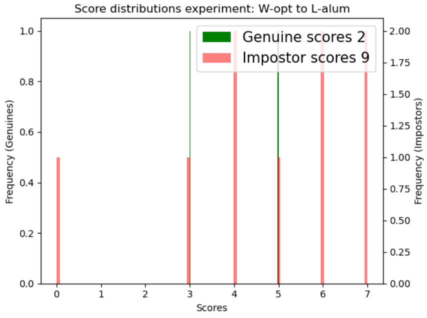


(e) W-opt to L-alum

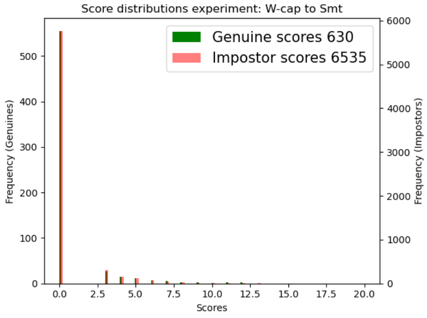


(f) W-cap to Smt

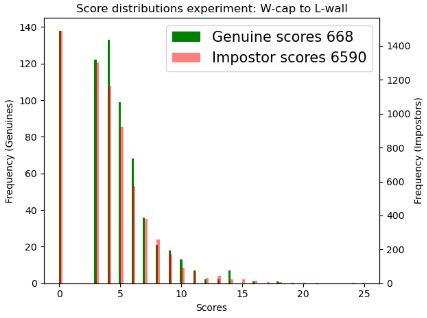


(g) W-cap to L-wall

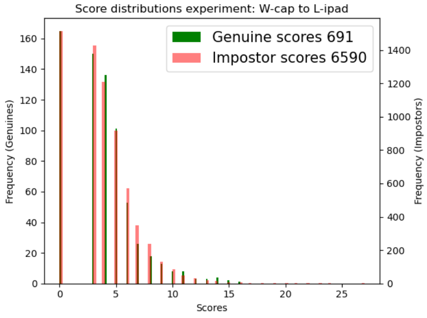


(h) W-cap to L-ipad

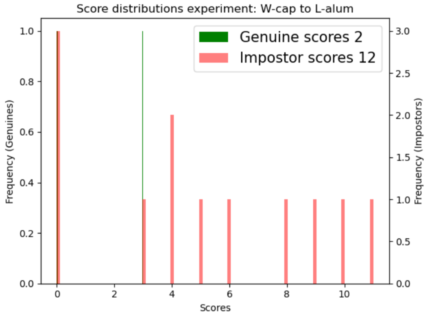


(i) W-cap to L-alum

Fig. 20: Distributions of the NBIS (part 3/4) comparison scores in the 'Latent in the Wild' database

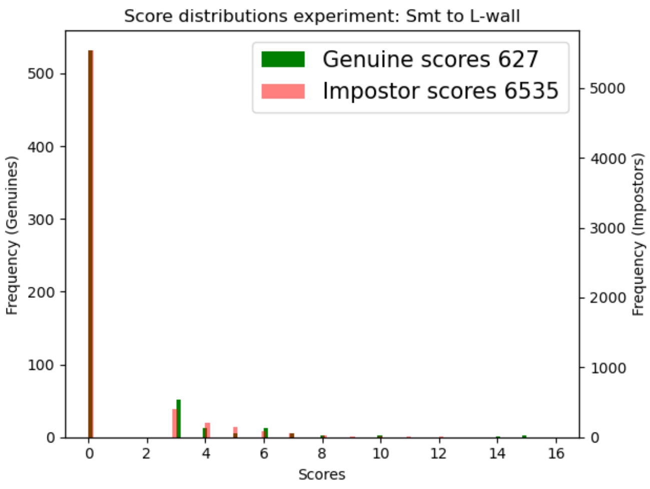


(a) Smt to L-wall

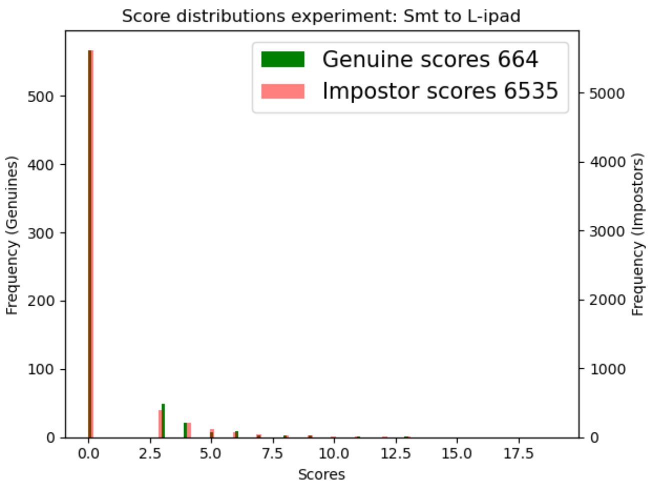


(b) Smt to L-ipad

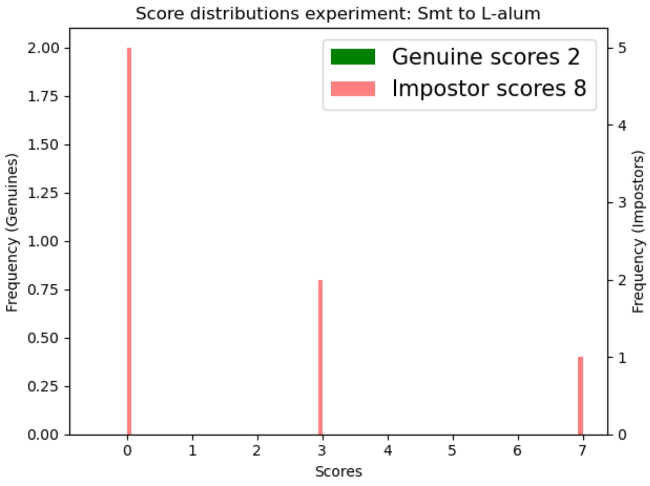


(c) Smt to L-alum

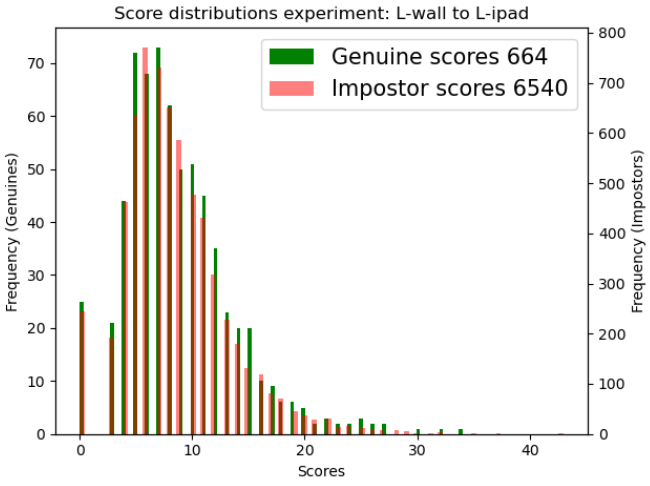


(d) L-wall to L-ipad

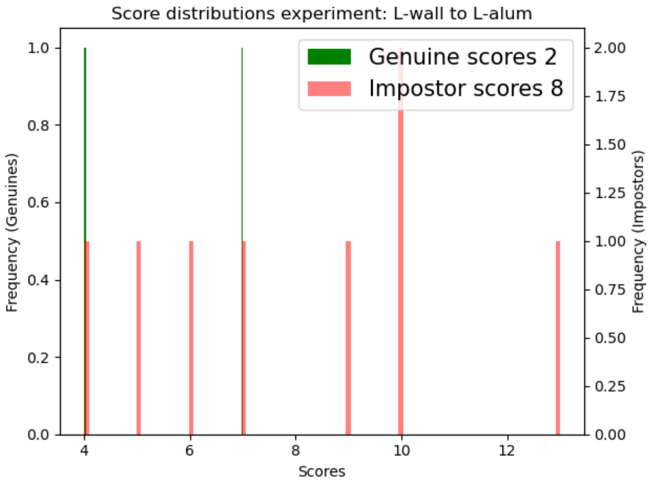


(e) L-wall to L-alum

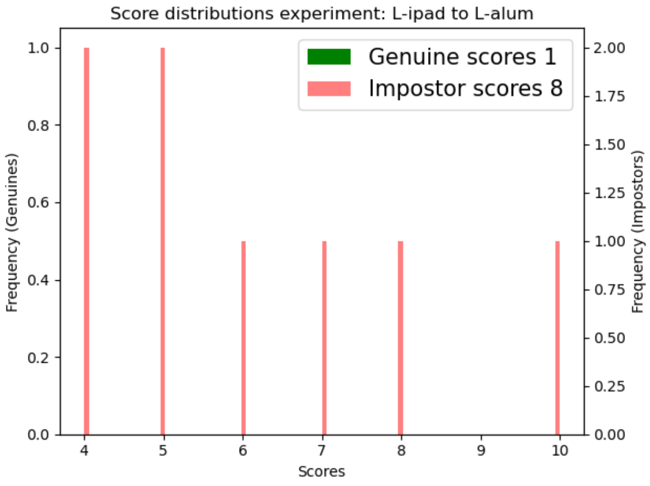


(f) L-ipad to L-alum

Fig. 21: Distributions of the NBIS (part 4/4) comparison scores in the 'Latent in the Wild' database

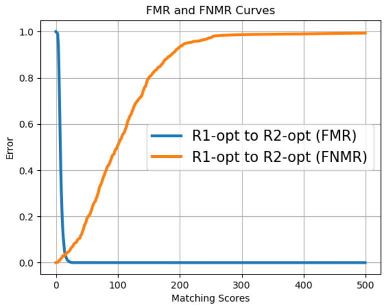


(a) R1-opt to R2-opt

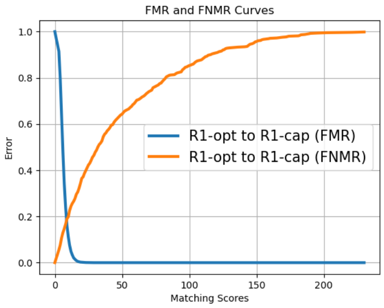


(b) R1-opt to R1-cap

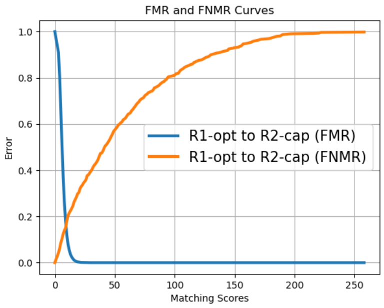


(c) R1-opt to R2-cap

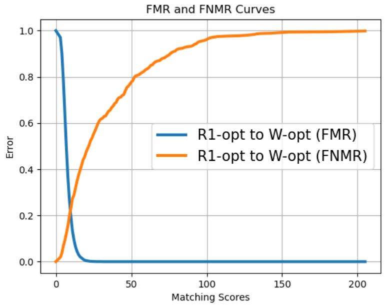


(d) R1-opt to W-opt

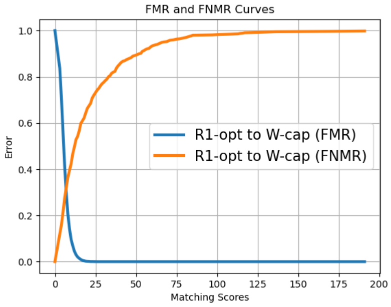


(e) R1-opt to W-cap

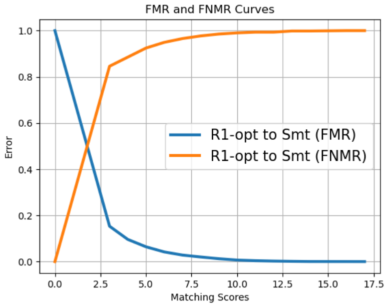


(f) R1-opt to Smt

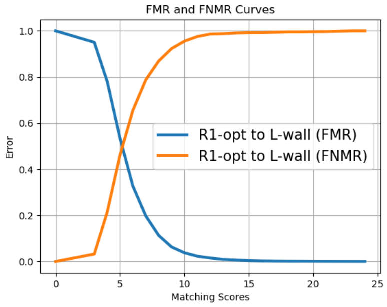


(g) R1-opt to L-wall

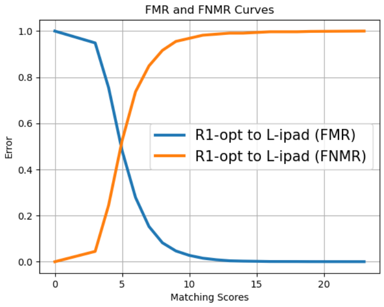


(h) R1-opt to L-ipad

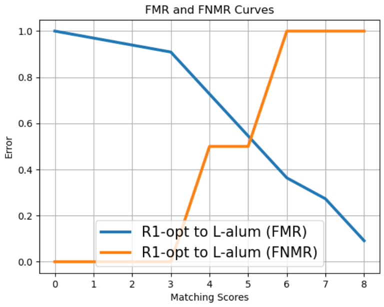


(i) R1-opt to L-alum

Fig. 22: FMR and FNMR curves of the NBIS (part 1/4) comparison scores in the 'Latent in the Wild' database

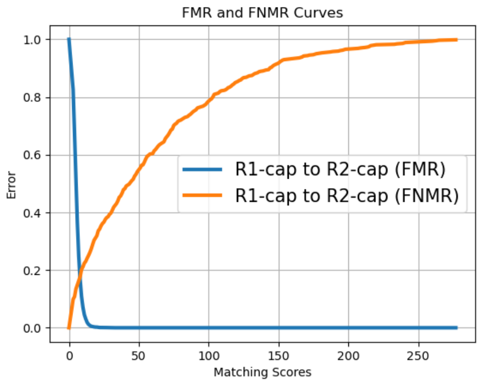


(a) R1-cap to R2-cap

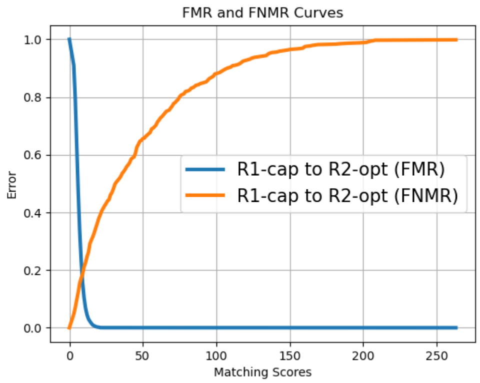


(b) R1-cap to R2-opt

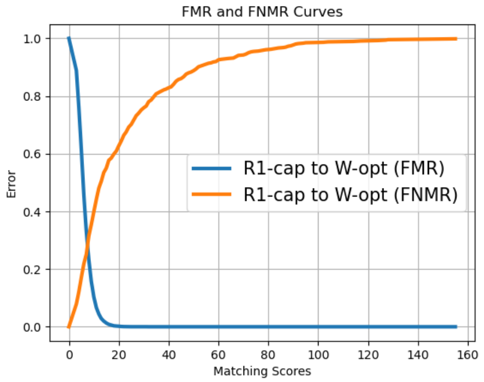


(c) R1-cap to W-opt

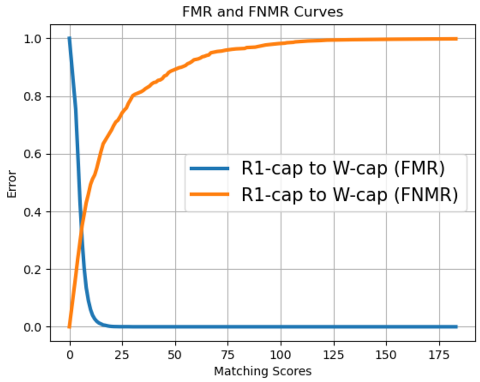


(d) R1-cap to W-cap

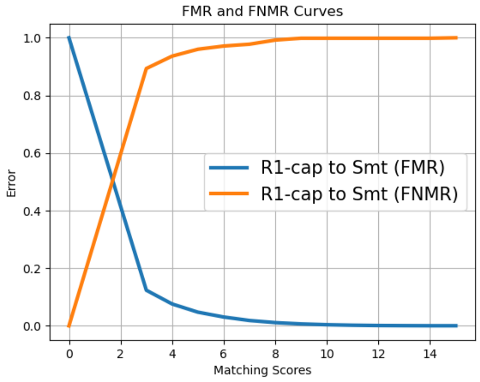


(e) R1-cap to Smt

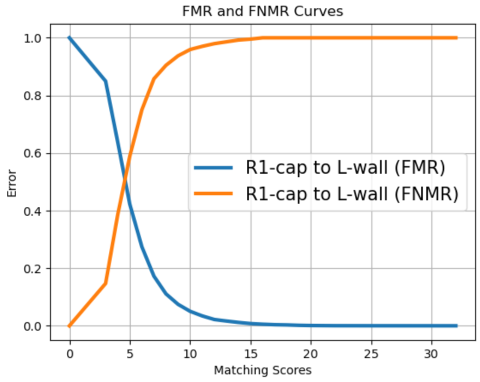


(f) R1-cap to L-wall

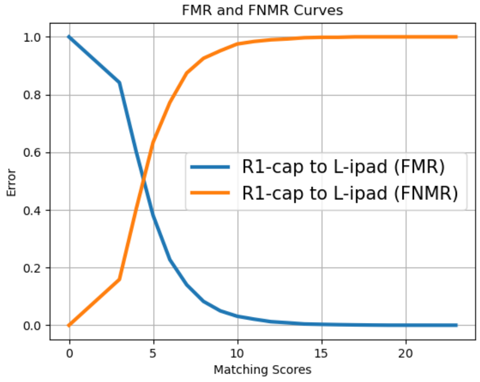


(g) R1-cap to L-ipad

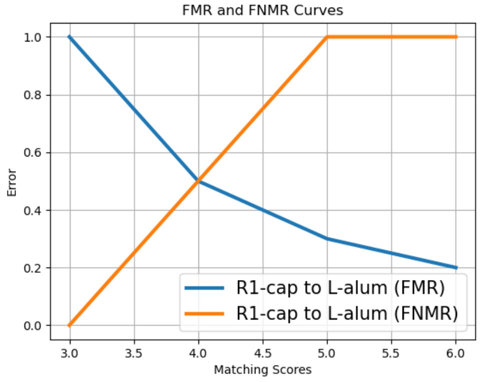


(h) R1-cap to L-alum

Fig. 23: FMR and FNMR curves of the NBIS (part 2/4) comparison scores in the 'Latent in the Wild' database

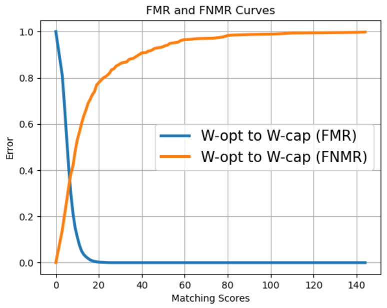


(a) W-opt to W-cap

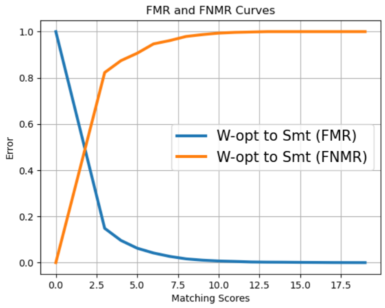


(b) W-opt to Smt

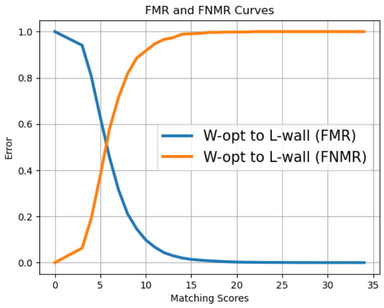


(c) W-opt to L-wall

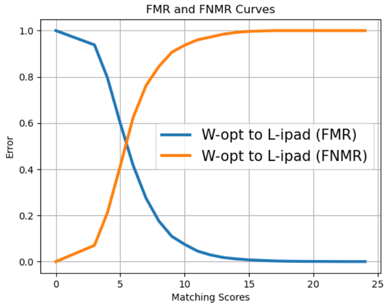


(d) W-opt to L-ipad

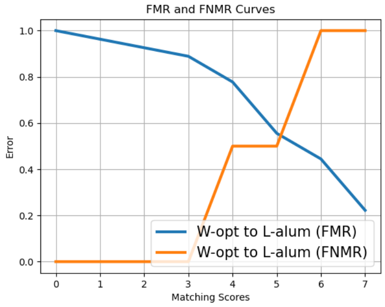


(e) W-opt to L-alum

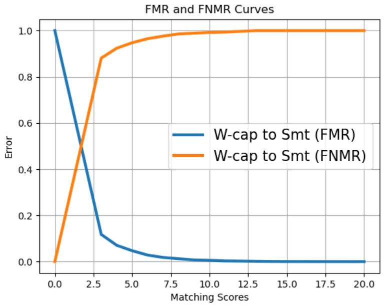


(f) W-cap to Smt

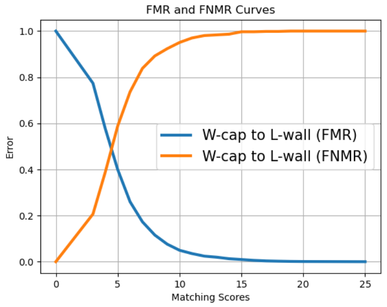


(g) W-cap to L-wall

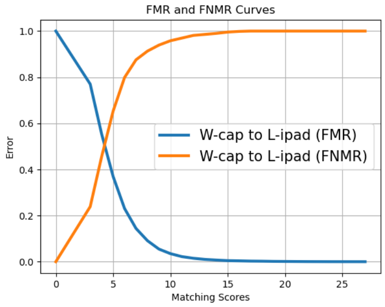


(h) W-cap to L-ipad

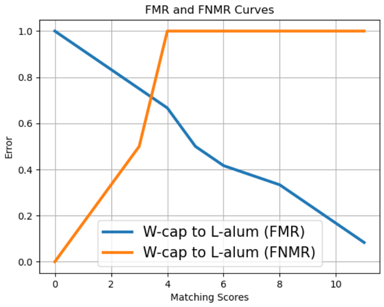


(i) W-cap to L-alum

Fig. 24: FMR and FNMR curves of the NBIS (part 3/4) comparison scores in the 'Latent in the Wild' database

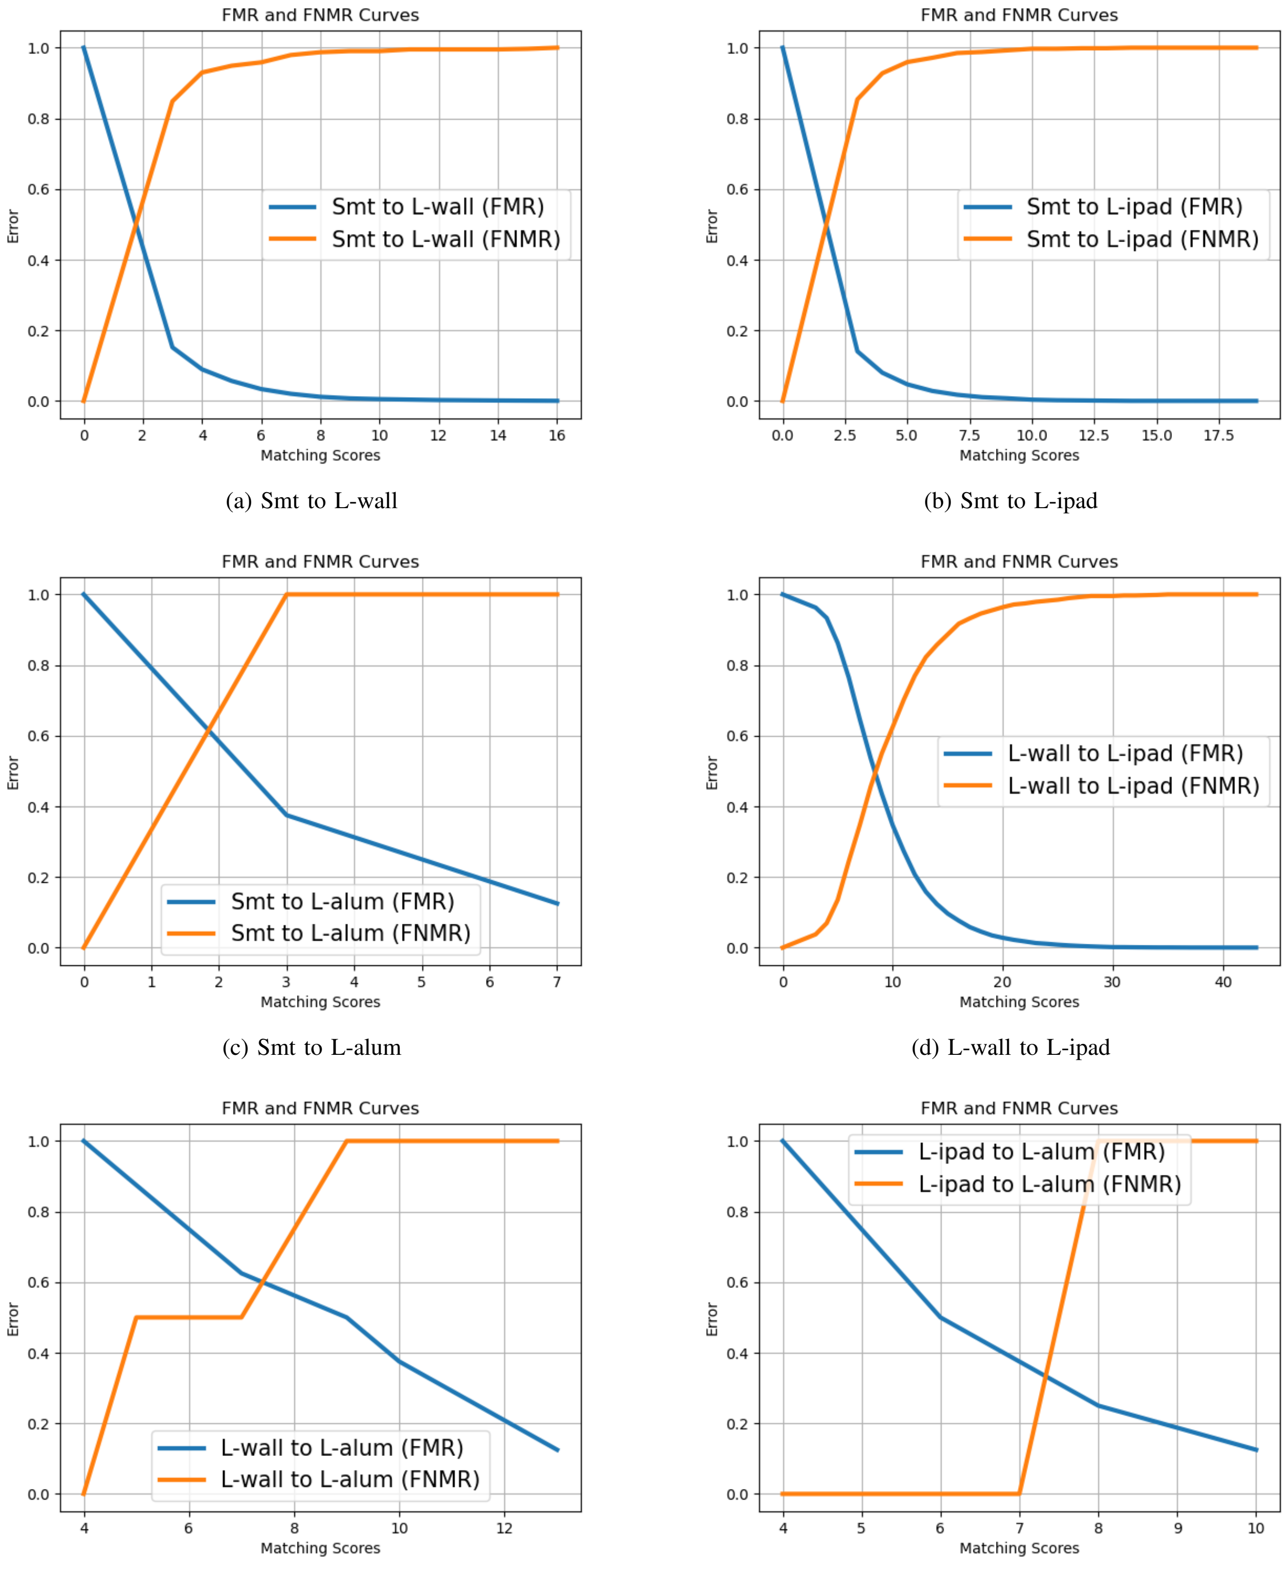


(a) Smt to L-wall

(b) Smt to L-ipad

(c) Smt to L-alum

(d) L-wall to L-ipad

(e) L-wall to L-alum

(f) L-ipad to L-alum

Fig. 25: FMR and FNMR curves of the NBIS (part 4/4) comparison scores in the 'Latent in the Wild' database

TABLE XIII: Performance indicators measured on the 'Latent in the Wild' database for the NBIS (part 1/4) comparison experiments.

| Comparison | GMean | GSTD | IMean | ISTD | SI | AUC | JI | JI_TH | MCC |
|---|---|---|---|---|---|---|---|---|---|
| R1-opt to R2-opt | 106.681 | 67.842 | 7.388 | 3.351 | 2.067 | 0.984 | 0.946 | 20.000 | 0.959 |
| R1-opt to R1-cap | 47.493 | 45.860 | 5.739 | 3.208 | 1.284 | 0.871 | 0.714 | 14.000 | 0.787 |
| R1-opt to R2-cap | 55.138 | 49.903 | 5.865 | 3.322 | 1.393 | 0.890 | 0.741 | 14.000 | 0.807 |
| R1-opt to W-opt | 32.441 | 31.046 | 6.995 | 3.396 | 1.152 | 0.853 | 0.618 | 13.000 | 0.676 |
| R1-opt to W-cap | 20.078 | 23.744 | 5.139 | 3.452 | 0.881 | 0.751 | 0.480 | 10.000 | 0.564 |
| R1-opt to Smt | 0.802 | 2.095 | 0.741 | 1.949 | 0.030 | 0.502 | 0.019 | 4.000 | 0.022 |
| R1-opt to L-wall | 5.132 | 2.449 | 4.970 | 2.333 | 0.068 | 0.510 | 0.018 | 8.000 | 0.028 |
| R1-opt to L-ipad | 4.735 | 2.210 | 4.706 | 2.121 | 0.013 | 0.497 | 0.007 | 3.000 | 0.033 |
| R1-opt to L-alum | 4.000 | 1.000 | 4.727 | 2.178 | 0.429 | 0.364 | 0.091 | 3.000 | 0.123 |
| | | | | | | | | | |
| Comparison | MCC_TH | EERL | EERH | EER | 0FMR | FMR1000 | FMR100 | FMR20 | FMR10 |
| R1-opt to R2-opt | 25.000 | 0.026 | 0.040 | 0.033 | 0.083 | 0.065 | 0.045 | 0.031 | 0.029 |
| R1-opt to R1-cap | 18.000 | 0.162 | 0.189 | 0.176 | 0.443 | 0.386 | 0.296 | 0.244 | 0.198 |
| R1-opt to R2-cap | 20.000 | 0.119 | 0.181 | 0.150 | 0.388 | 0.330 | 0.262 | 0.215 | 0.181 |
| R1-opt to W-opt | 20.000 | 0.194 | 0.231 | 0.212 | 0.621 | 0.535 | 0.439 | 0.347 | 0.288 |
| R1-opt to W-cap | 18.000 | 0.297 | 0.320 | 0.308 | 0.742 | 0.674 | 0.599 | 0.496 | 0.424 |
| R1-opt to Smt | 12.000 | 0.153 | 0.846 | 0.500 | 1.000 | 0.998 | 0.985 | 0.949 | 0.885 |
| R1-opt to L-wall | 16.000 | 0.327 | 0.656 | 0.491 | 1.000 | 0.995 | 0.988 | 0.955 | 0.869 |
| R1-opt to L-ipad | 14.000 | 0.245 | 0.754 | 0.500 | 1.000 | 0.997 | 0.987 | 0.955 | 0.916 |
| R1-opt to L-alum | 3.000 | 0.500 | 0.545 | 0.523 | 1.000 | 1.000 | 1.000 | 1.000 | 1.000 |
| | | | | | | | | | |
| Comparison | 0FNMR | EER_TH | 0FMR_TH | FMR1000_TH | FMR100_TH | FMR20_TH | FMR10_TH | 0FNMR_TH | |
| R1-opt to R2-opt | 1.000 | 16.000 | 30.000 | 25.000 | 19.000 | 14.000 | 12.000 | 0.000 | |
| R1-opt to R1-cap | 1.000 | 9.000 | 27.000 | 22.000 | 16.000 | 12.000 | 10.000 | 0.000 | |
| R1-opt to R2-cap | 1.000 | 10.000 | 29.000 | 22.000 | 16.000 | 12.000 | 10.000 | 0.000 | |
| R1-opt to W-opt | 1.000 | 10.000 | 31.000 | 24.000 | 18.000 | 14.000 | 12.000 | 0.000 | |
| R1-opt to W-cap | 1.000 | 7.000 | 26.000 | 21.000 | 16.000 | 12.000 | 10.000 | 0.000 | |
| R1-opt to Smt | 1.000 | 3.000 | 17.000 | 13.000 | 9.000 | 6.000 | 4.000 | 0.000 | |
| R1-opt to L-wall | 1.000 | 6.000 | 24.000 | 19.000 | 13.000 | 10.000 | 8.000 | 0.000 | |
| R1-opt to L-ipad | 1.000 | 4.000 | 23.000 | 16.000 | 12.000 | 9.000 | 8.000 | 0.000 | |
| R1-opt to L-alum | 0.909 | 5.000 | 8.000 | 8.000 | 8.000 | 8.000 | 8.000 | 3.000 | |

*Note: **GMean:** Genuine scores distribution mean; **GSTD:** Genuine scores distribution standard deviation; **IMean:** Impostor scores distribution mean; **ISTD:** Impostor scores distribution standard deviation; **AUC:** Area under the ROC curve; **SI:** Sensitivity Index; **JI:** Youden's J Index; **TH:** THreshold; **MCC:** Matthews Correlation Coefficient; **EER:** Equal Error Rate; **EERL:** EER low; **EERH:** EER high.*

TABLE XIV: Performance indicators measured on the 'Latent in the Wild' database for the NBIS (part 2/4) comparison experiments.

| Comparison | GMean | GSTD | IMean | ISTD | SI | AUC | JI | JI_TH | MCC |
|---|---|---|---|---|---|---|---|---|---|
| R1-cap to R2-cap | 58.953 | 57.403 | 4.761 | 3.256 | 1.333 | 0.868 | 0.740 | 13.000 | 0.808 |
| R1-cap to R2-opt | 45.151 | 43.782 | 5.674 | 3.192 | 1.272 | 0.874 | 0.708 | 12.000 | 0.768 |
| R1-cap to W-opt | 21.450 | 23.503 | 5.518 | 3.283 | 0.949 | 0.779 | 0.498 | 10.000 | 0.587 |
| R1-cap to W-cap | 19.086 | 24.309 | 4.220 | 3.333 | 0.857 | 0.728 | 0.449 | 9.000 | 0.537 |
| R1-cap to Smt | 0.492 | 1.567 | 0.570 | 1.668 | 0.048 | 0.491 | 0.004 | 7.000 | 0.018 |
| R1-cap to L-wall | 4.254 | 2.694 | 4.405 | 2.924 | 0.054 | 0.487 | 0.003 | 3.000 | 0.003 |
| R1-cap to L-ipad | 4.025 | 2.508 | 4.094 | 2.607 | 0.027 | 0.494 | 0.000 | 6.000 | 0.000 |
| R1-cap to L-alum | 3.500 | 0.500 | 4.000 | 1.183 | 0.550 | 0.425 | 0.000 | 3.000 | 0.000 |
| | | | | | | | | | |
| Comparison | MCC_TH | EERL | EERH | EER | 0FMR | FMR1000 | FMR100 | FMR20 | FMR10 |
| R1-cap to R2-cap | 16.000 | 0.166 | 0.177 | 0.171 | 0.393 | 0.343 | 0.250 | 0.224 | 0.202 |
| R1-cap to R2-opt | 19.000 | 0.156 | 0.186 | 0.171 | 0.444 | 0.391 | 0.317 | 0.247 | 0.212 |
| R1-cap to W-opt | 18.000 | 0.232 | 0.315 | 0.274 | 0.780 | 0.644 | 0.577 | 0.480 | 0.398 |
| R1-cap to W-cap | 18.000 | 0.303 | 0.349 | 0.326 | 0.801 | 0.683 | 0.608 | 0.493 | 0.460 |
| R1-cap to Smt | 14.000 | 0.000 | 1.000 | 0.500 | 0.998 | 0.998 | 0.992 | 0.960 | 0.893 |
| R1-cap to L-wall | 3.000 | 0.423 | 0.588 | 0.506 | 1.000 | 1.000 | 0.992 | 0.959 | 0.905 |
| R1-cap to L-ipad | 6.000 | 0.404 | 0.602 | 0.503 | 1.000 | 1.000 | 0.993 | 0.952 | 0.926 |
| R1-cap to L-alum | 3.000 | 0.500 | 0.500 | 0.500 | 1.000 | 1.000 | 1.000 | 1.000 | 1.000 |
| | | | | | | | | | |
| Comparison | 0FNMR | EER_TH | 0FMR_TH | FMR1000_TH | FMR100_TH | FMR20_TH | FMR10_TH | 0FNMR_TH | |
| R1-cap to R2-cap | 1.000 | 8.000 | 29.000 | 22.000 | 14.000 | 11.000 | 9.000 | 0.000 | |
| R1-cap to R2-opt | 1.000 | 9.000 | 27.000 | 21.000 | 16.000 | 12.000 | 10.000 | 0.000 | |
| R1-cap to W-opt | 1.000 | 8.000 | 32.000 | 21.000 | 16.000 | 12.000 | 10.000 | 0.000 | |
| R1-cap to W-cap | 1.000 | 6.000 | 30.000 | 20.000 | 15.000 | 10.000 | 9.000 | 0.000 | |
| R1-cap to Smt | 1.000 | 0.000 | 14.000 | 12.000 | 8.000 | 5.000 | 3.000 | 0.000 | |
| R1-cap to L-wall | 1.000 | 5.000 | 32.000 | 20.000 | 14.000 | 10.000 | 8.000 | 0.000 | |
| R1-cap to L-ipad | 1.000 | 4.000 | 23.000 | 18.000 | 13.000 | 9.000 | 8.000 | 0.000 | |
| R1-cap to L-alum | 1.000 | 4.000 | 6.000 | 6.000 | 6.000 | 6.000 | 6.000 | 3.000 | |

*Note: **GMean:** Genuine scores distribution mean; **GSTD:** Genuine scores distribution standard deviation; **IMean:** Impostor scores distribution mean; **ISTD:** Impostor scores distribution standard deviation; **AUC:** Area under the ROC curve; **SI:** Sensitivity Index; **JI:** Youden's J Index; **TH:** THreshold; **MCC:** Matthews Correlation Coefficient; **EER:** Equal Error Rate; **EERL:** EER low; **EERH:** EER high.*

TABLE XV: Performance indicators measured on the 'Latent in the Wild' database for the NBIS (part 3/4) comparison experiments.

| Comparison | GMean | GSTD | IMean | ISTD | SI | AUC | JI | JI_TH | MCC |
|---|---|---|---|---|---|---|---|---|---|
| W-opt to W-cap | 15.207 | 19.286 | 5.080 | 3.670 | 0.730 | 0.702 | 0.367 | 8.000 | 0.441 |
| W-opt to Smt | 0.887 | 2.091 | 0.722 | 1.949 | 0.082 | 0.515 | 0.031 | 5.000 | 0.035 |
| W-opt to L-wall | 5.479 | 2.827 | 5.699 | 3.074 | 0.074 | 0.484 | 0.001 | 4.000 | 0.001 |
| W-opt to L-ipad | 5.183 | 2.613 | 5.387 | 2.748 | 0.076 | 0.481 | 0.000 | 0.000 | 0.000 |
| W-opt to L-alum | 4.000 | 1.000 | 4.667 | 2.108 | 0.404 | 0.333 | 0.111 | 3.000 | 0.149 |
| W-cap to Smt | 0.587 | 1.785 | 0.554 | 1.698 | 0.019 | 0.501 | 0.006 | 6.000 | 0.015 |
| W-cap to L-wall | 4.150 | 2.981 | 4.090 | 3.149 | 0.020 | 0.512 | 0.034 | 4.000 | 0.020 |
| W-cap to L-ipad | 3.770 | 2.901 | 3.863 | 2.915 | 0.032 | 0.488 | 0.008 | 11.000 | 0.016 |
| W-cap to L-alum | 1.500 | 1.500 | 5.000 | 3.742 | 1.228 | 0.208 | 0.000 | 0.000 | 0.000 |
| | | | | | | | | | |
| Comparison | MCC_TH | EERL | EERH | EER | 0FMR | FMR1000 | FMR100 | FMR20 | FMR10 |
| W-opt to W-cap | 18.000 | 0.297 | 0.385 | 0.341 | 0.836 | 0.804 | 0.707 | 0.603 | 0.532 |
| W-opt to Smt | 5.000 | 0.149 | 0.823 | 0.486 | 1.000 | 1.000 | 0.987 | 0.947 | 0.874 |
| W-opt to L-wall | 4.000 | 0.378 | 0.629 | 0.503 | 1.000 | 1.000 | 0.992 | 0.966 | 0.917 |
| W-opt to L-ipad | 0.000 | 0.414 | 0.599 | 0.507 | 1.000 | 1.000 | 0.992 | 0.960 | 0.906 |
| W-opt to L-alum | 3.000 | 0.500 | 0.556 | 0.528 | 1.000 | 1.000 | 1.000 | 1.000 | 1.000 |
| W-cap to Smt | 11.000 | 0.118 | 0.881 | 0.499 | 1.000 | 1.000 | 0.989 | 0.948 | 0.881 |
| W-cap to L-wall | 4.000 | 0.389 | 0.576 | 0.483 | 1.000 | 1.000 | 0.997 | 0.951 | 0.892 |
| W-cap to L-ipad | 11.000 | 0.456 | 0.553 | 0.505 | 1.000 | 1.000 | 0.986 | 0.939 | 0.913 |
| W-cap to L-alum | 0.000 | 0.500 | 0.750 | 0.625 | 1.000 | 1.000 | 1.000 | 1.000 | 1.000 |
| | | | | | | | | | |
| Comparison | 0FNMR | EER_TH | 0FMR_TH | FMR1000_TH | FMR100_TH | FMR20_TH | FMR10_TH | 0FNMR_TH | |
| W-opt to W-cap | 1.000 | 7.000 | 26.000 | 23.000 | 16.000 | 12.000 | 10.000 | 0.000 | |
| W-opt to Smt | 1.000 | 3.000 | 19.000 | 16.000 | 9.000 | 6.000 | 4.000 | 0.000 | |
| W-opt to L-wall | 1.000 | 5.000 | 34.000 | 23.000 | 16.000 | 12.000 | 10.000 | 0.000 | |
| W-opt to L-ipad | 1.000 | 5.000 | 24.000 | 21.000 | 14.000 | 11.000 | 9.000 | 0.000 | |
| W-opt to L-alum | 0.889 | 5.000 | 7.000 | 7.000 | 7.000 | 7.000 | 7.000 | 3.000 | |
| W-cap to Smt | 1.000 | 3.000 | 20.000 | 14.000 | 9.000 | 5.000 | 3.000 | 0.000 | |
| W-cap to L-wall | 1.000 | 4.000 | 25.000 | 20.000 | 15.000 | 10.000 | 8.000 | 0.000 | |
| W-cap to L-ipad | 1.000 | 4.000 | 27.000 | 21.000 | 13.000 | 9.000 | 8.000 | 0.000 | |
| W-cap to L-alum | 1.000 | 3.000 | 11.000 | 11.000 | 11.000 | 11.000 | 11.000 | 0.000 | |

*Note:* ***GMean:*** *Genuine scores distribution mean;* ***GSTD:*** *Genuine scores distribution standard deviation;* ***IMean:*** *Impostor scores distribution mean;* ***ISTD:*** *Impostor scores distribution standard deviation;* ***AUC:*** *Area under the ROC curve;* ***SI:*** *Sensitivity Index;* ***JI:*** *Youden's J Index;* ***TH:*** *THreshold;* ***MCC:*** *Matthews Correlation Coefficient;* ***EER:*** *Equal Error Rate;* ***EERL:*** *EER low;* ***EERH:*** *EER high.*

TABLE XVI: Performance indicators measured on the 'Latent in the Wild' database for the NBIS (part 4/4) comparison experiments.

| Comparison | GMean | GSTD | IMean | ISTD | SI | AUC | JI | JI_TH | MCC |
|---|---|---|---|---|---|---|---|---|---|
| Smt to L-wall | 0.692 | 1.910 | 0.691 | 1.821 | 0.001 | 0.499 | 0.008 | 6.000 | 0.024 |
| Smt to L-ipad | 0.623 | 1.676 | 0.622 | 1.704 | 0.001 | 0.502 | 0.006 | 3.000 | 0.005 |
| Smt to L-alum | 0.000 | 0.000 | 1.625 | 2.395 | 0.960 | 0.313 | 0.000 | 0.000 | 0.000 |
| L-wall to L-ipad | 8.858 | 4.925 | 8.609 | 4.588 | 0.052 | 0.510 | 0.029 | 10.000 | 0.021 |
| L-wall to L-alum | 5.500 | 1.500 | 8.000 | 2.828 | 1.104 | 0.250 | 0.000 | 4.000 | 0.000 |
| L-ipad to L-alum | 7.000 | 0.000 | 6.125 | 1.965 | 0.630 | 0.688 | 0.625 | 7.000 | 0.395 |
| | | | | | | | | | |
| Comparison | MCC_TH | EERL | EERH | EER | 0FMR | FMR1000 | FMR100 | FMR20 | FMR10 |
| Smt to L-wall | 14.000 | 0.000 | 1.000 | 0.500 | 1.000 | 0.997 | 0.987 | 0.949 | 0.930 |
| Smt to L-ipad | 13.000 | 0.140 | 0.854 | 0.497 | 1.000 | 0.998 | 0.988 | 0.959 | 0.928 |
| Smt to L-alum | 0.000 | 0.000 | 1.000 | 0.500 | 1.000 | 1.000 | 1.000 | 1.000 | 1.000 |
| L-wall to L-ipad | 25.000 | 0.436 | 0.550 | 0.493 | 1.000 | 0.997 | 0.982 | 0.946 | 0.887 |
| L-wall to L-alum | 4.000 | 0.500 | 0.625 | 0.563 | 1.000 | 1.000 | 1.000 | 1.000 | 1.000 |
| L-ipad to L-alum | 7.000 | 0.000 | 0.375 | 0.188 | 1.000 | 1.000 | 1.000 | 1.000 | 1.000 |
| | | | | | | | | | |
| Comparison | 0FNMR | EER_TH | 0FMR_TH | FMR1000_TH | FMR100_TH | FMR20_TH | FMR10_TH | 0FNMR_TH | |
| Smt to L-wall | 1.000 | 0.000 | 16.000 | 15.000 | 8.000 | 5.000 | 4.000 | 0.000 | |
| Smt to L-ipad | 1.000 | 3.000 | 19.000 | 13.000 | 8.000 | 5.000 | 4.000 | 0.000 | |
| Smt to L-alum | 1.000 | 0.000 | 7.000 | 7.000 | 7.000 | 7.000 | 7.000 | 0.000 | |
| L-wall to L-ipad | 1.000 | 9.000 | 43.000 | 32.000 | 24.000 | 18.000 | 15.000 | 0.000 | |
| L-wall to L-alum | 1.000 | 7.000 | 13.000 | 13.000 | 13.000 | 13.000 | 13.000 | 4.000 | |
| L-ipad to L-alum | 0.375 | 7.000 | 10.000 | 10.000 | 10.000 | 10.000 | 10.000 | 7.000 | |

*Note: **GMean:** Genuine scores distribution mean; **GSTD:** Genuine scores distribution standard deviation; **IMean:** Impostor scores distribution mean; **ISTD:** Impostor scores distribution standard deviation; **AUC:** Area under the ROC curve; **SI:** Sensitivity Index; **JI:** Youden's J Index; **TH:** THreshold; **MCC:** Matthews Correlation Coefficient; **EER:** Equal Error Rate; **EERL:** EER low; **EERH:** EER high.*

### C. Supplementary results for the MCC comparison experiments

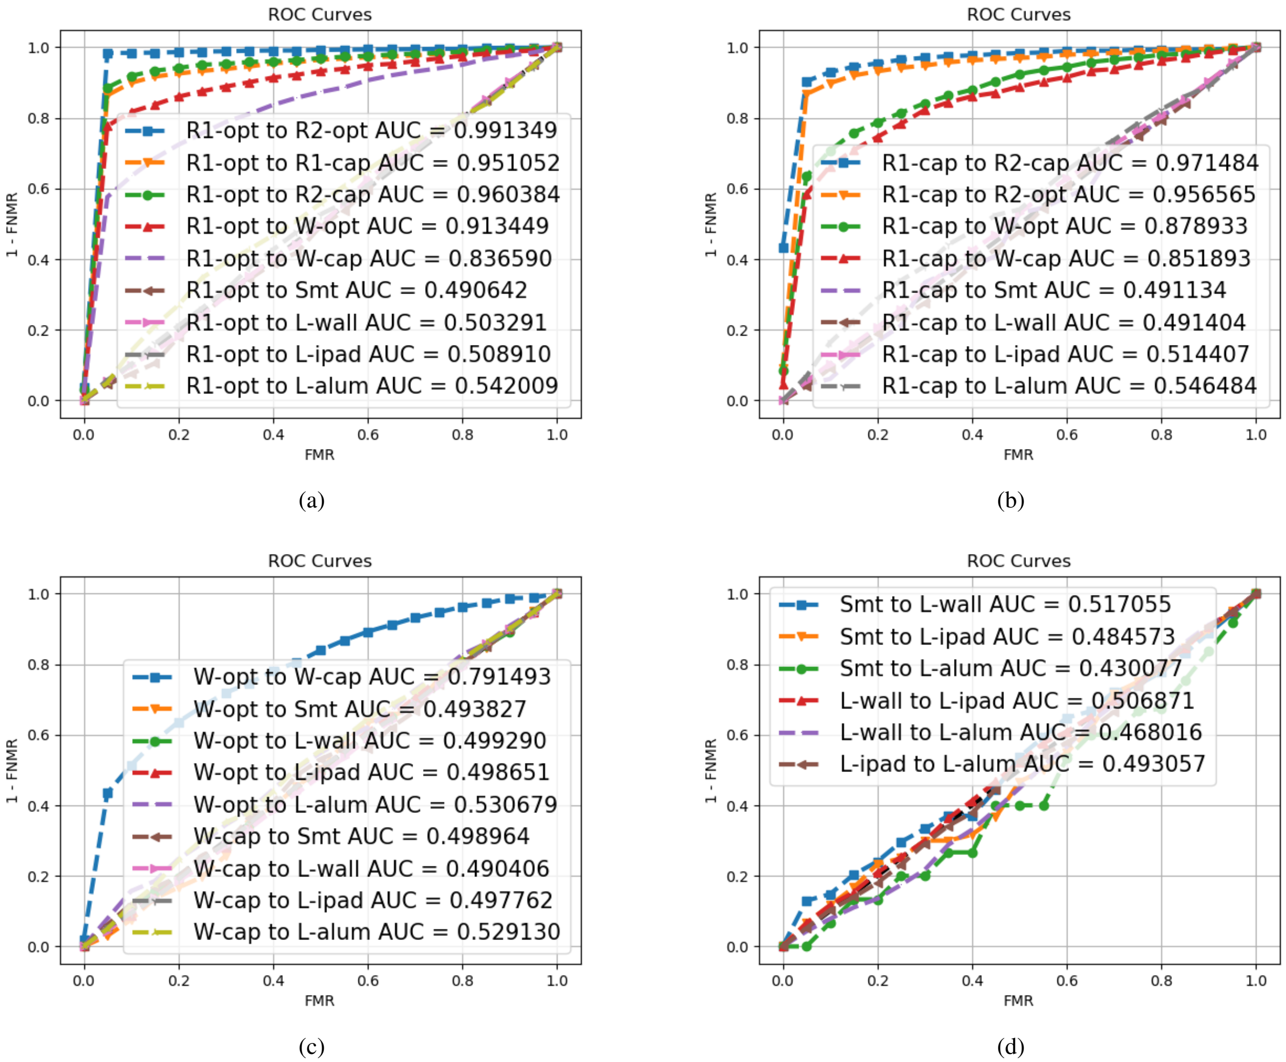


Fig. 26: ROC curve of the MCC comparison experiments for the 'Latent in the Wild' database

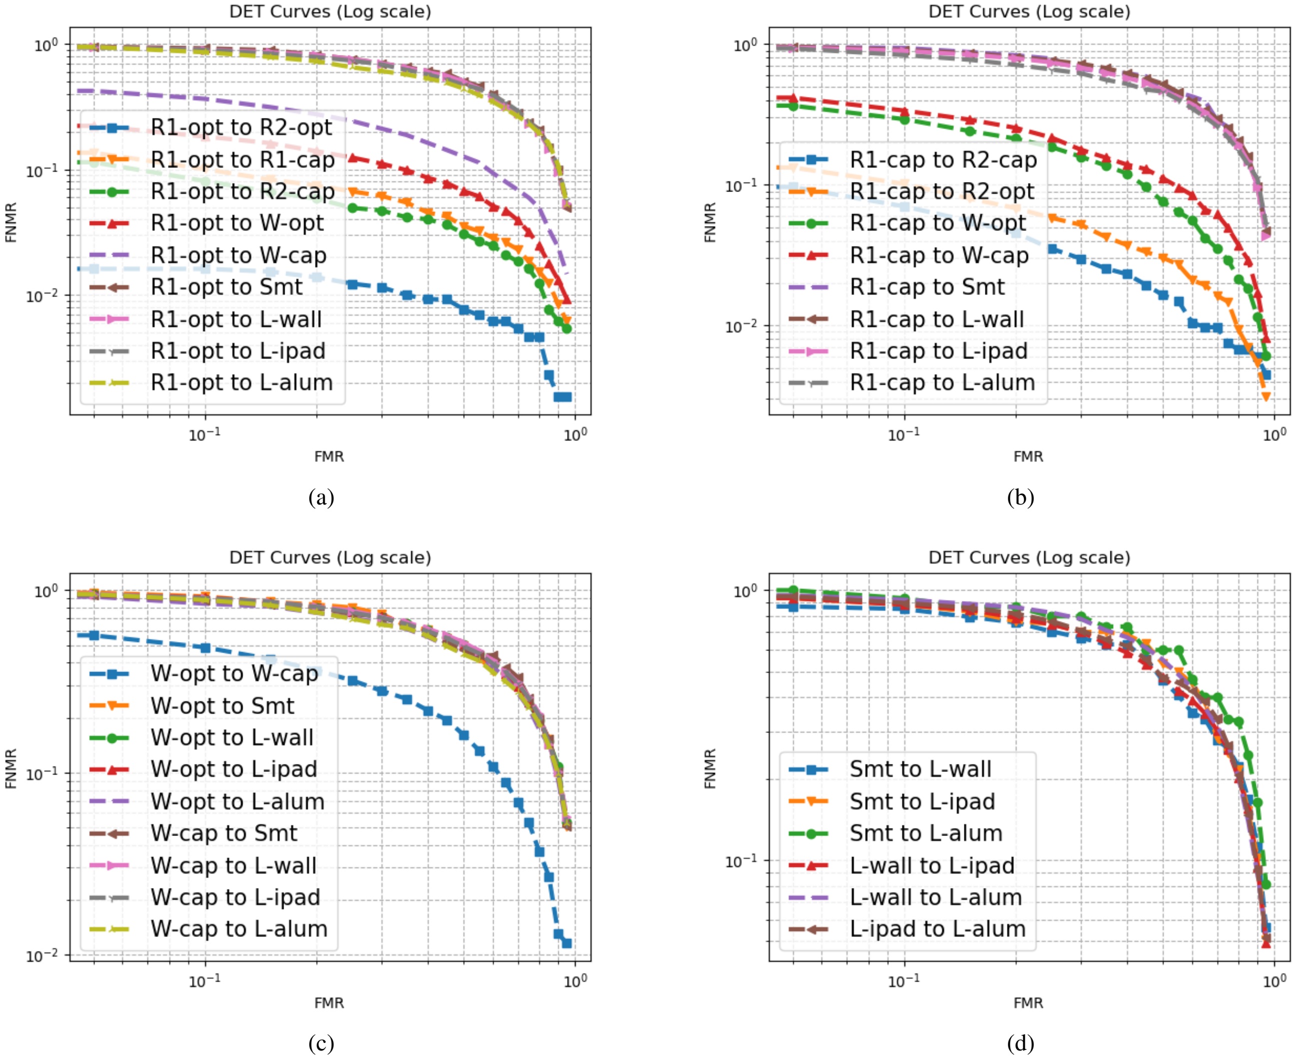


(a) (b) (c) (d)

Fig. 27: DET curve of the MCC comparison experiments for the 'Latent in the Wild' database

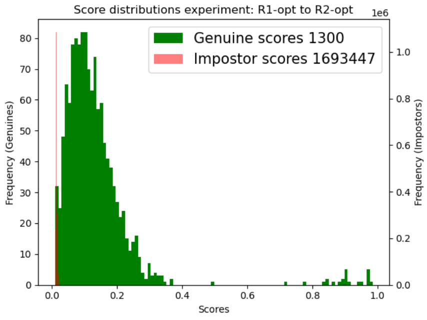


(a) R1-opt to R2-opt

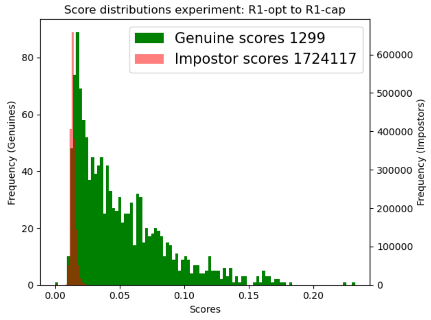


(b) R1-opt to R1-cap

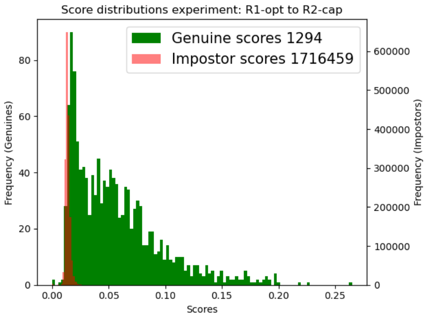


(c) R1-opt to R2-cap

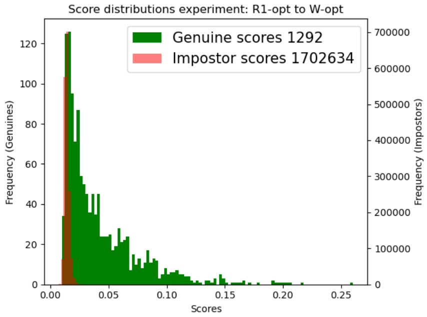


(d) R1-opt to W-opt

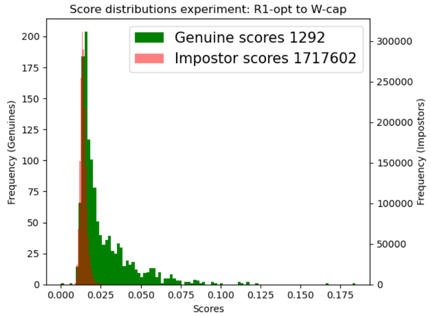


(e) R1-opt to W-cap

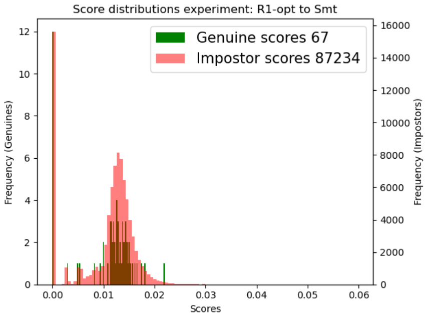


(f) R1-opt to Smt

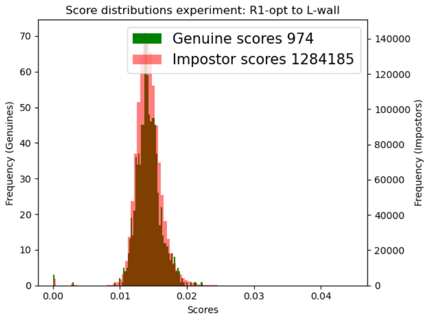


(g) R1-opt to L-wall

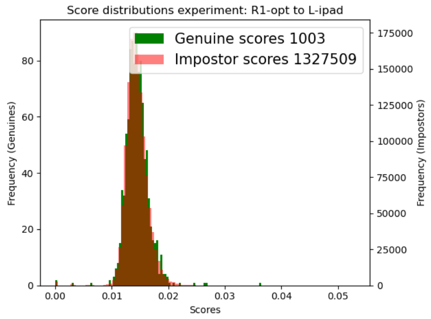


(h) R1-opt to L-ipad

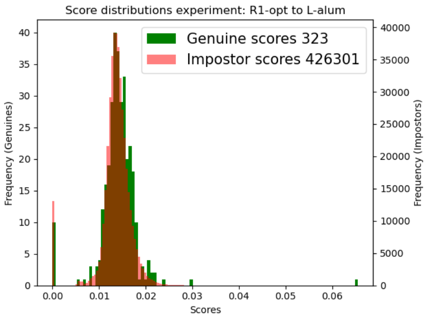


(i) R1-opt to L-alum

Fig. 28: Distributions of the MCC (part 1/4) comparison scores in the 'Latent in the Wild' database

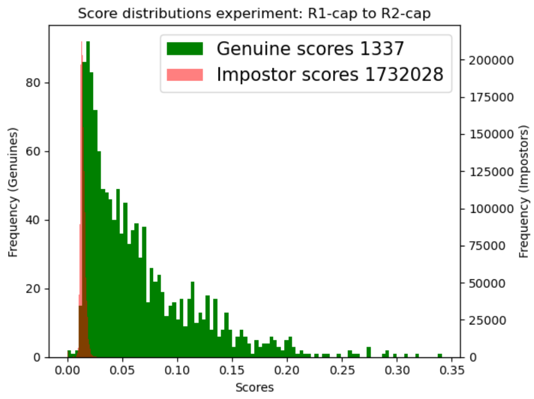


(a) R1-cap to R2-cap

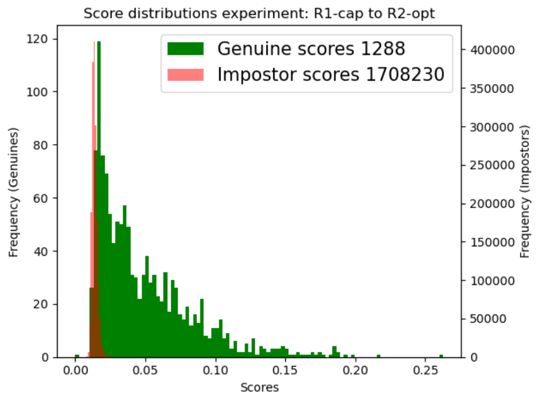


(b) R1-cap to R2-opt

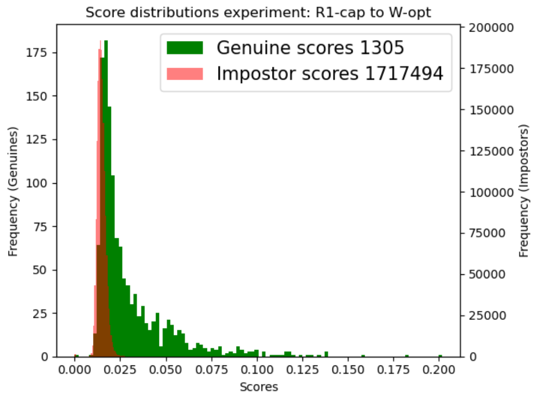


(c) R1-cap to W-opt

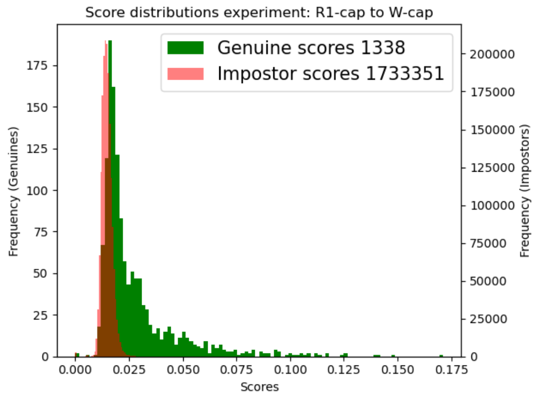


(d) R1-cap to W-cap

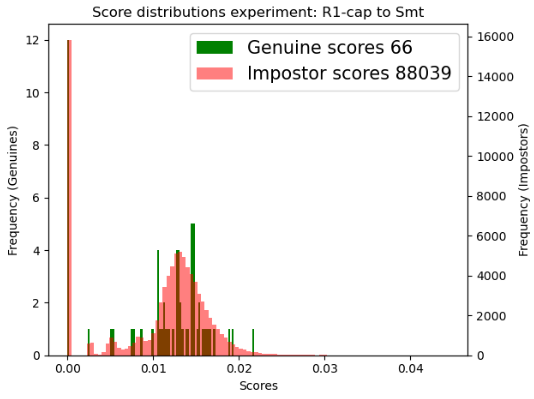


(e) R1-cap to Smt

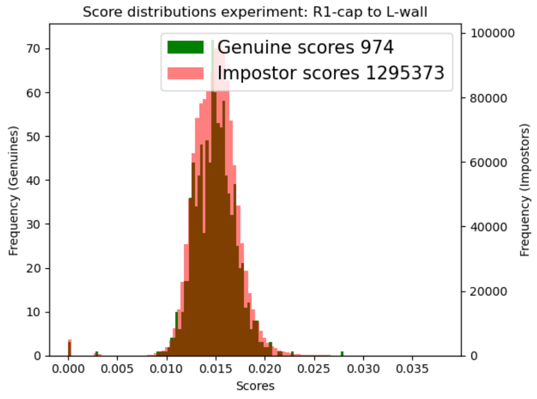


(f) R1-cap to L-wall

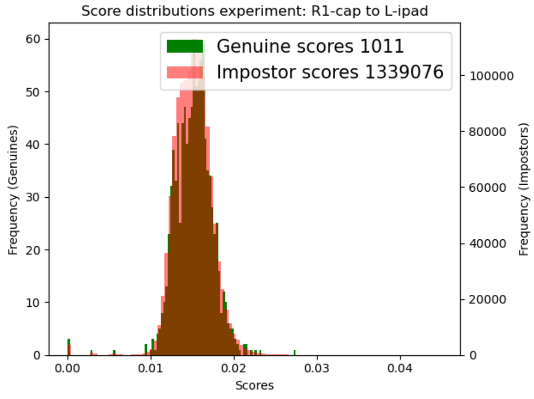


(g) R1-cap to L-ipad

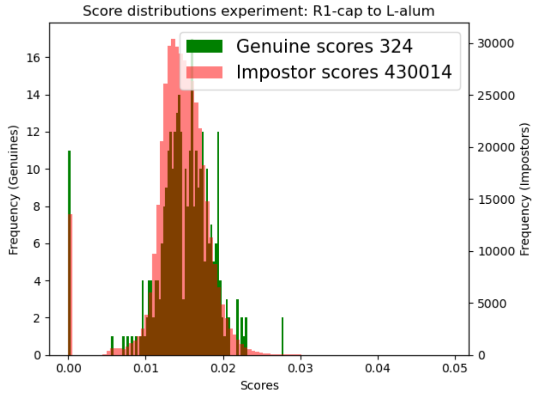


(h) R1-cap to L-alum

Fig. 29: Distributions of the MCC (part 2/4) comparison scores in the 'Latent in the Wild' database

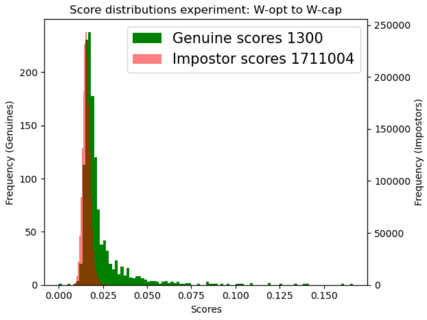


(a) W-opt to W-cap

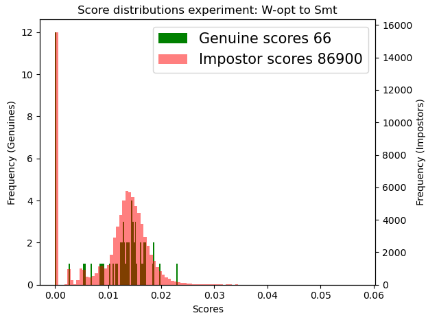


(b) W-opt to Smt

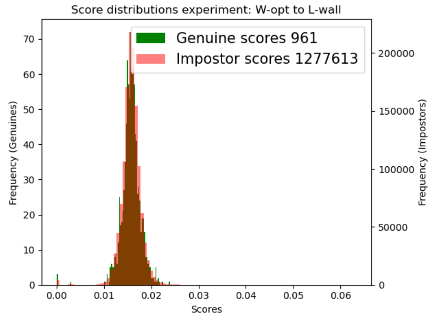


(c) W-opt to L-wall

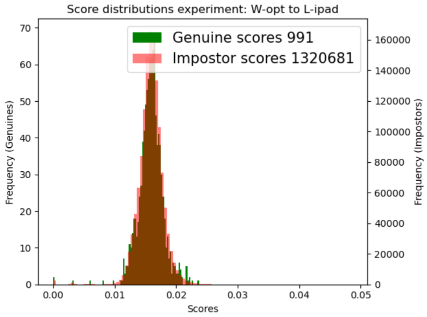


(d) W-opt to L-ipad

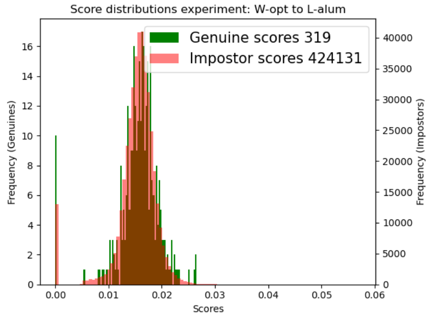


(e) W-opt to L-alum

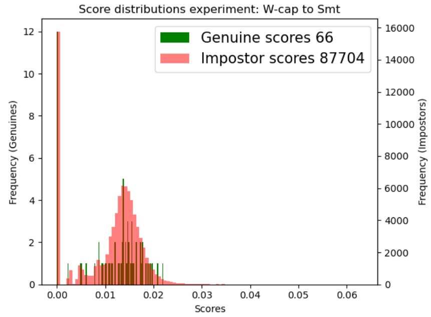


(f) W-cap to Smt

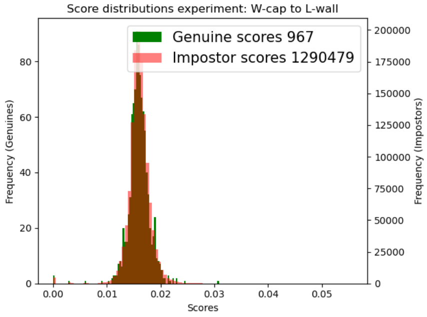


(g) W-cap to L-wall

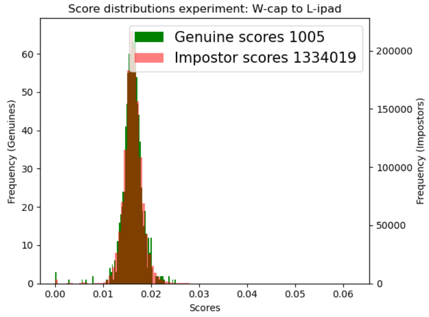


(h) W-cap to L-ipad

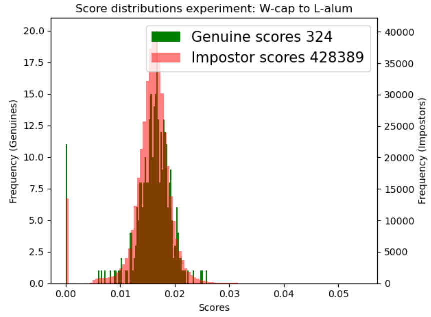


(i) W-cap to L-alum

Fig. 30: Distributions of the MCC (part 3/4) comparison scores in the 'Latent in the Wild' database

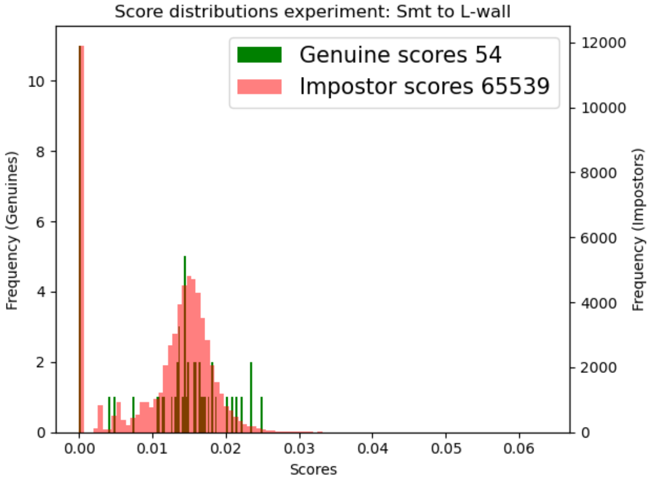


(a) Smt to L-wall

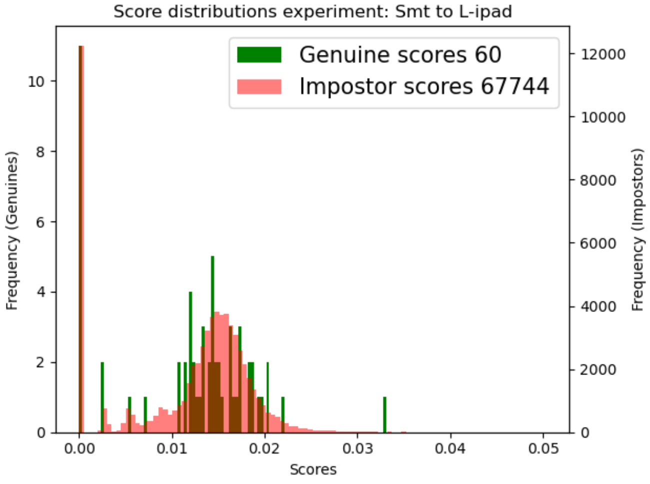


(b) Smt to L-ipad

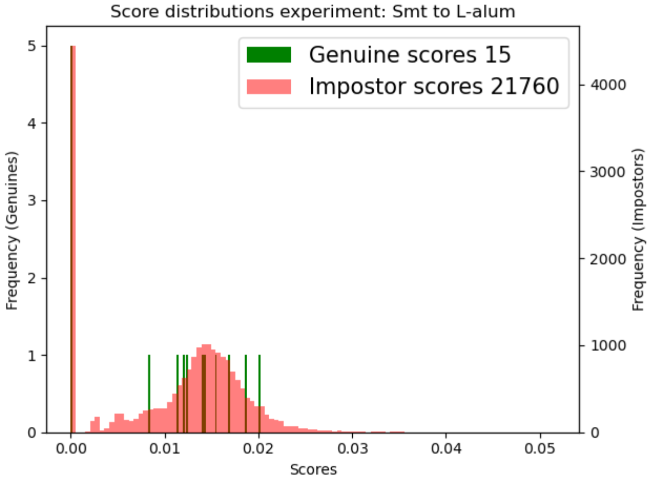


(c) Smt to L-alum

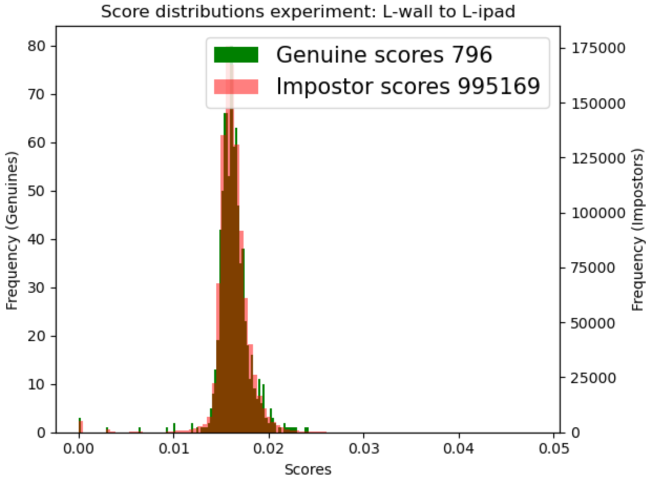


(d) L-wall to L-ipad

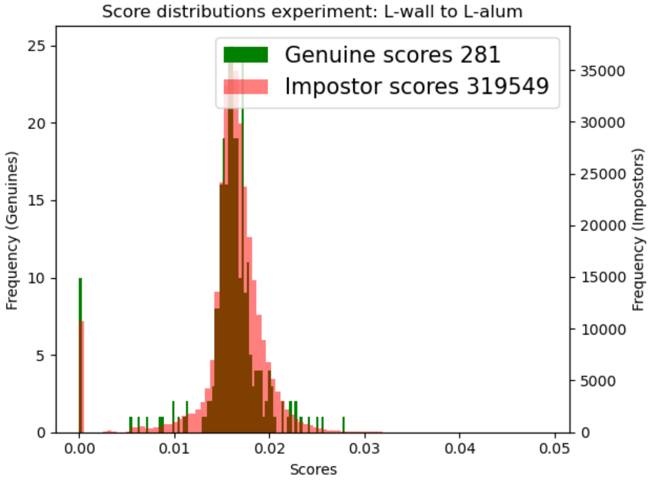


(e) L-wall to L-alum

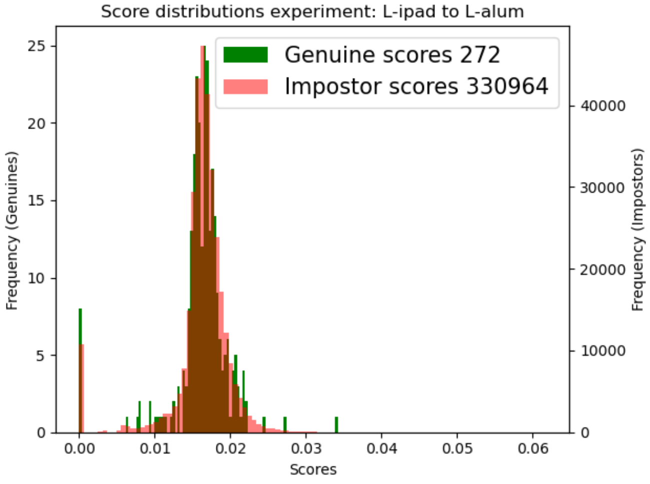


(f) L-ipad to L-alum

Fig. 31: Distributions of the MCC (part 4/4) comparison scores in the 'Latent in the Wild' database

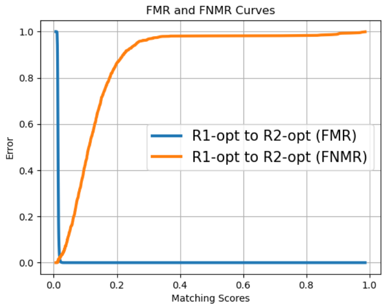


(a) R1-opt to R2-opt

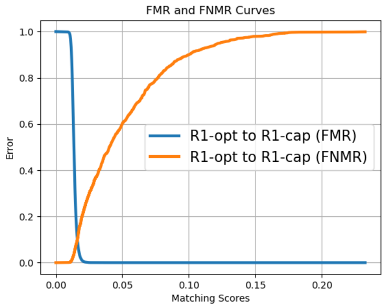


(b) R1-opt to R1-cap

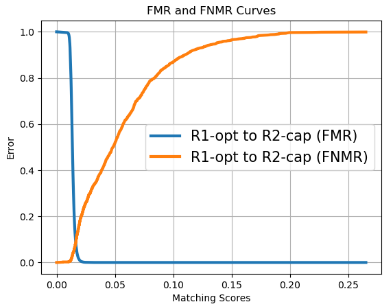


(c) R1-opt to R2-cap

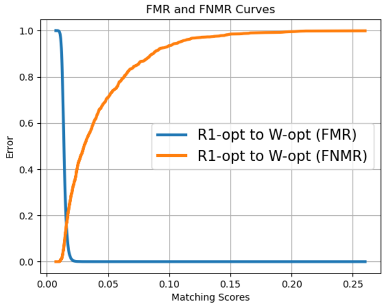


(d) R1-opt to W-opt

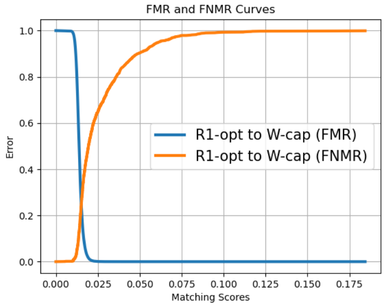


(e) R1-opt to W-cap

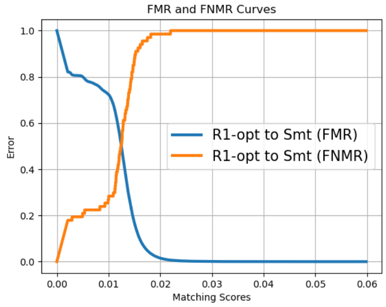


(f) R1-opt to Smt

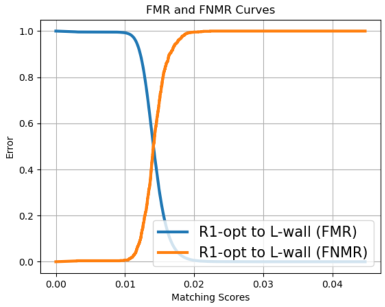


(g) R1-opt to L-wall

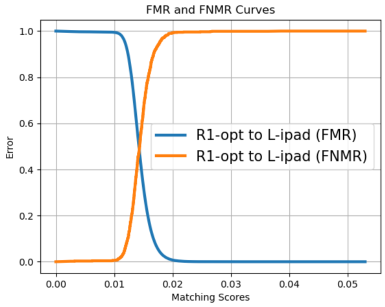


(h) R1-opt to L-ipad

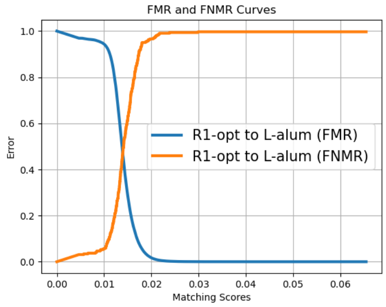


(i) R1-opt to L-alum

Fig. 32: FMR and FNMR curves of the MCC (part 1/4) comparison scores in the 'Latent in the Wild' database

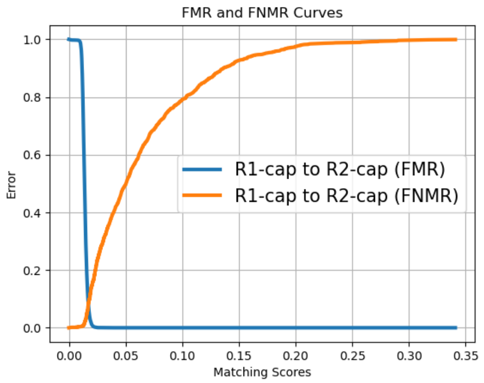


(a) R1-cap to R2-cap

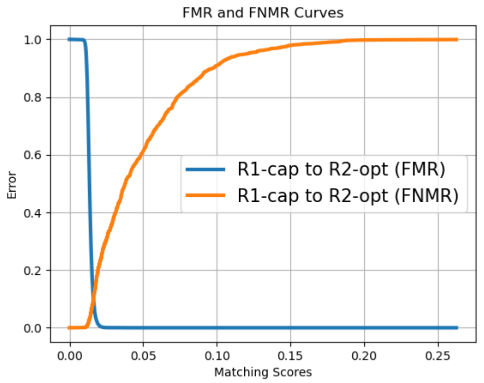


(b) R1-cap to R2-opt

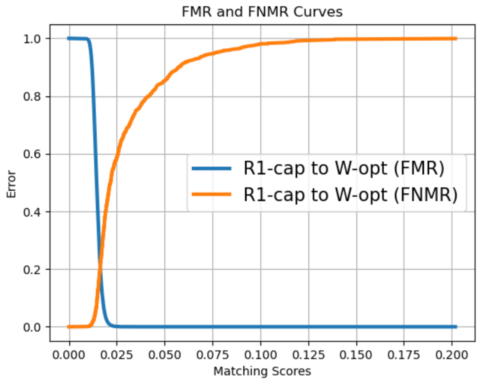


(c) R1-cap to W-opt

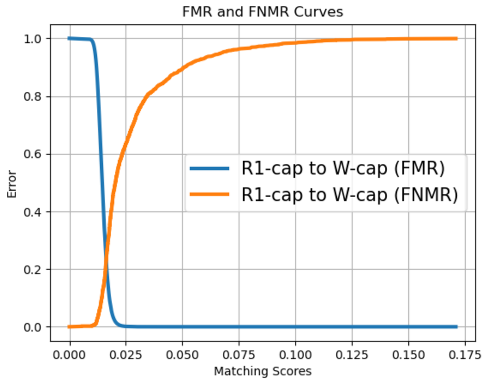


(d) R1-cap to W-cap

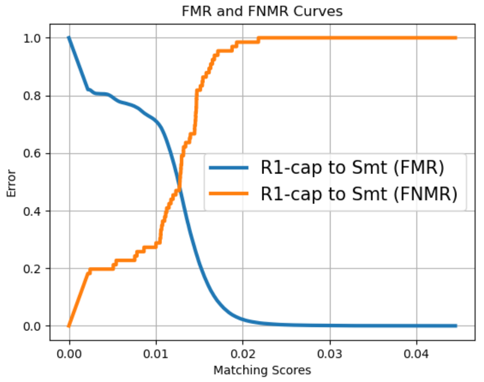


(e) R1-cap to Smt

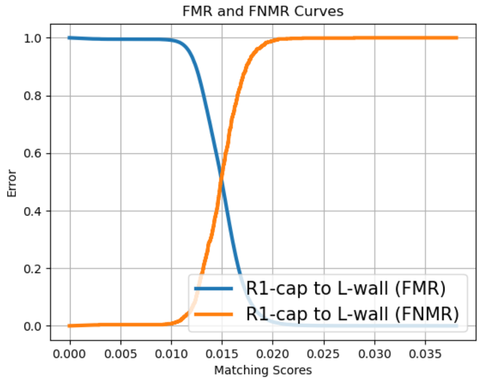


(f) R1-cap to L-wall

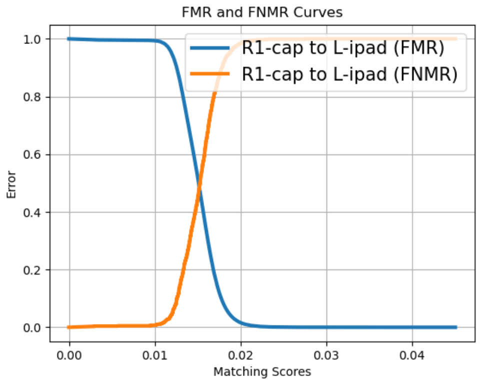


(g) R1-cap to L-ipad

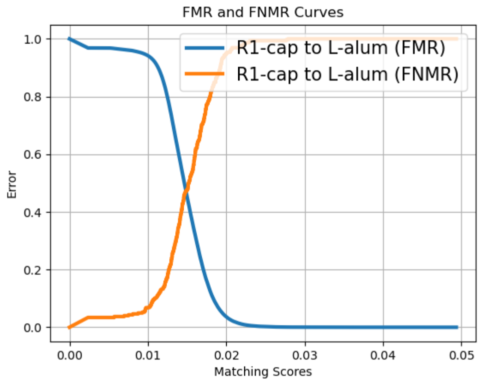


(h) R1-cap to L-alum

Fig. 33: FMR and FNMR curves of the MCC (part 2/4) comparison scores in the 'Latent in the Wild' database

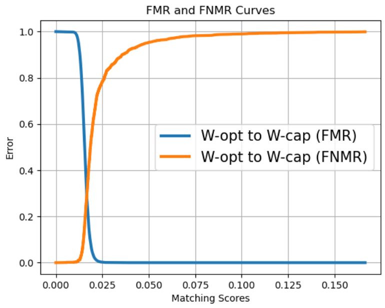


(a) W-opt to W-cap

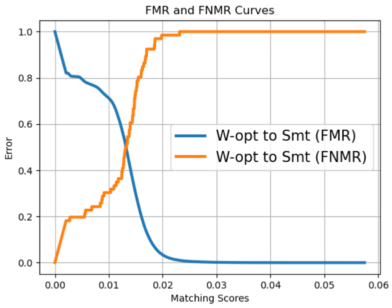


(b) W-opt to Smt

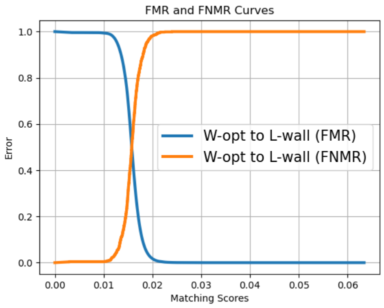


(c) W-opt to L-wall

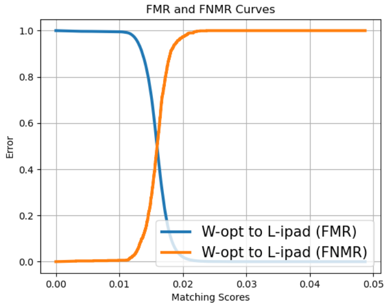


(d) W-opt to L-ipad

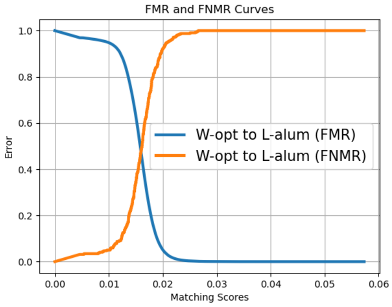


(e) W-opt to L-alum

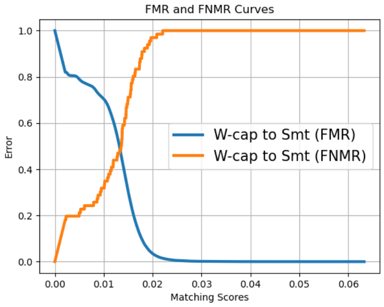


(f) W-cap to Smt

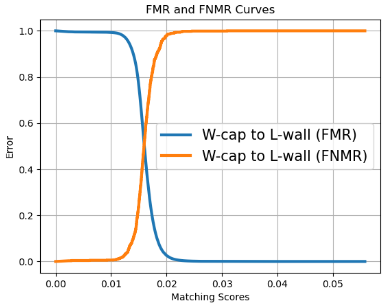


(g) W-cap to L-wall

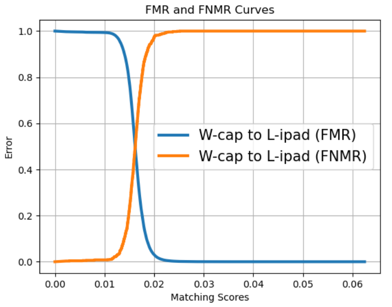


(h) W-cap to L-ipad

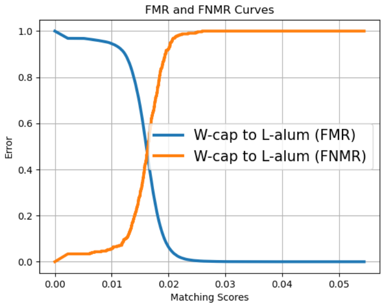


(i) W-cap to L-alum

Fig. 34: FMR and FNMR curves of the MCC (part 3/4) comparison scores in the 'Latent in the Wild' database

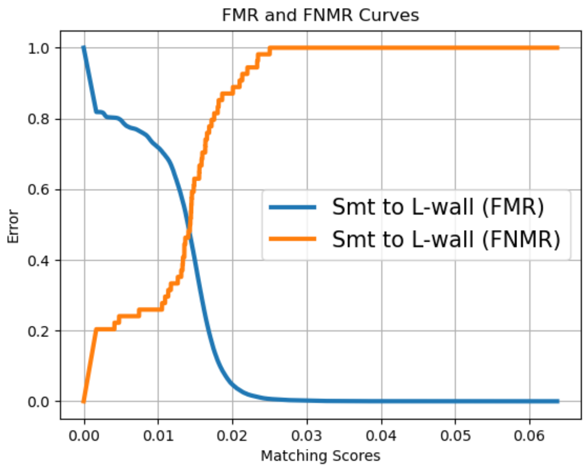


(a) Smt to L-wall

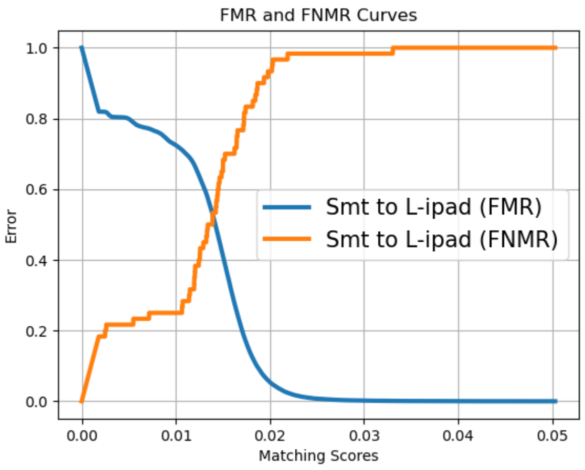


(b) Smt to L-ipad

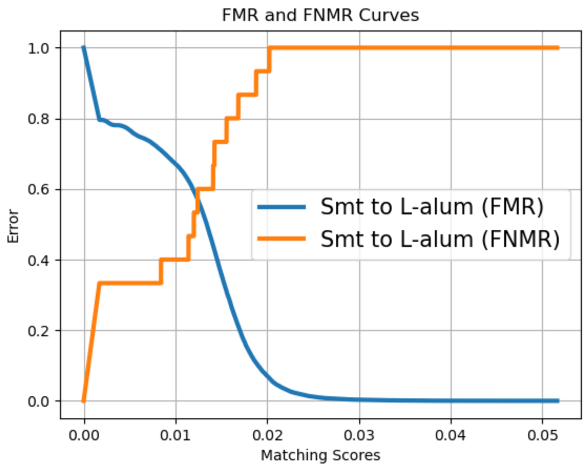


(c) Smt to L-alum

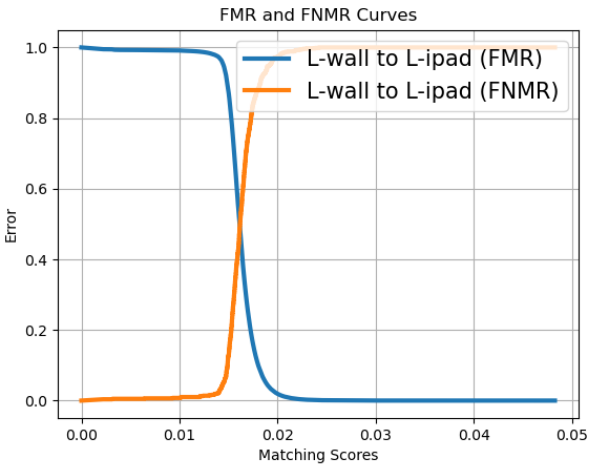


(d) L-wall to L-ipad

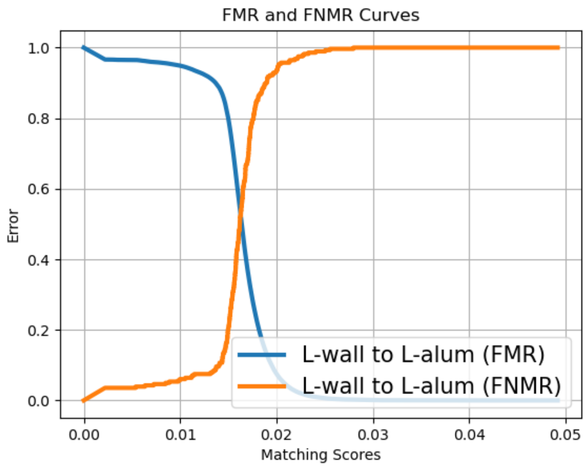


(e) L-wall to L-alum

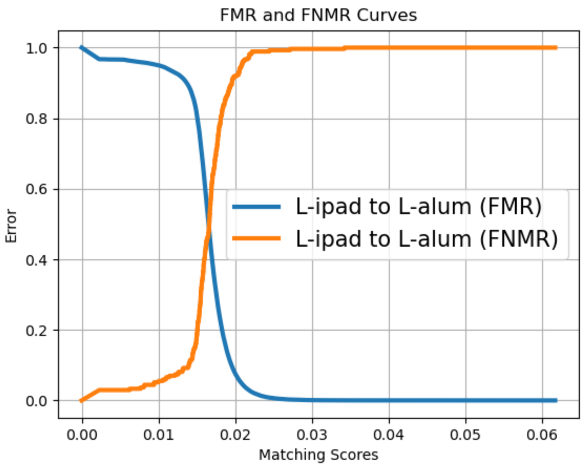


(f) L-ipad to L-alum

Fig. 35: FMR and FNMR curves of the MCC (part 4/4) comparison scores in the 'Latent in the Wild' database

TABLE XVII: Performance indicators measured on the 'Latent in the Wild' database for the MCC (part 1/4) comparison experiments.

| Comparison | GMean | GSTD | IMean | ISTD | SI | AUC | JI | JI_TH | MCC |
|---|---|---|---|---|---|---|---|---|---|
| R1-opt to R2-opt | 0.134 | 0.123 | 0.014 | 0.002 | 1.388 | 0.991 | 0.970 | 0.022 | 0.952 |
| R1-opt to R1-cap | 0.050 | 0.035 | 0.014 | 0.002 | 1.461 | 0.951 | 0.814 | 0.017 | 0.760 |
| R1-opt to R2-cap | 0.056 | 0.039 | 0.014 | 0.002 | 1.531 | 0.960 | 0.842 | 0.018 | 0.785 |
| R1-opt to W-opt | 0.042 | 0.033 | 0.014 | 0.002 | 1.190 | 0.913 | 0.728 | 0.018 | 0.663 |
| R1-opt to W-cap | 0.026 | 0.018 | 0.014 | 0.002 | 0.976 | 0.837 | 0.539 | 0.016 | 0.435 |
| R1-opt to Smt | 0.011 | 0.006 | 0.011 | 0.006 | 0.019 | 0.491 | 0.046 | 0.011 | 0.003 |
| R1-opt to L-wall | 0.014 | 0.002 | 0.014 | 0.002 | 0.004 | 0.503 | 0.034 | 0.014 | 0.002 |
| R1-opt to L-ipad | 0.014 | 0.002 | 0.014 | 0.002 | 0.035 | 0.509 | 0.032 | 0.014 | 0.016 |
| R1-opt to L-alum | 0.014 | 0.005 | 0.014 | 0.003 | 0.120 | 0.542 | 0.103 | 0.015 | 0.056 |
| | | | | | | | | | |
| Comparison | MCC_TH | EERL | EERH | EER | 0FMR | FMR1000 | FMR100 | FMR20 | FMR10 |
| R1-opt to R2-opt | 0.039 | 0.022 | 0.022 | 0.022 | 0.962 | 0.034 | 0.025 | 0.016 | 0.016 |
| R1-opt to R1-cap | 0.031 | 0.100 | 0.100 | 0.100 | 0.983 | 0.274 | 0.200 | 0.136 | 0.101 |
| R1-opt to R2-cap | 0.033 | 0.085 | 0.085 | 0.085 | 0.968 | 0.243 | 0.174 | 0.114 | 0.081 |
| R1-opt to W-opt | 0.031 | 0.159 | 0.160 | 0.160 | 0.998 | 0.387 | 0.296 | 0.223 | 0.183 |
| R1-opt to W-cap | 0.033 | 0.247 | 0.247 | 0.247 | 0.979 | 0.642 | 0.531 | 0.424 | 0.366 |
| R1-opt to Smt | 0.022 | 0.507 | 0.507 | 0.507 | 1.000 | 1.000 | 0.985 | 0.955 | 0.925 |
| R1-opt to L-wall | 0.014 | 0.501 | 0.501 | 0.501 | 1.000 | 1.000 | 0.994 | 0.946 | 0.901 |
| R1-opt to L-ipad | 0.036 | 0.486 | 0.486 | 0.486 | 1.000 | 0.996 | 0.990 | 0.942 | 0.898 |
| R1-opt to L-alum | 0.065 | 0.471 | 0.471 | 0.471 | 0.997 | 0.994 | 0.978 | 0.950 | 0.861 |
| | | | | | | | | | |
| Comparison | 0FNMR | EER_TH | 0FMR_TH | FMR1000_TH | FMR100_TH | FMR20_TH | FMR10_TH | 0FNMR_TH | |
| R1-opt to R2-opt | 0.993 | 0.019 | 0.286 | 0.025 | 0.020 | 0.017 | 0.016 | 0.011 | |
| R1-opt to R1-cap | 1.000 | 0.016 | 0.160 | 0.024 | 0.020 | 0.017 | 0.016 | 0.000 | |
| R1-opt to R2-cap | 1.000 | 0.016 | 0.155 | 0.024 | 0.020 | 0.017 | 0.016 | 0.000 | |
| R1-opt to W-opt | 0.996 | 0.016 | 0.216 | 0.024 | 0.020 | 0.018 | 0.017 | 0.010 | |
| R1-opt to W-cap | 1.000 | 0.015 | 0.078 | 0.024 | 0.020 | 0.018 | 0.017 | 0.000 | |
| R1-opt to Smt | 1.000 | 0.012 | 0.060 | 0.028 | 0.021 | 0.017 | 0.016 | 0.000 | |
| R1-opt to L-wall | 1.000 | 0.014 | 0.045 | 0.022 | 0.019 | 0.017 | 0.017 | 0.000 | |
| R1-opt to L-ipad | 1.000 | 0.014 | 0.053 | 0.023 | 0.020 | 0.018 | 0.017 | 0.000 | |
| R1-opt to L-alum | 1.000 | 0.014 | 0.065 | 0.026 | 0.021 | 0.018 | 0.017 | 0.000 | |

*Note:* ***GMean:*** *Genuine scores distribution mean;* ***GSTD:*** *Genuine scores distribution standard deviation;* ***IMean:*** *Impostor scores distribution mean;* ***ISTD:*** *Impostor scores distribution standard deviation;* ***AUC:*** *Area under the ROC curve;* ***SI:*** *Sensitivity Index;* ***JI:*** *Youden's J Index;* ***TH:*** *THreshold;* ***MCC:*** *Matthews Correlation Coefficient;* ***EER:*** *Equal Error Rate;* ***EERL:*** *EER low;* ***EERH:*** *EER high.*

TABLE XVIII: Performance indicators measured on the 'Latent in the Wild' database for the MCC (part 2/4) comparison experiments.

| Comparison | GMean | GSTD | IMean | ISTD | SI | AUC | JI | JI_TH | MCC |
|---|---|---|---|---|---|---|---|---|---|
| R1-cap to R2-cap | 0.066 | 0.052 | 0.014 | 0.002 | 1.409 | 0.971 | 0.861 | 0.019 | 0.798 |
| R1-cap to R2-opt | 0.049 | 0.035 | 0.014 | 0.002 | 1.411 | 0.957 | 0.819 | 0.017 | 0.750 |
| R1-cap to W-opt | 0.030 | 0.022 | 0.015 | 0.002 | 1.001 | 0.879 | 0.612 | 0.017 | 0.519 |
| R1-cap to W-cap | 0.028 | 0.019 | 0.015 | 0.002 | 0.942 | 0.852 | 0.566 | 0.017 | 0.402 |
| R1-cap to Smt | 0.011 | 0.006 | 0.011 | 0.006 | 0.031 | 0.491 | 0.063 | 0.014 | 0.004 |
| R1-cap to L-wall | 0.015 | 0.002 | 0.015 | 0.002 | 0.026 | 0.491 | 0.013 | 0.014 | 0.003 |
| R1-cap to L-ipad | 0.015 | 0.002 | 0.015 | 0.002 | 0.039 | 0.514 | 0.038 | 0.015 | 0.002 |
| R1-cap to L-alum | 0.015 | 0.004 | 0.014 | 0.004 | 0.114 | 0.546 | 0.100 | 0.016 | 0.007 |
| | | | | | | | | | |
| Comparison | MCC_TH | EERL | EERH | EER | 0FMR | FMR1000 | FMR100 | FMR20 | FMR10 |
| R1-cap to R2-cap | 0.033 | 0.082 | 0.082 | 0.082 | 0.568 | 0.220 | 0.147 | 0.096 | 0.070 |
| R1-cap to R2-opt | 0.032 | 0.100 | 0.101 | 0.101 | 0.910 | 0.286 | 0.210 | 0.133 | 0.102 |
| R1-cap to W-opt | 0.032 | 0.207 | 0.207 | 0.207 | 0.914 | 0.580 | 0.479 | 0.366 | 0.293 |
| R1-cap to W-cap | 0.032 | 0.231 | 0.231 | 0.231 | 0.954 | 0.641 | 0.539 | 0.416 | 0.337 |
| R1-cap to Smt | 0.014 | 0.485 | 0.485 | 0.485 | 1.000 | 1.000 | 1.000 | 0.955 | 0.939 |
| R1-cap to L-wall | 0.028 | 0.510 | 0.511 | 0.511 | 1.000 | 0.999 | 0.993 | 0.960 | 0.910 |
| R1-cap to L-ipad | 0.027 | 0.485 | 0.485 | 0.485 | 1.000 | 0.999 | 0.991 | 0.947 | 0.896 |
| R1-cap to L-alum | 0.019 | 0.472 | 0.472 | 0.472 | 1.000 | 0.994 | 0.978 | 0.932 | 0.836 |
| | | | | | | | | | |
| Comparison | 0FNMR | EER_TH | 0FMR_TH | FMR1000_TH | FMR100_TH | FMR20_TH | FMR10_TH | 0FNMR_TH | |
| R1-cap to R2-cap | 1.000 | 0.017 | 0.058 | 0.024 | 0.020 | 0.018 | 0.017 | 0.000 | |
| R1-cap to R2-opt | 1.000 | 0.016 | 0.100 | 0.024 | 0.020 | 0.017 | 0.016 | 0.000 | |
| R1-cap to W-opt | 1.000 | 0.016 | 0.060 | 0.025 | 0.021 | 0.019 | 0.018 | 0.000 | |
| R1-cap to W-cap | 1.000 | 0.016 | 0.069 | 0.025 | 0.021 | 0.019 | 0.018 | 0.000 | |
| R1-cap to Smt | 1.000 | 0.013 | 0.044 | 0.030 | 0.022 | 0.018 | 0.017 | 0.000 | |
| R1-cap to L-wall | 1.000 | 0.015 | 0.038 | 0.024 | 0.020 | 0.018 | 0.018 | 0.000 | |
| R1-cap to L-ipad | 1.000 | 0.015 | 0.045 | 0.024 | 0.021 | 0.019 | 0.018 | 0.000 | |
| R1-cap to L-alum | 1.000 | 0.015 | 0.049 | 0.027 | 0.022 | 0.019 | 0.018 | 0.000 | |

*Note:* ***GMean:*** *Genuine scores distribution mean;* ***GSTD:*** *Genuine scores distribution standard deviation;* ***IMean:*** *Impostor scores distribution mean;* ***ISTD:*** *Impostor scores distribution standard deviation;* ***AUC:*** *Area under the ROC curve;* ***SI:*** *Sensitivity Index;* ***JI:*** *Youden's J Index;* ***TH:*** *THreshold;* ***MCC:*** *Matthews Correlation Coefficient;* ***EER:*** *Equal Error Rate;* ***EERL:*** *EER low;* ***EERH:*** *EER high.*

TABLE XIX: Performance indicators measured on the 'Latent in the Wild' database for the MCC (part 3/4) comparison experiments.

| Comparison | GMean | GSTD | IMean | ISTD | SI | AUC | JI | JI_TH | MCC |
|---|---|---|---|---|---|---|---|---|---|
| W-opt to W-cap | 0.023 | 0.015 | 0.016 | 0.002 | 0.701 | 0.791 | 0.441 | 0.017 | 0.250 |
| W-opt to Smt | 0.011 | 0.006 | 0.011 | 0.006 | 0.030 | 0.494 | 0.056 | 0.012 | 0.003 |
| W-opt to L-wall | 0.016 | 0.002 | 0.016 | 0.002 | 0.001 | 0.499 | 0.016 | 0.018 | 0.001 |
| W-opt to L-ipad | 0.016 | 0.002 | 0.016 | 0.002 | 0.005 | 0.499 | 0.014 | 0.016 | 0.002 |
| W-opt to L-alum | 0.016 | 0.004 | 0.015 | 0.004 | 0.084 | 0.531 | 0.060 | 0.016 | 0.005 |
| W-cap to Smt | 0.011 | 0.006 | 0.011 | 0.006 | 0.020 | 0.499 | 0.050 | 0.014 | 0.004 |
| W-cap to L-wall | 0.016 | 0.002 | 0.016 | 0.002 | 0.023 | 0.490 | 0.008 | 0.019 | 0.002 |
| W-cap to L-ipad | 0.016 | 0.002 | 0.016 | 0.002 | 0.014 | 0.498 | 0.011 | 0.016 | 0.001 |
| W-cap to L-alum | 0.016 | 0.004 | 0.016 | 0.004 | 0.049 | 0.529 | 0.060 | 0.018 | 0.004 |
| | | | | | | | | | |
| Comparison | MCC_TH | EERL | EERH | EER | 0FMR | FMR1000 | FMR100 | FMR20 | FMR10 |
| W-opt to W-cap | 0.035 | 0.288 | 0.288 | 0.288 | 0.981 | 0.807 | 0.717 | 0.565 | 0.486 |
| W-opt to Smt | 0.012 | 0.500 | 0.500 | 0.500 | 1.000 | 1.000 | 0.985 | 0.970 | 0.924 |
| W-opt to L-wall | 0.018 | 0.501 | 0.501 | 0.501 | 1.000 | 0.999 | 0.988 | 0.949 | 0.888 |
| W-opt to L-ipad | 0.022 | 0.499 | 0.499 | 0.499 | 1.000 | 1.000 | 0.988 | 0.949 | 0.913 |
| W-opt to L-alum | 0.019 | 0.476 | 0.476 | 0.476 | 1.000 | 1.000 | 0.981 | 0.922 | 0.843 |
| W-cap to Smt | 0.017 | 0.485 | 0.485 | 0.485 | 1.000 | 1.000 | 1.000 | 0.939 | 0.879 |
| W-cap to L-wall | 0.031 | 0.508 | 0.508 | 0.508 | 1.000 | 0.999 | 0.990 | 0.957 | 0.902 |
| W-cap to L-ipad | 0.022 | 0.495 | 0.495 | 0.495 | 1.000 | 1.000 | 0.988 | 0.946 | 0.905 |
| W-cap to L-alum | 0.018 | 0.472 | 0.472 | 0.472 | 1.000 | 1.000 | 0.988 | 0.951 | 0.883 |
| | | | | | | | | | |
| Comparison | 0FNMR | EER_TH | 0FMR_TH | FMR1000_TH | FMR100_TH | FMR20_TH | FMR10_TH | 0FNMR_TH | |
| W-opt to W-cap | 1.000 | 0.017 | 0.073 | 0.026 | 0.022 | 0.019 | 0.018 | 0.000 | |
| W-opt to Smt | 1.000 | 0.013 | 0.057 | 0.031 | 0.023 | 0.019 | 0.018 | 0.000 | |
| W-opt to L-wall | 1.000 | 0.016 | 0.063 | 0.024 | 0.021 | 0.019 | 0.018 | 0.000 | |
| W-opt to L-ipad | 1.000 | 0.016 | 0.049 | 0.024 | 0.021 | 0.019 | 0.018 | 0.000 | |
| W-opt to L-alum | 1.000 | 0.016 | 0.057 | 0.028 | 0.023 | 0.020 | 0.019 | 0.000 | |
| W-cap to Smt | 1.000 | 0.013 | 0.063 | 0.031 | 0.023 | 0.019 | 0.018 | 0.000 | |
| W-cap to L-wall | 1.000 | 0.016 | 0.056 | 0.026 | 0.021 | 0.019 | 0.018 | 0.000 | |
| W-cap to L-ipad | 1.000 | 0.016 | 0.062 | 0.026 | 0.022 | 0.019 | 0.018 | 0.000 | |
| W-cap to L-alum | 1.000 | 0.016 | 0.054 | 0.029 | 0.023 | 0.020 | 0.019 | 0.000 | |

*Note:* ***GMean:*** *Genuine scores distribution mean;* ***GSTD:*** *Genuine scores distribution standard deviation;* ***IMean:*** *Impostor scores distribution mean;* ***ISTD:*** *Impostor scores distribution standard deviation;* ***AUC:*** *Area under the ROC curve;* ***SI:*** *Sensitivity Index;* ***JI:*** *Youden's J Index;* ***TH:*** *THreshold;* ***MCC:*** *Matthews Correlation Coefficient;* ***EER:*** *Equal Error Rate;* ***EERL:*** *EER low;* ***EERH:*** *EER high.*

TABLE XX: Performance indicators measured on the 'Latent in the Wild' database for the MCC (part 4/4) comparison experiments.

| Comparison | GMean | GSTD | IMean | ISTD | SI | AUC | JI | JI_TH | MCC |
|---|---|---|---|---|---|---|---|---|---|
| Smt to L-wall | 0.012 | 0.007 | 0.012 | 0.007 | 0.050 | 0.517 | 0.084 | 0.020 | 0.013 |
| Smt to L-ipad | 0.012 | 0.007 | 0.012 | 0.007 | 0.011 | 0.485 | 0.045 | 0.018 | 0.014 |
| Smt to L-alum | 0.010 | 0.007 | 0.011 | 0.007 | 0.252 | 0.430 | 0.026 | 0.019 | 0.002 |
| L-wall to L-ipad | 0.016 | 0.002 | 0.016 | 0.002 | 0.037 | 0.507 | 0.030 | 0.016 | 0.002 |
| L-wall to L-alum | 0.016 | 0.004 | 0.016 | 0.004 | 0.060 | 0.468 | 0.024 | 0.014 | 0.002 |
| L-ipad to L-alum | 0.016 | 0.004 | 0.016 | 0.004 | 0.003 | 0.493 | 0.031 | 0.017 | 0.007 |
| | | | | | | | | | |
| Comparison | MCC_TH | EERL | EERH | EER | 0FMR | FMR1000 | FMR100 | FMR20 | FMR10 |
| Smt to L-wall | 0.021 | 0.481 | 0.481 | 0.481 | 1.000 | 1.000 | 0.981 | 0.870 | 0.852 |
| Smt to L-ipad | 0.033 | 0.517 | 0.531 | 0.524 | 1.000 | 1.000 | 0.983 | 0.933 | 0.883 |
| Smt to L-alum | 0.019 | 0.533 | 0.571 | 0.552 | 1.000 | 1.000 | 1.000 | 1.000 | 0.933 |
| L-wall to L-ipad | 0.019 | 0.490 | 0.491 | 0.490 | 1.000 | 1.000 | 0.987 | 0.935 | 0.883 |
| L-wall to L-alum | 0.014 | 0.523 | 0.523 | 0.523 | 1.000 | 1.000 | 0.986 | 0.957 | 0.922 |
| L-ipad to L-alum | 0.034 | 0.485 | 0.487 | 0.486 | 1.000 | 0.996 | 0.989 | 0.949 | 0.897 |
| | | | | | | | | | |
| Comparison | 0FNMR | EER_TH | 0FMR_TH | FMR1000_TH | FMR100_TH | FMR20_TH | FMR10_TH | 0FNMR_TH | |
| Smt to L-wall | 1.000 | 0.014 | 0.064 | 0.032 | 0.024 | 0.020 | 0.018 | 0.000 | |
| Smt to L-ipad | 1.000 | 0.014 | 0.050 | 0.033 | 0.024 | 0.020 | 0.019 | 0.000 | |
| Smt to L-alum | 1.000 | 0.012 | 0.052 | 0.035 | 0.026 | 0.021 | 0.019 | 0.000 | |
| L-wall to L-ipad | 1.000 | 0.016 | 0.048 | 0.025 | 0.021 | 0.019 | 0.018 | 0.000 | |
| L-wall to L-alum | 1.000 | 0.016 | 0.049 | 0.030 | 0.024 | 0.021 | 0.019 | 0.000 | |
| L-ipad to L-alum | 1.000 | 0.017 | 0.062 | 0.029 | 0.024 | 0.021 | 0.020 | 0.000 | |

*Note:* ***GMean:*** *Genuine scores distribution mean;* ***GSTD:*** *Genuine scores distribution standard deviation;* ***IMean:*** *Impostor scores distribution mean;* ***ISTD:*** *Impostor scores distribution standard deviation;* ***AUC:*** *Area under the ROC curve;* ***SI:*** *Sensitivity Index;* ***JI:*** *Youden's J Index;* ***TH:*** *THreshold;* ***MCC:*** *Matthews Correlation Coefficient;* ***EER:*** *Equal Error Rate;* ***EERL:*** *EER low;* ***EERH:*** *EER high.*

### *D. Supplementary results for the VeriFinger comparison experiment*

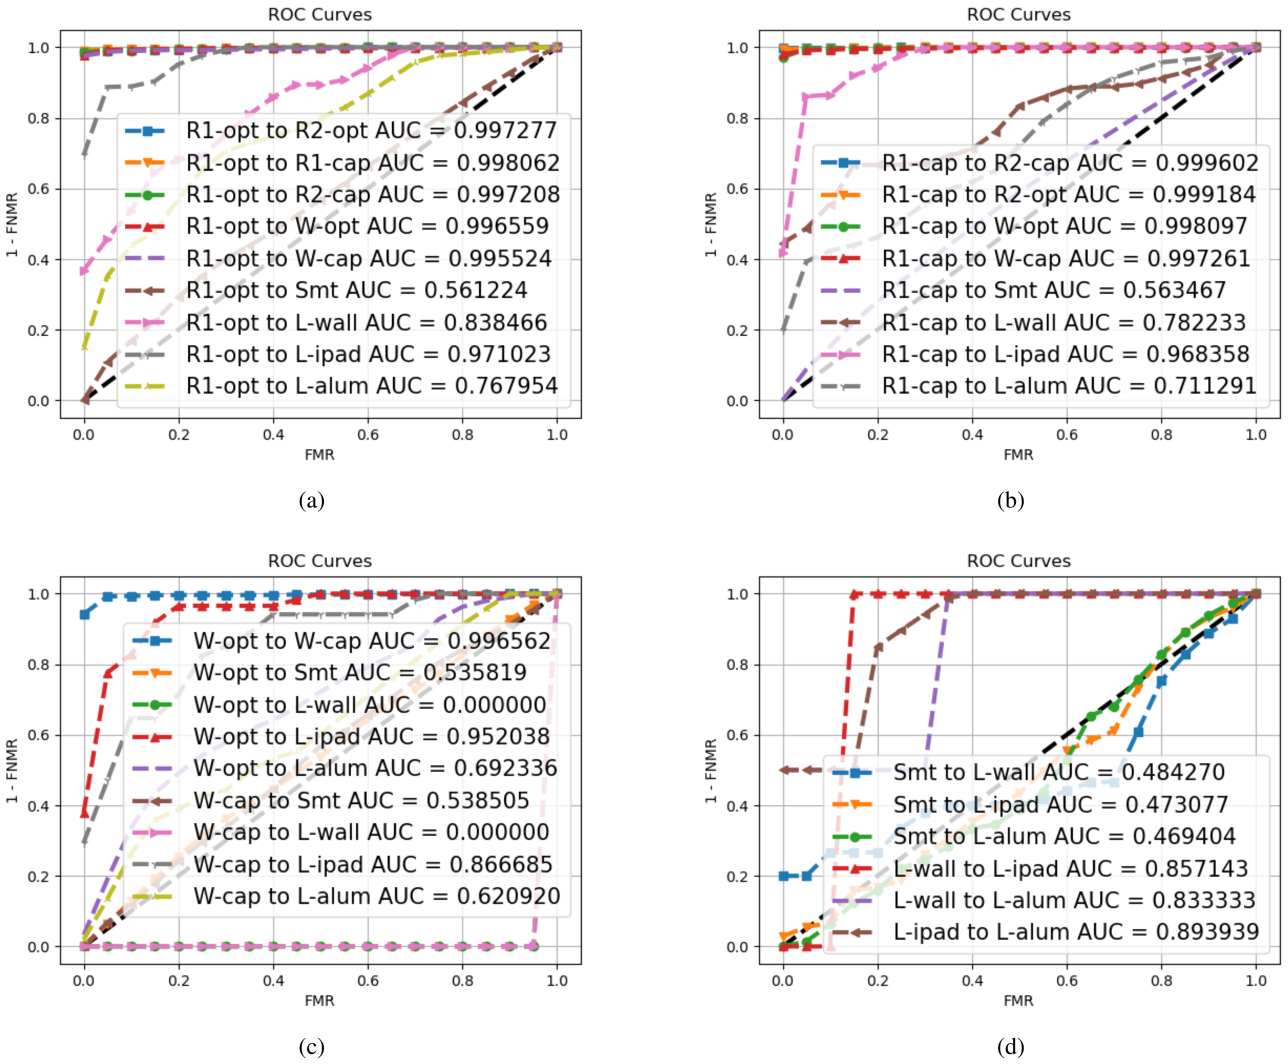


Fig. 36: ROC curve of the VeriFinger comparison experiments for the 'Latent in the Wild' database

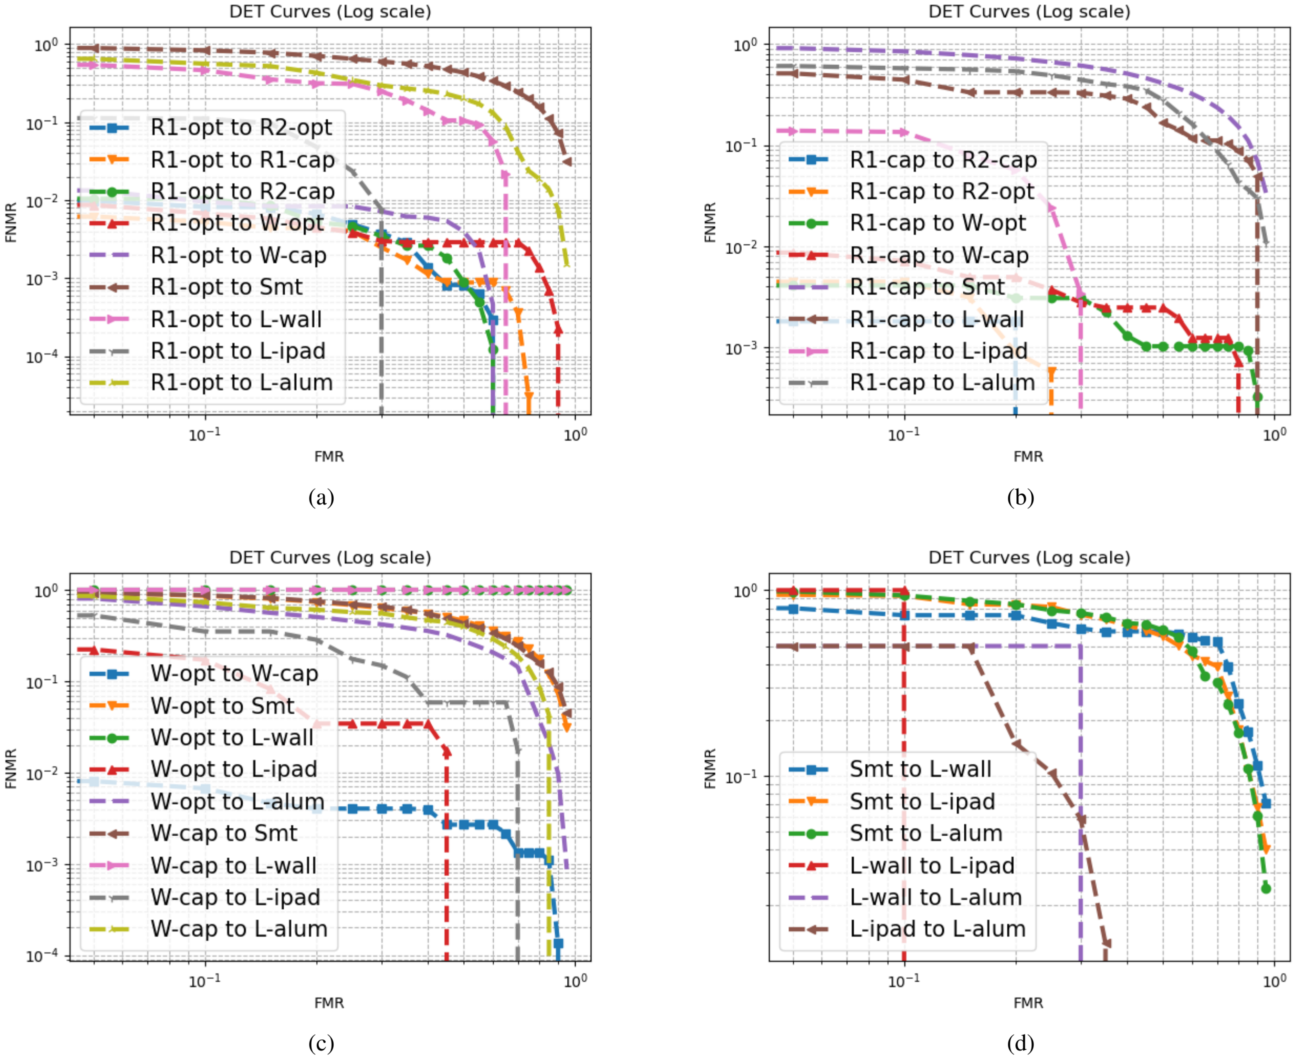


Fig. 37: DET curve of the VeriFinger comparison experiments for the 'Latent in the Wild' database

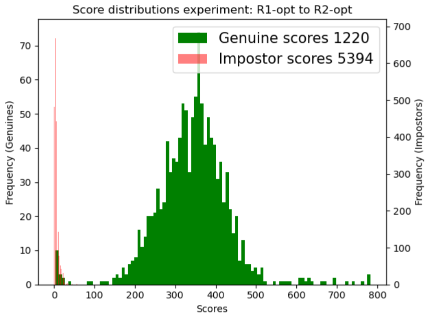


(a) R1-opt to R2-opt

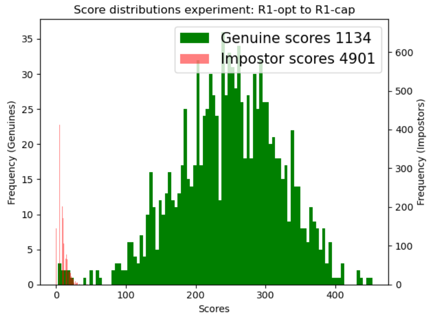


(b) R1-opt to R1-cap

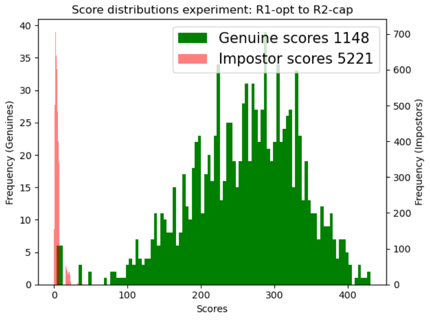


(c) R1-opt to R2-cap

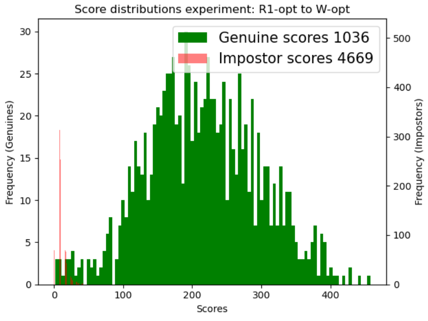


(d) R1-opt to W-opt

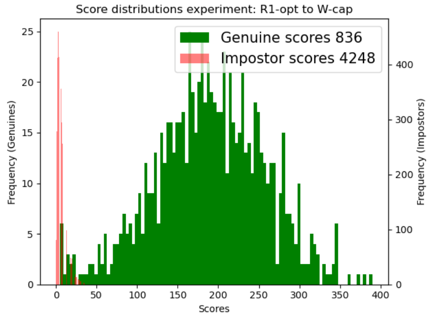


(e) R1-opt to W-cap

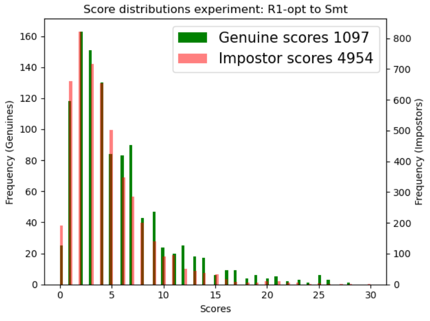


(f) R1-opt to Smt

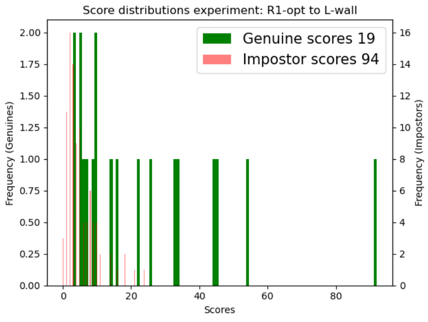


(g) R1-opt to L-wall

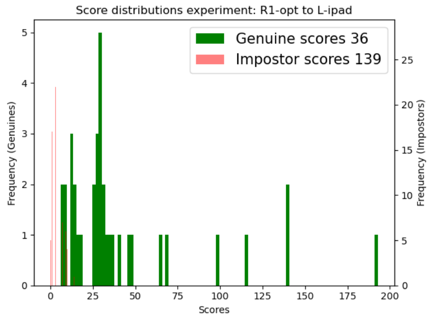


(h) R1-opt to L-ipad

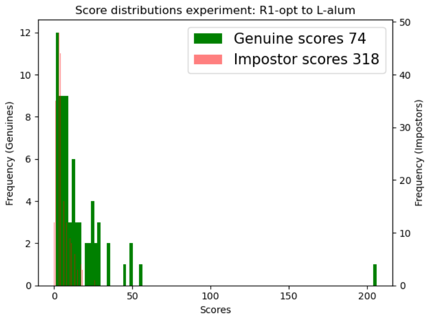


(i) R1-opt to L-alum

Fig. 38: Distributions of the VeriFinger (part 1/4) comparison scores in the 'Latent in the Wild' database

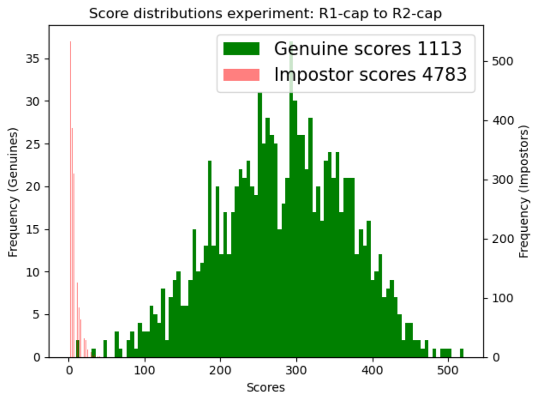


(a) R1-cap to R2-cap

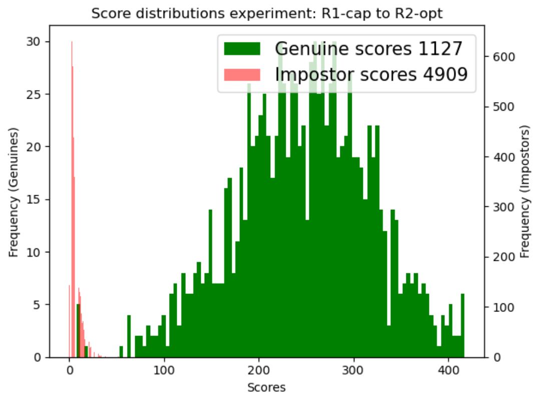


(b) R1-cap to R2-opt

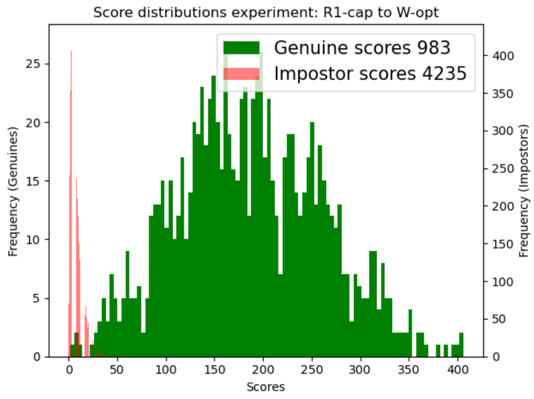


(c) R1-cap to W-opt

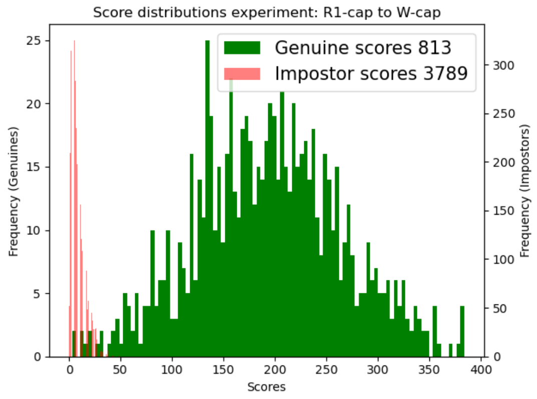


(d) R1-cap to W-cap

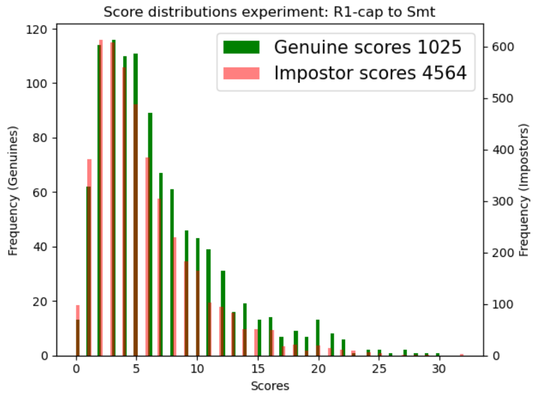


(e) R1-cap to Smt

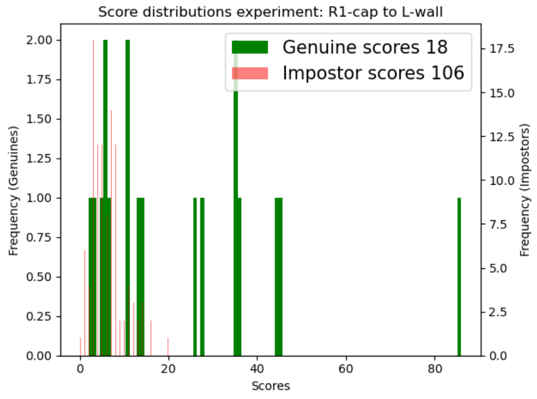


(f) R1-cap to L-wall

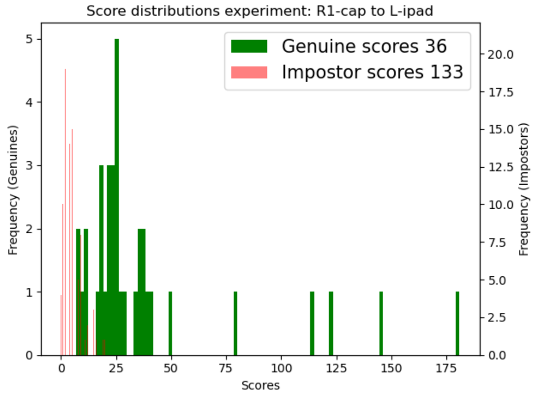


(g) R1-cap to L-ipad

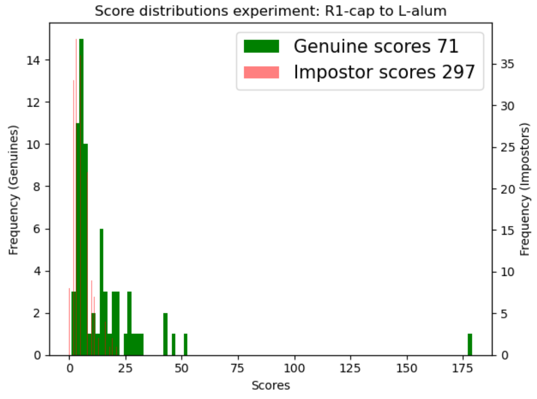


(h) R1-cap to L-alum

Fig. 39: Distributions of the VeriFinger (part 2/4) comparison scores in the 'Latent in the Wild' database

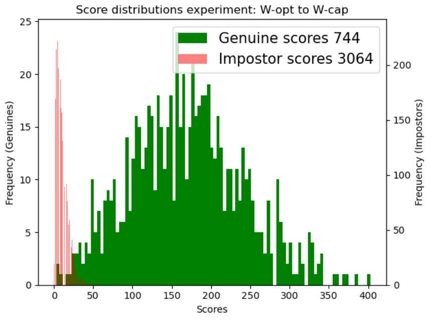


(a) W-opt to W-cap

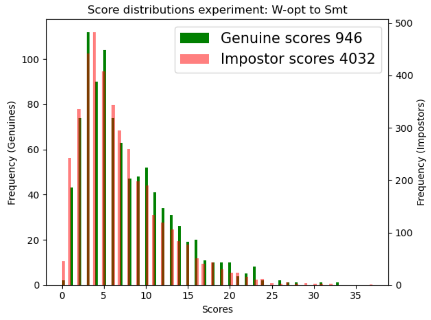


(b) W-opt to Smt

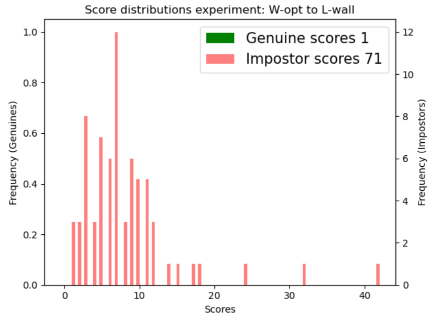


(c) W-opt to L-wall

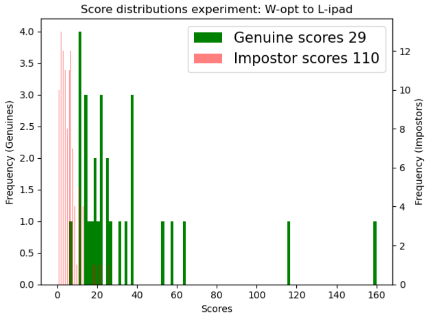


(d) W-opt to L-ipad

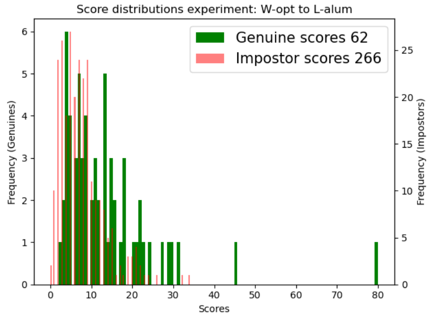


(e) W-opt to L-alum

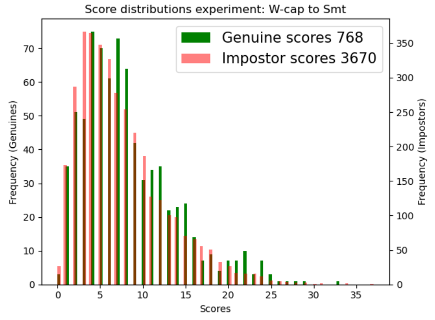


(f) W-cap to Smt

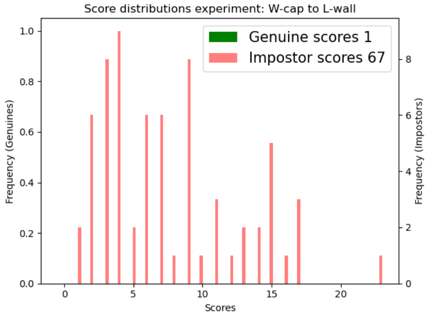


(g) W-cap to L-wall

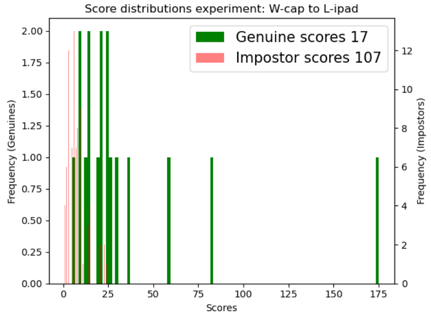


(h) W-cap to L-ipad

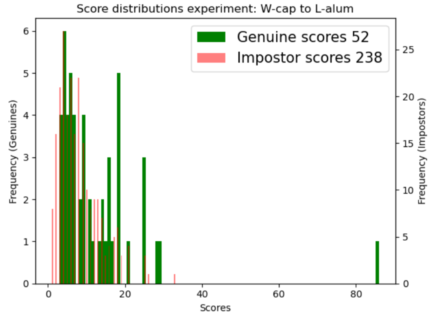


(i) W-cap to L-alum

Fig. 40: Distributions of the VeriFinger (part 3/4) comparison scores in the 'Latent in the Wild' database

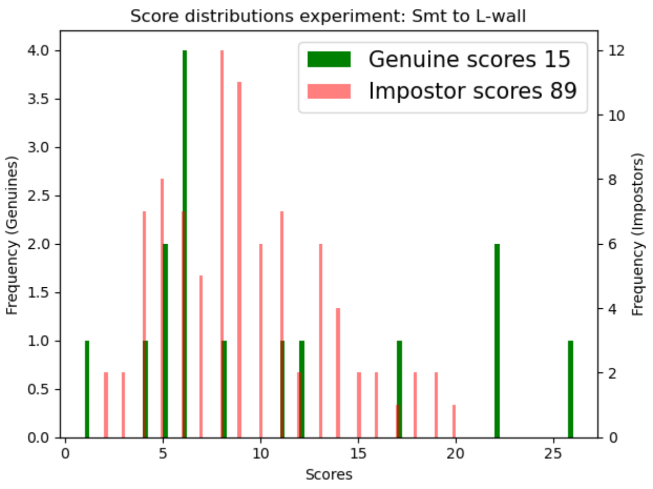


(a) Smt to L-wall

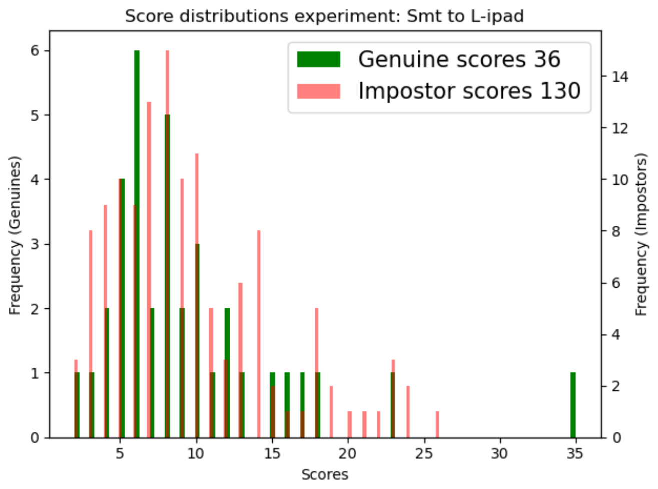


(b) Smt to L-ipad

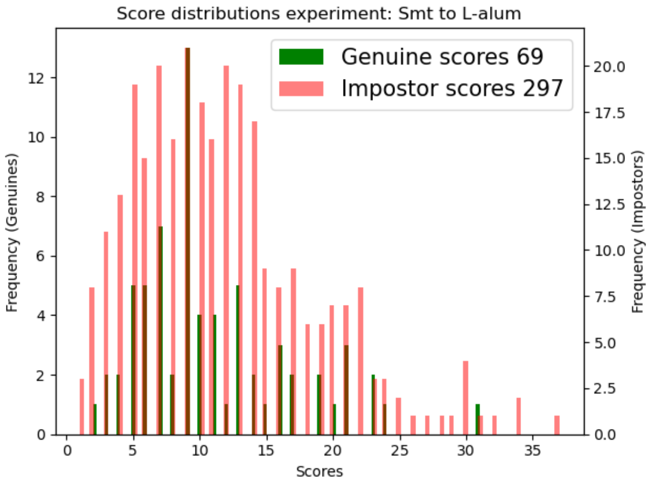


(c) Smt to L-alum

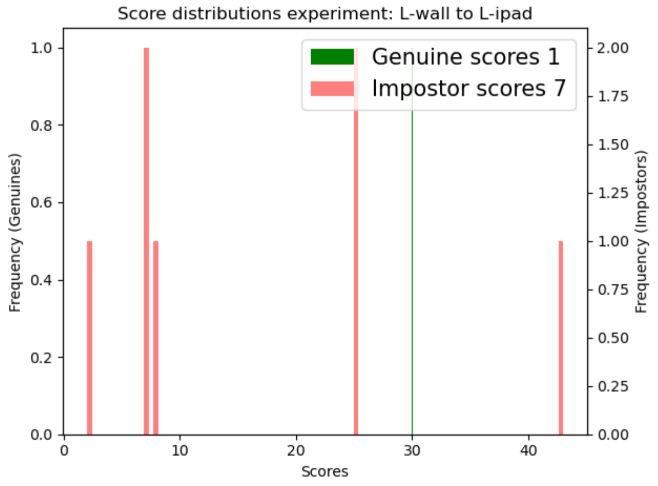


(d) L-wall to L-ipad

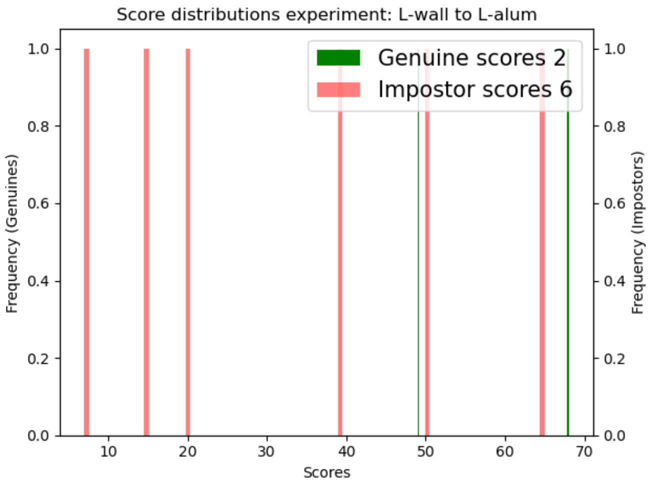


(e) L-wall to L-alum

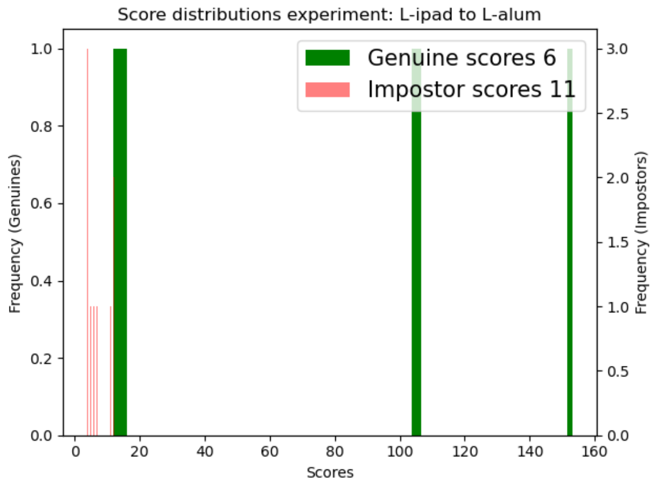


(f) L-ipad to L-alum

Fig. 41: Distributions of the VeriFinger (part 4/4) comparison scores in the 'Latent in the Wild' database

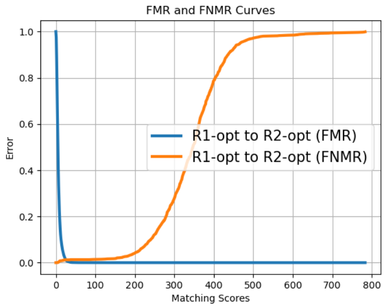


(a) R1-opt to R2-opt

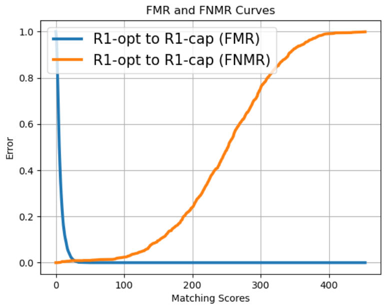


(b) R1-opt to R1-cap

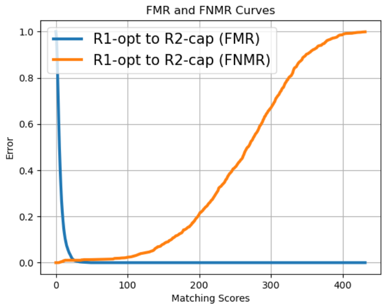


(c) R1-opt to R2-cap

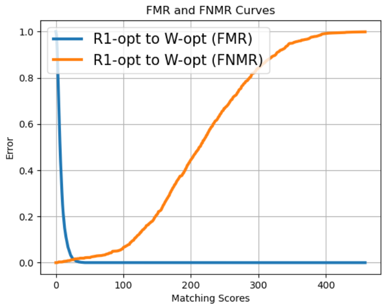


(d) R1-opt to W-opt

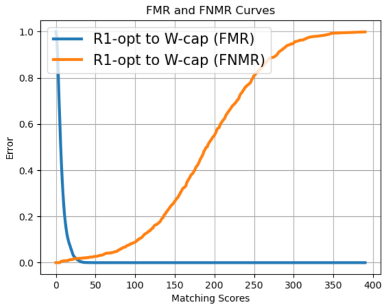


(e) R1-opt to W-cap

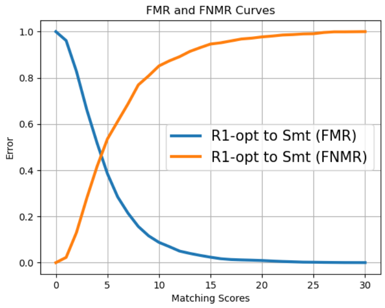


(f) R1-opt to Smt

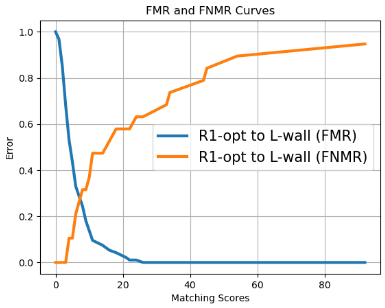


(g) R1-opt to L-wall

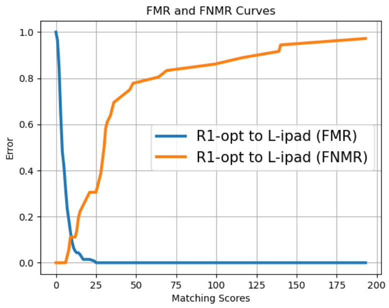


(h) R1-opt to L-ipad

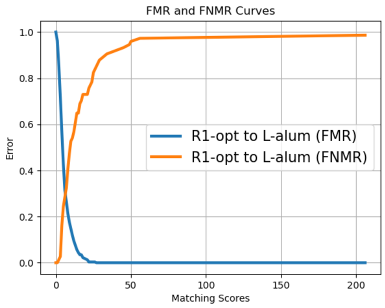


(i) R1-opt to L-alum

Fig. 42: FMR and FNMR curves of the VeriFinger (part 1/4) comparison scores in the 'Latent in the Wild' database

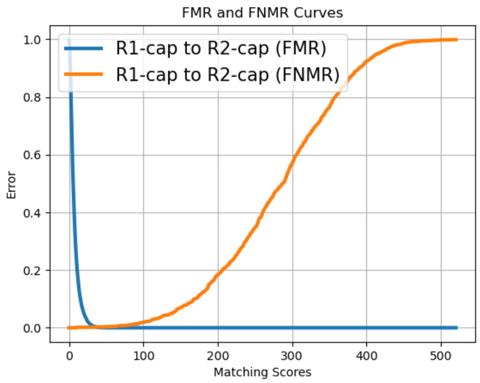


(a) R1-cap to R2-cap

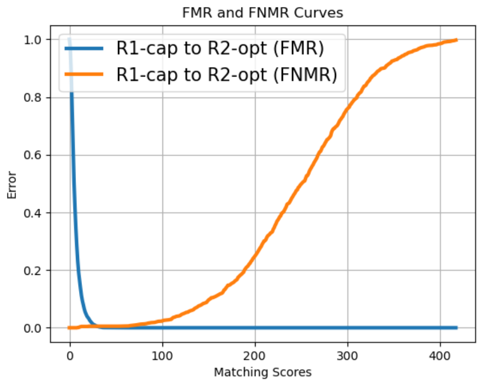


(b) R1-cap to R2-opt

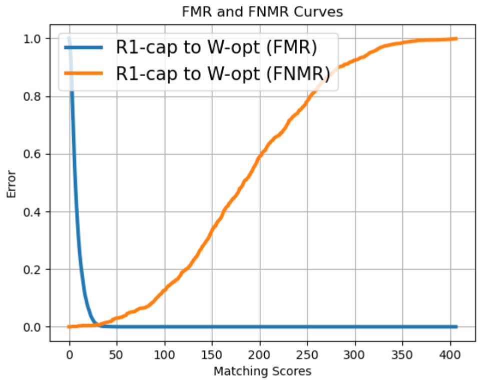


(c) R1-cap to W-opt

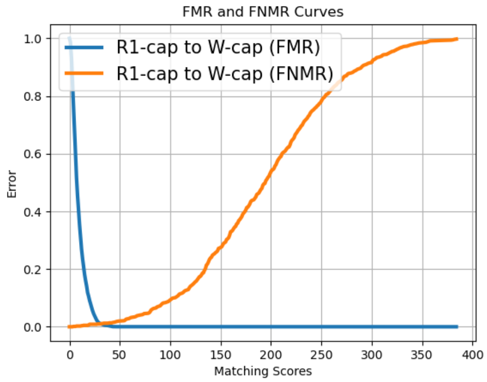


(d) R1-cap to W-cap

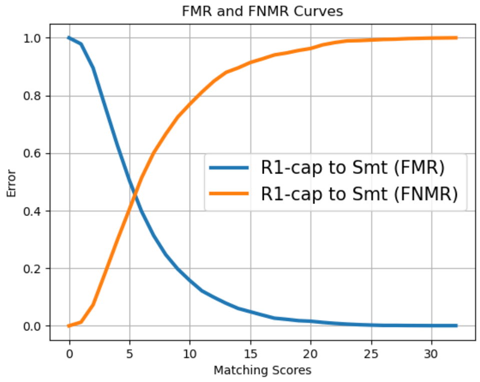


(e) R1-cap to Smt

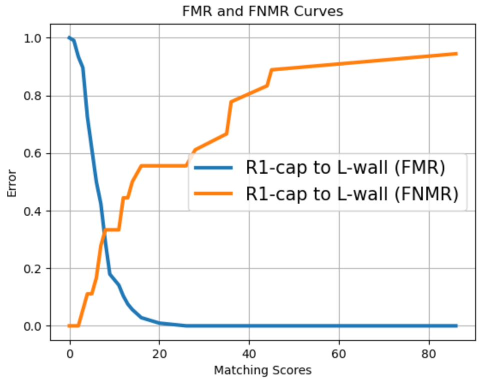


(f) R1-cap to L-wall

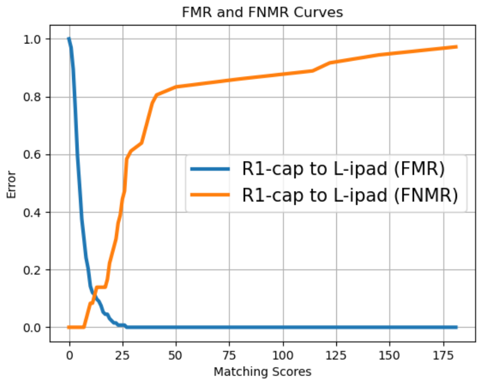


(g) R1-cap to L-ipad

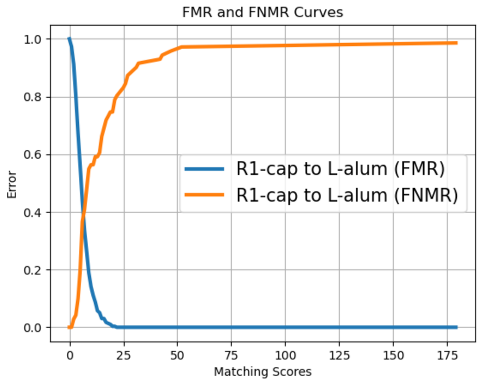


(h) R1-cap to L-alum

Fig. 43: FMR and FNMR curves of the VeriFinger (part 2/4) comparison scores in the 'Latent in the Wild' database

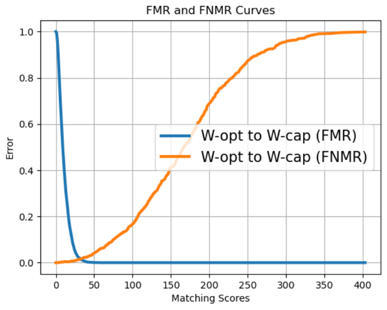


(a) W-opt to W-cap

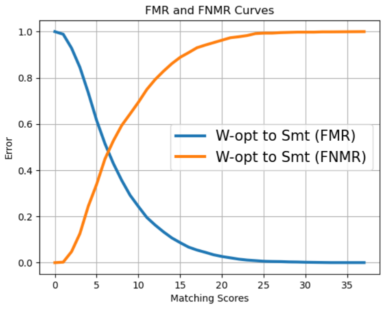


(b) W-opt to Smt

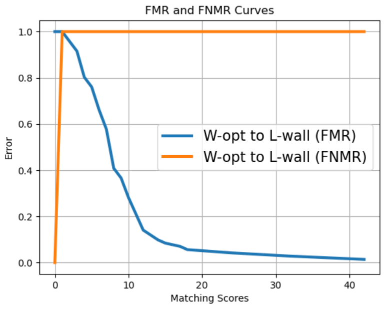


(c) W-opt to L-wall

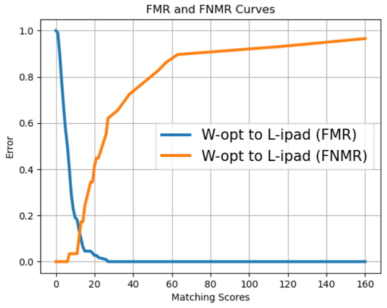


(d) W-opt to L-ipad

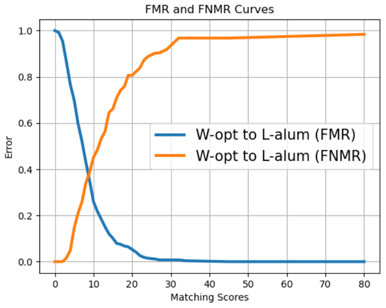


(e) W-opt to L-alum

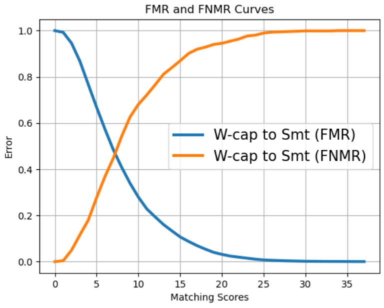


(f) W-cap to Smt

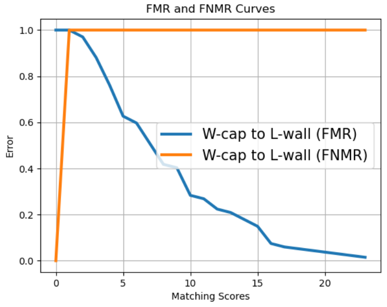


(g) W-cap to L-wall

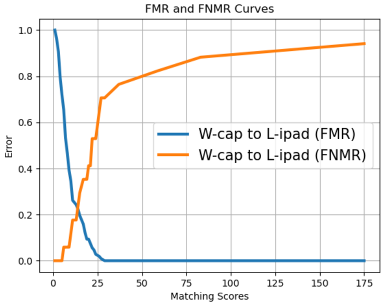


(h) W-cap to L-ipad

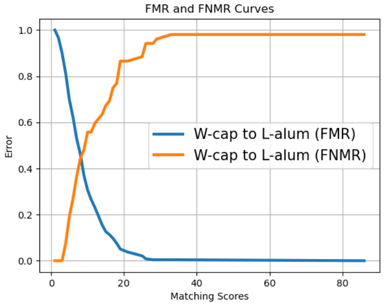


(i) W-cap to L-alum

Fig. 44: FMR and FNMR curves of the VeriFinger (part 3/4) comparison scores in the 'Latent in the Wild' database

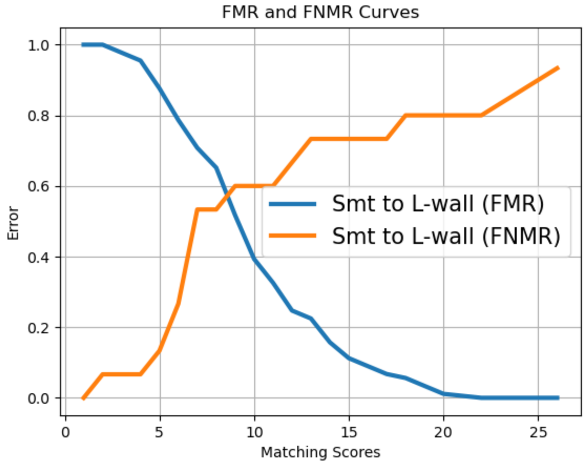


(a) Smt to L-wall

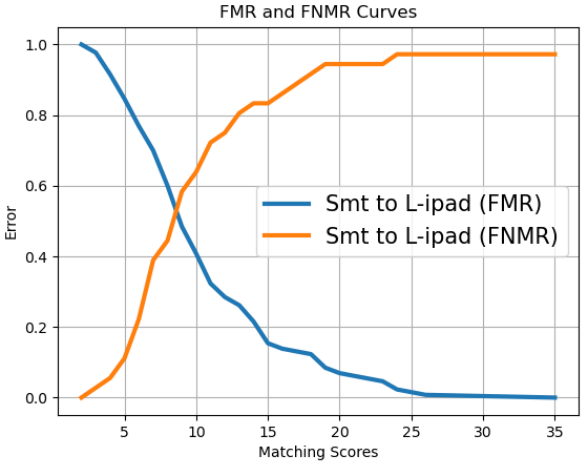


(b) Smt to L-ipad

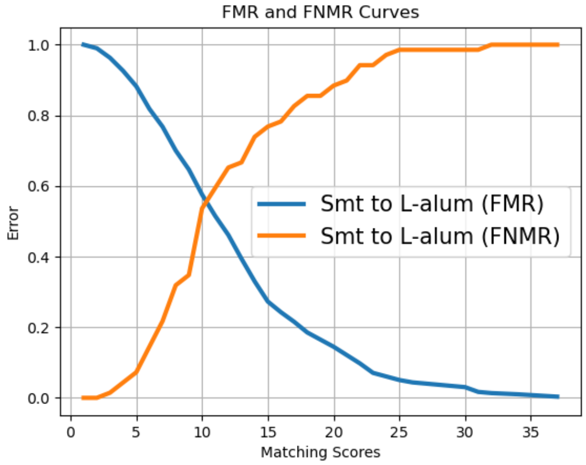


(c) Smt to L-alum

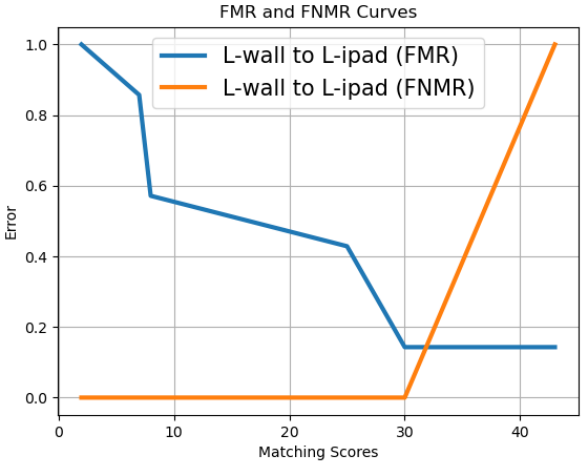


(d) L-wall to L-ipad

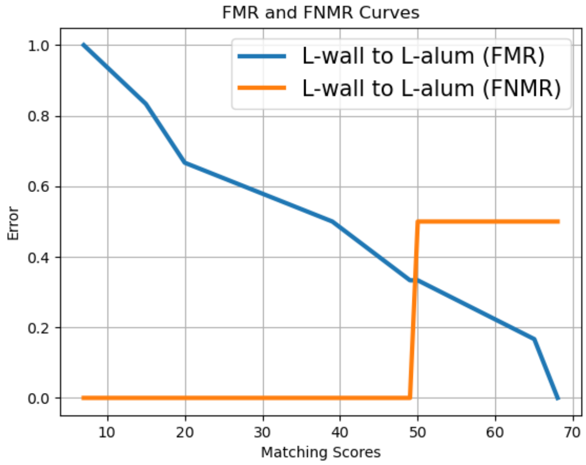


(e) L-wall to L-alum

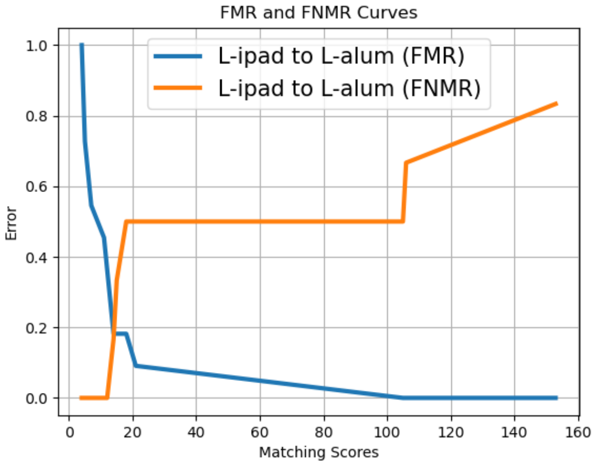


(f) L-ipad to L-alum

Fig. 45: FMR and FNMR curves of the VeriFinger (part 4/4) comparison scores in the 'Latent in the Wild' database

TABLE XXI: Performance indicators measured on the 'Latent in the Wild' database for the VeriFinger (part 1/4) comparison experiments.

| Comparison | GMean | GSTD | IMean | ISTD | SI | AUC | JI | JI_TH | MCC |
|---|---|---|---|---|---|---|---|---|---|
| R1-opt to R2-opt | 341.848 | 91.300 | 6.177 | 5.364 | 5.190 | 0.997 | 0.987 | 85.000 | 0.992 |
| R1-opt to R1-cap | 247.989 | 73.233 | 6.264 | 5.527 | 4.655 | 0.998 | 0.990 | 39.000 | 0.994 |
| R1-opt to R2-cap | 259.413 | 75.449 | 6.051 | 5.402 | 4.737 | 0.997 | 0.987 | 49.000 | 0.992 |
| R1-opt to W-opt | 214.817 | 81.119 | 7.306 | 5.872 | 3.608 | 0.997 | 0.980 | 42.000 | 0.987 |
| R1-opt to W-cap | 189.911 | 68.021 | 7.220 | 5.823 | 3.784 | 0.996 | 0.979 | 37.000 | 0.986 |
| R1-opt to Smt | 5.574 | 4.696 | 4.513 | 3.699 | 0.251 | 0.561 | 0.104 | 6.000 | 0.094 |
| R1-opt to L-wall | 23.053 | 22.402 | 5.255 | 4.615 | 1.100 | 0.838 | 0.503 | 9.000 | 0.572 |
| R1-opt to L-ipad | 42.694 | 42.220 | 4.669 | 3.932 | 1.268 | 0.971 | 0.839 | 12.000 | 0.814 |
| R1-opt to L-alum | 16.311 | 25.294 | 5.176 | 4.312 | 0.614 | 0.768 | 0.412 | 7.000 | 0.438 |
| | | | | | | | | | |
| Comparison | MCC_TH | EERL | EERH | EER | 0FMR | FMR1000 | FMR100 | FMR20 | FMR10 |
| R1-opt to R2-opt | 85.000 | 0.011 | 0.012 | 0.012 | 0.013 | 0.013 | 0.012 | 0.010 | 0.008 |
| R1-opt to R1-cap | 51.000 | 0.007 | 0.009 | 0.008 | 0.010 | 0.009 | 0.009 | 0.006 | 0.005 |
| R1-opt to R2-cap | 49.000 | 0.009 | 0.010 | 0.010 | 0.013 | 0.013 | 0.010 | 0.010 | 0.010 |
| R1-opt to W-opt | 42.000 | 0.013 | 0.015 | 0.014 | 0.022 | 0.019 | 0.016 | 0.009 | 0.007 |
| R1-opt to W-cap | 40.000 | 0.016 | 0.018 | 0.017 | 0.025 | 0.020 | 0.018 | 0.013 | 0.011 |
| R1-opt to Smt | 12.000 | 0.386 | 0.535 | 0.460 | 1.000 | 0.999 | 0.972 | 0.892 | 0.851 |
| R1-opt to L-wall | 26.000 | 0.263 | 0.287 | 0.275 | 0.632 | 0.632 | 0.579 | 0.526 | 0.474 |
| R1-opt to L-ipad | 12.000 | 0.094 | 0.111 | 0.102 | 0.306 | 0.306 | 0.306 | 0.111 | 0.111 |
| R1-opt to L-alum | 22.000 | 0.264 | 0.324 | 0.294 | 0.851 | 0.851 | 0.730 | 0.649 | 0.568 |
| | | | | | | | | | |
| Comparison | 0FNMR | EER_TH | 0FMR_TH | FMR1000_TH | FMR100_TH | FMR20_TH | FMR10_TH | 0FNMR_TH | |
| R1-opt to R2-opt | 0.644 | 25.000 | 85.000 | 40.000 | 26.000 | 18.000 | 13.000 | 4.000 | |
| R1-opt to R1-cap | 0.755 | 28.000 | 51.000 | 38.000 | 27.000 | 18.000 | 14.000 | 3.000 | |
| R1-opt to R2-cap | 0.616 | 26.000 | 49.000 | 41.000 | 26.000 | 18.000 | 13.000 | 4.000 | |
| R1-opt to W-opt | 0.924 | 26.000 | 51.000 | 41.000 | 29.000 | 20.000 | 16.000 | 2.000 | |
| R1-opt to W-cap | 0.613 | 26.000 | 47.000 | 35.000 | 28.000 | 20.000 | 16.000 | 5.000 | |
| R1-opt to Smt | 1.000 | 5.000 | 30.000 | 27.000 | 19.000 | 12.000 | 10.000 | 0.000 | |
| R1-opt to L-wall | 0.681 | 7.000 | 26.000 | 26.000 | 22.000 | 16.000 | 11.000 | 3.000 | |
| R1-opt to L-ipad | 0.324 | 10.000 | 25.000 | 25.000 | 24.000 | 12.000 | 10.000 | 6.000 | |
| R1-opt to L-alum | 0.962 | 7.000 | 27.000 | 27.000 | 21.000 | 15.000 | 12.000 | 1.000 | |

*Note:* ***GMean:*** *Genuine scores distribution mean;* ***GSTD:*** *Genuine scores distribution standard deviation;* ***IMean:*** *Impostor scores distribution mean;* ***ISTD:*** *Impostor scores distribution standard deviation;* ***AUC:*** *Area under the ROC curve;* ***SI:*** *Sensitivity Index;* ***JI:*** *Youden's J Index;* ***TH:*** *THreshold;* ***MCC:*** *Matthews Correlation Coefficient;* ***EER:*** *Equal Error Rate;* ***EERL:*** *EER low;* ***EERH:*** *EER high.*

TABLE XXII: Performance indicators measured on the 'Latent in the Wild' database for the VeriFinger (part 2/4) comparison experiments.

| Comparison | GMean | GSTD | IMean | ISTD | SI | AUC | JI | JI_TH | MCC |
|---|---|---|---|---|---|---|---|---|---|
| R1-cap to R2-cap | 281.227 | 85.241 | 6.930 | 6.141 | 4.539 | 1.000 | 0.997 | 48.000 | 0.998 |
| R1-cap to R2-opt | 247.232 | 72.208 | 6.205 | 5.452 | 4.707 | 0.999 | 0.995 | 53.000 | 0.997 |
| R1-cap to W-opt | 186.701 | 74.574 | 8.054 | 6.350 | 3.376 | 0.998 | 0.989 | 33.000 | 0.989 |
| R1-cap to W-cap | 193.782 | 71.234 | 8.805 | 6.978 | 3.655 | 0.997 | 0.986 | 42.000 | 0.990 |
| R1-cap to Smt | 6.755 | 5.089 | 5.649 | 4.332 | 0.234 | 0.563 | 0.090 | 5.000 | 0.077 |
| R1-cap to L-wall | 22.944 | 20.887 | 6.189 | 3.729 | 1.117 | 0.782 | 0.525 | 11.000 | 0.637 |
| R1-cap to L-ipad | 39.194 | 39.096 | 5.722 | 4.767 | 1.202 | 0.968 | 0.816 | 17.000 | 0.808 |
| R1-cap to L-alum | 15.183 | 22.617 | 5.700 | 3.824 | 0.585 | 0.711 | 0.351 | 13.000 | 0.446 |
| | | | | | | | | | |
| Comparison | MCC_TH | EERL | EERH | EER | 0FMR | FMR1000 | FMR100 | FMR20 | FMR10 |
| R1-cap to R2-cap | 48.000 | 0.002 | 0.003 | 0.002 | 0.003 | 0.003 | 0.002 | 0.002 | 0.002 |
| R1-cap to R2-opt | 53.000 | 0.004 | 0.005 | 0.005 | 0.005 | 0.005 | 0.005 | 0.004 | 0.004 |
| R1-cap to W-opt | 35.000 | 0.005 | 0.007 | 0.006 | 0.030 | 0.015 | 0.007 | 0.004 | 0.004 |
| R1-cap to W-cap | 45.000 | 0.009 | 0.011 | 0.010 | 0.021 | 0.014 | 0.010 | 0.009 | 0.006 |
| R1-cap to Smt | 8.000 | 0.405 | 0.505 | 0.455 | 0.999 | 0.997 | 0.983 | 0.914 | 0.850 |
| R1-cap to L-wall | 26.000 | 0.292 | 0.333 | 0.313 | 0.556 | 0.556 | 0.556 | 0.500 | 0.444 |
| R1-cap to L-ipad | 17.000 | 0.111 | 0.113 | 0.112 | 0.583 | 0.583 | 0.361 | 0.139 | 0.139 |
| R1-cap to L-alum | 20.000 | 0.337 | 0.408 | 0.373 | 0.803 | 0.803 | 0.746 | 0.606 | 0.563 |
| | | | | | | | | | |
| Comparison | 0FNMR | EER_TH | 0FMR_TH | FMR1000_TH | FMR100_TH | FMR20_TH | FMR10_TH | 0FNMR_TH | |
| R1-cap to R2-cap | 0.238 | 37.000 | 48.000 | 40.000 | 30.000 | 20.000 | 15.000 | 10.000 | |
| R1-cap to R2-opt | 0.284 | 30.000 | 53.000 | 36.000 | 27.000 | 18.000 | 14.000 | 8.000 | |
| R1-cap to W-opt | 0.926 | 31.000 | 50.000 | 40.000 | 29.000 | 22.000 | 18.000 | 2.000 | |
| R1-cap to W-cap | 0.848 | 32.000 | 54.000 | 42.000 | 31.000 | 24.000 | 19.000 | 3.000 | |
| R1-cap to Smt | 1.000 | 5.000 | 30.000 | 28.000 | 22.000 | 15.000 | 12.000 | 0.000 | |
| R1-cap to L-wall | 0.934 | 8.000 | 26.000 | 26.000 | 20.000 | 14.000 | 12.000 | 2.000 | |
| R1-cap to L-ipad | 0.308 | 12.000 | 27.000 | 27.000 | 23.000 | 16.000 | 13.000 | 7.000 | |
| R1-cap to L-alum | 0.973 | 7.000 | 22.000 | 22.000 | 19.000 | 14.000 | 11.000 | 1.000 | |

*Note:* ***GMean:*** *Genuine scores distribution mean;* ***GSTD:*** *Genuine scores distribution standard deviation;* ***IMean:*** *Impostor scores distribution mean;* ***ISTD:*** *Impostor scores distribution standard deviation;* ***AUC:*** *Area under the ROC curve;* ***SI:*** *Sensitivity Index;* ***JI:*** *Youden's J Index;* ***TH:*** *THreshold;* ***MCC:*** *Matthews Correlation Coefficient;* ***EER:*** *Equal Error Rate;* ***EERL:*** *EER low;* ***EERH:*** *EER high.*

TABLE XXIII: Performance indicators measured on the 'Latent in the Wild' database for the VeriFinger (part 3/4) comparison experiments.

| Comparison | GMean | GSTD | IMean | ISTD | SI | AUC | JI | JI_TH | MCC |
|---|---|---|---|---|---|---|---|---|---|
| W-opt to W-cap | 168.520 | 71.581 | 10.326 | 7.458 | 3.109 | 0.997 | 0.973 | 41.000 | 0.978 |
| W-opt to Smt | 7.616 | 5.288 | 6.943 | 4.980 | 0.131 | 0.536 | 0.064 | 9.000 | 0.056 |
| W-opt to L-wall | 0.000 | 0.000 | 8.183 | 6.471 | 1.789 | 0.000 | 0.000 | 0.000 | 0.000 |
| W-opt to L-ipad | 33.138 | 32.271 | 6.336 | 4.787 | 1.162 | 0.952 | 0.784 | 11.000 | 0.746 |
| W-opt to L-alum | 13.597 | 11.870 | 7.729 | 5.471 | 0.635 | 0.692 | 0.298 | 11.000 | 0.277 |
| W-cap to Smt | 8.224 | 5.490 | 7.528 | 5.180 | 0.130 | 0.539 | 0.068 | 7.000 | 0.052 |
| W-cap to L-wall | 0.000 | 0.000 | 7.701 | 4.969 | 2.192 | 0.000 | 0.000 | 0.000 | 0.000 |
| W-cap to L-ipad | 34.353 | 39.860 | 8.832 | 6.224 | 0.895 | 0.867 | 0.581 | 13.000 | 0.535 |
| W-cap to L-alum | 12.500 | 12.497 | 8.168 | 5.498 | 0.449 | 0.621 | 0.210 | 14.000 | 0.210 |
| | | | | | | | | | |
| Comparison | MCC_TH | EERL | EERH | EER | 0FMR | FMR1000 | FMR100 | FMR20 | FMR10 |
| W-opt to W-cap | 41.000 | 0.013 | 0.016 | 0.015 | 0.058 | 0.038 | 0.020 | 0.008 | 0.007 |
| W-opt to Smt | 10.000 | 0.429 | 0.527 | 0.478 | 0.999 | 0.998 | 0.983 | 0.930 | 0.862 |
| W-opt to L-wall | 0.000 | 1.000 | 1.000 | 1.000 | 1.000 | 1.000 | 1.000 | 1.000 | 1.000 |
| W-opt to L-ipad | 14.000 | 0.103 | 0.136 | 0.120 | 0.621 | 0.621 | 0.552 | 0.241 | 0.172 |
| W-opt to L-alum | 13.000 | 0.350 | 0.387 | 0.368 | 0.968 | 0.968 | 0.903 | 0.806 | 0.661 |
| W-cap to Smt | 7.000 | 0.448 | 0.484 | 0.466 | 1.000 | 0.999 | 0.980 | 0.928 | 0.870 |
| W-cap to L-wall | 0.000 | 1.000 | 1.000 | 1.000 | 1.000 | 1.000 | 1.000 | 1.000 | 1.000 |
| W-cap to L-ipad | 24.000 | 0.176 | 0.243 | 0.210 | 0.706 | 0.706 | 0.706 | 0.529 | 0.353 |
| W-cap to L-alum | 16.000 | 0.370 | 0.481 | 0.425 | 0.981 | 0.981 | 0.942 | 0.865 | 0.750 |
| | | | | | | | | | |
| Comparison | 0FNMR | EER_TH | 0FMR_TH | FMR1000_TH | FMR100_TH | FMR20_TH | FMR10_TH | 0FNMR_TH | |
| W-opt to W-cap | 0.907 | 33.000 | 57.000 | 48.000 | 35.000 | 25.000 | 21.000 | 3.000 | |
| W-opt to Smt | 1.000 | 7.000 | 33.000 | 31.000 | 23.000 | 17.000 | 14.000 | 0.000 | |
| W-opt to L-wall | 1.000 | 1.000 | 42.000 | 42.000 | 42.000 | 18.000 | 14.000 | 0.000 | |
| W-opt to L-ipad | 0.500 | 12.000 | 27.000 | 27.000 | 26.000 | 15.000 | 13.000 | 6.000 | |
| W-opt to L-alum | 0.955 | 9.000 | 45.000 | 45.000 | 26.000 | 20.000 | 15.000 | 2.000 | |
| W-cap to Smt | 1.000 | 7.000 | 37.000 | 33.000 | 24.000 | 18.000 | 15.000 | 0.000 | |
| W-cap to L-wall | 1.000 | 1.000 | 23.000 | 23.000 | 23.000 | 17.000 | 16.000 | 0.000 | |
| W-cap to L-ipad | 0.720 | 13.000 | 29.000 | 29.000 | 27.000 | 23.000 | 19.000 | 5.000 | |
| W-cap to L-alum | 0.899 | 9.000 | 86.000 | 86.000 | 26.000 | 19.000 | 17.000 | 3.000 | |

*Note: **GMean:** Genuine scores distribution mean; **GSTD:** Genuine scores distribution standard deviation; **IMean:** Impostor scores distribution mean; **ISTD:** Impostor scores distribution standard deviation; **AUC:** Area under the ROC curve; **SI:** Sensitivity Index; **JI:** Youden's J Index; **TH:** THreshold; **MCC:** Matthews Correlation Coefficient; **EER:** Equal Error Rate; **EERL:** EER low; **EERH:** EER high.*

TABLE XXIV: Performance indicators measured on the 'Latent in the Wild' database for the VeriFinger (part 4/4) comparison experiments.

| Comparison | GMean | GSTD | IMean | ISTD | SI | AUC | JI | JI_TH | MCC |
|---|---|---|---|---|---|---|---|---|---|
| Smt to L-wall | 10.467 | 7.437 | 9.191 | 4.146 | 0.212 | 0.484 | 0.200 | 22.000 | 0.420 |
| Smt to L-ipad | 9.528 | 6.234 | 9.685 | 5.415 | 0.027 | 0.473 | 0.043 | 5.000 | 0.148 |
| Smt to L-alum | 11.029 | 5.856 | 11.842 | 6.860 | 0.127 | 0.469 | 0.045 | 5.000 | 0.057 |
| L-wall to L-ipad | 30.000 | 0.000 | 16.714 | 13.677 | 1.374 | 0.857 | 0.857 | 30.000 | 0.655 |
| L-wall to L-alum | 58.500 | 9.500 | 32.667 | 20.483 | 1.618 | 0.833 | 0.667 | 49.000 | 0.655 |
| L-ipad to L-alum | 67.500 | 56.121 | 9.455 | 5.630 | 1.455 | 0.894 | 0.652 | 14.000 | 0.633 |
| | | | | | | | | | |
| Comparison | MCC_TH | EERL | EERH | EER | 0FMR | FMR1000 | FMR100 | FMR20 | FMR10 |
| Smt to L-wall | 22.000 | 0.517 | 0.600 | 0.558 | 0.800 | 0.800 | 0.800 | 0.800 | 0.733 |
| Smt to L-ipad | 35.000 | 0.444 | 0.600 | 0.522 | 0.972 | 0.972 | 0.972 | 0.944 | 0.944 |
| Smt to L-alum | 5.000 | 0.515 | 0.594 | 0.555 | 1.000 | 1.000 | 1.000 | 0.986 | 0.942 |
| L-wall to L-ipad | 30.000 | 0.000 | 0.143 | 0.071 | 0.000 | 0.000 | 0.000 | 0.000 | 0.000 |
| L-wall to L-alum | 68.000 | 0.000 | 0.333 | 0.167 | 0.500 | 0.500 | 0.500 | 0.500 | 0.500 |
| L-ipad to L-alum | 14.000 | 0.167 | 0.182 | 0.174 | 0.500 | 0.500 | 0.500 | 0.500 | 0.500 |
| | | | | | | | | | |
| Comparison | 0FNMR | EER_TH | 0FMR_TH | FMR1000_TH | FMR100_TH | FMR20_TH | FMR10_TH | 0FNMR_TH | |
| Smt to L-wall | 1.000 | 9.000 | 22.000 | 22.000 | 20.000 | 18.000 | 16.000 | 1.000 | |
| Smt to L-ipad | 1.000 | 8.000 | 35.000 | 35.000 | 26.000 | 22.000 | 19.000 | 2.000 | |
| Smt to L-alum | 0.990 | 11.000 | 37.000 | 37.000 | 34.000 | 25.000 | 22.000 | 2.000 | |
| L-wall to L-ipad | 0.143 | 30.000 | 30.000 | 30.000 | 30.000 | 30.000 | 30.000 | 30.000 | |
| L-wall to L-alum | 0.333 | 49.000 | 68.000 | 68.000 | 68.000 | 68.000 | 65.000 | 49.000 | |
| L-ipad to L-alum | 0.364 | 14.000 | 105.000 | 105.000 | 105.000 | 21.000 | 21.000 | 12.000 | |

*Note: **GMean:** Genuine scores distribution mean; **GSTD:** Genuine scores distribution standard deviation; **IMean:** Impostor scores distribution mean; **ISTD:** Impostor scores distribution standard deviation; **AUC:** Area under the ROC curve; **SI:** Sensitivity Index; **JI:** Youden's J Index; **TH:** THreshold; **MCC:** Matthews Correlation Coefficient; **EER:** Equal Error Rate; **EERL:** EER low; **EERH:** EER high.*

### *E. Supplementary results for the MinutiaeNet-MCC comparison experiment*

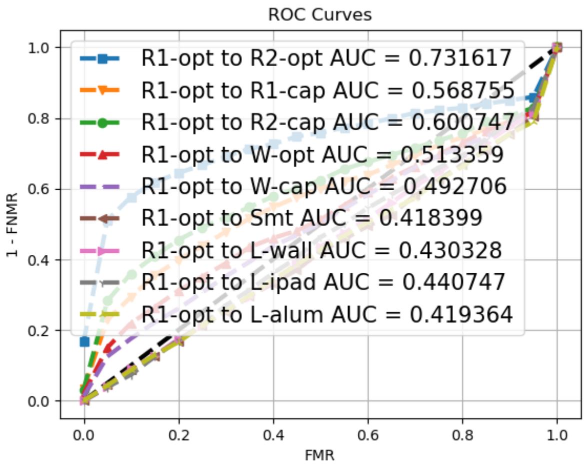


(a)

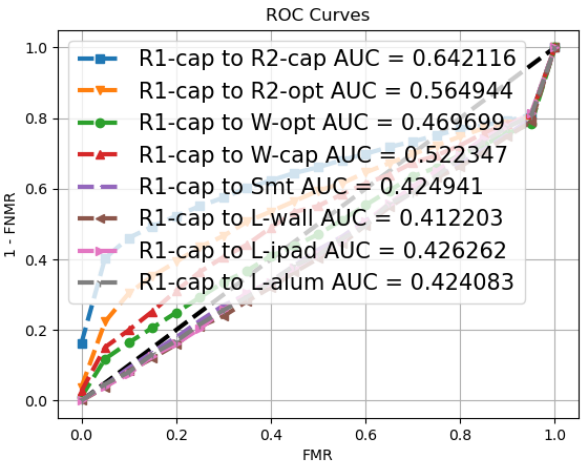


(b)

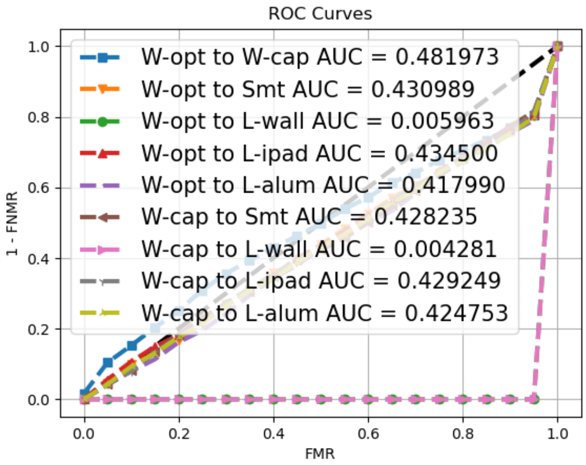


(c)

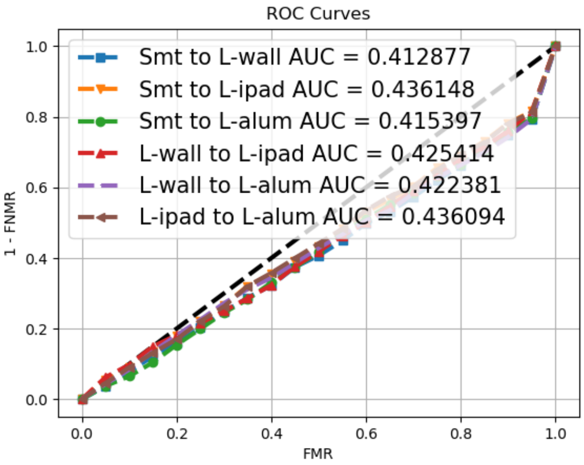


(d)

Fig. 46: ROC curve of the MinutiaeNet-MCC comparison experiments for the 'Latent in the Wild' database

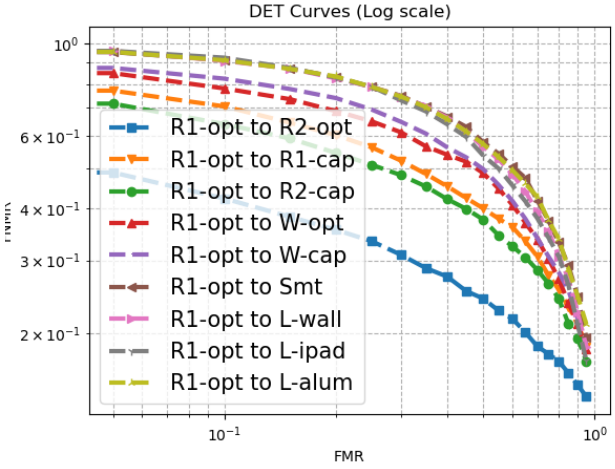


(a)

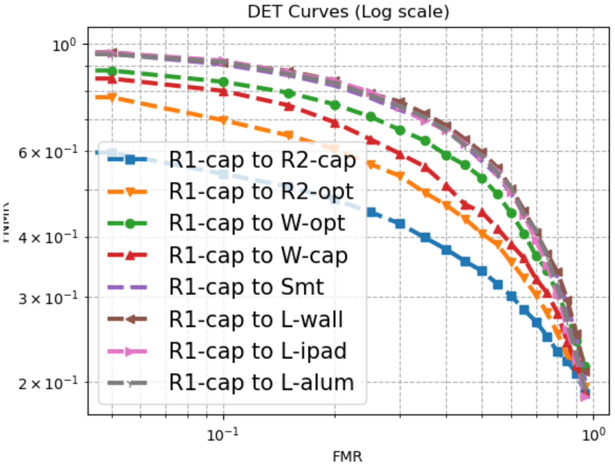


(b)

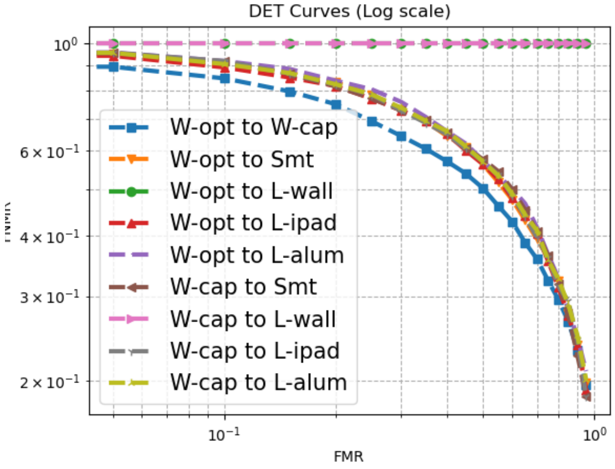


(c)

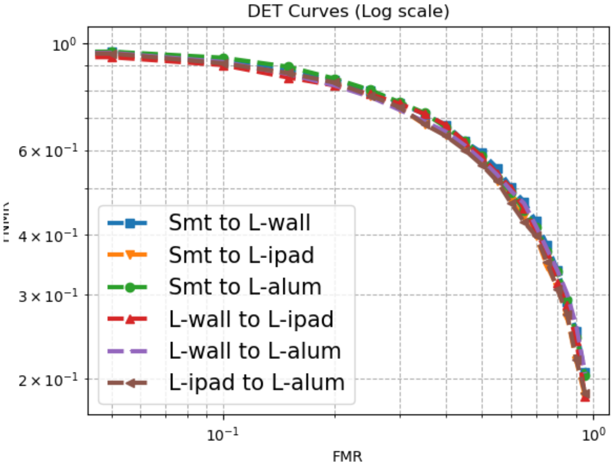


(d)

Fig. 47: DET curve of the MinutiaeNet-MCC comparison experiments for the 'Latent in the Wild' database

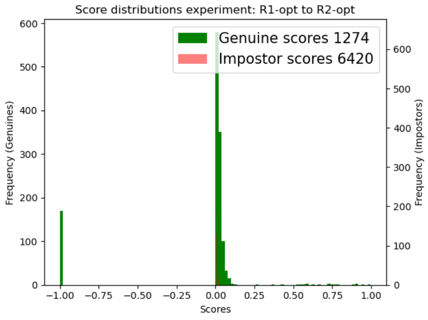


(a) R1-opt to R2-opt

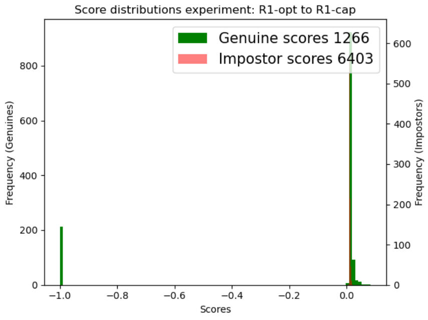


(b) R1-opt to R1-cap

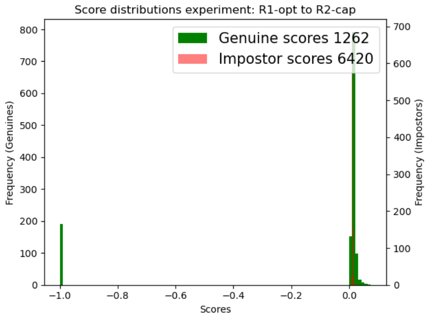


(c) R1-opt to R2-cap

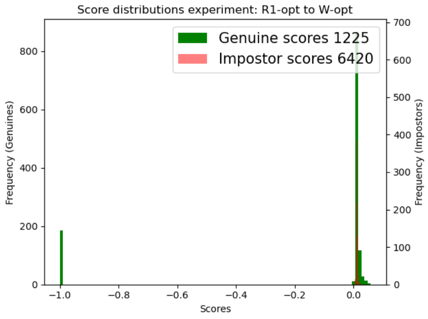


(d) R1-opt to W-opt

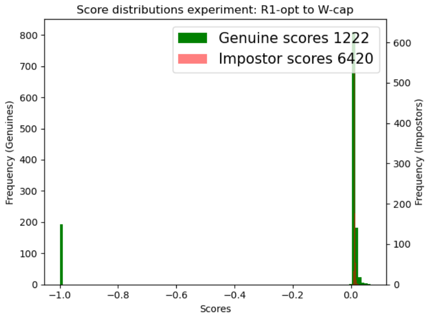


(e) R1-opt to W-cap

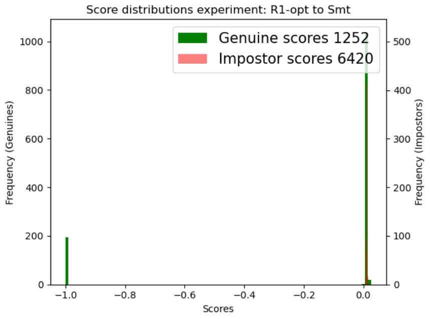


(f) R1-opt to Smt

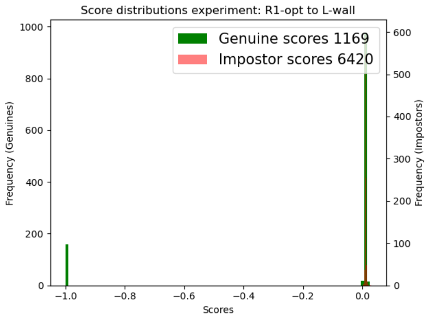


(g) R1-opt to L-wall

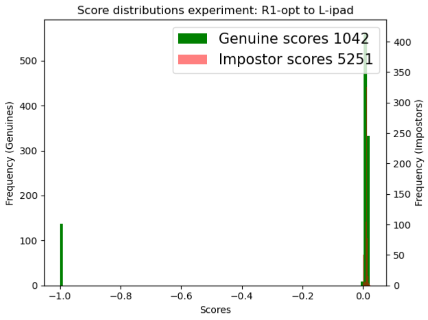


(h) R1-opt to L-ipad

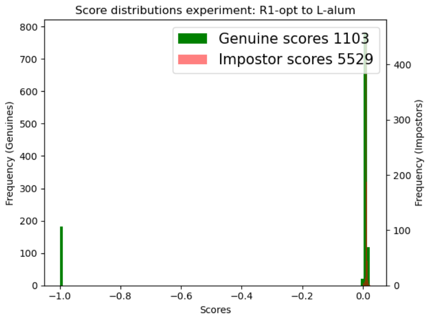


(i) R1-opt to L-alum

Fig. 48: Distributions of the MinutiaeNet-MCC (part 1/4) comparison scores in the 'Latent in the Wild' database

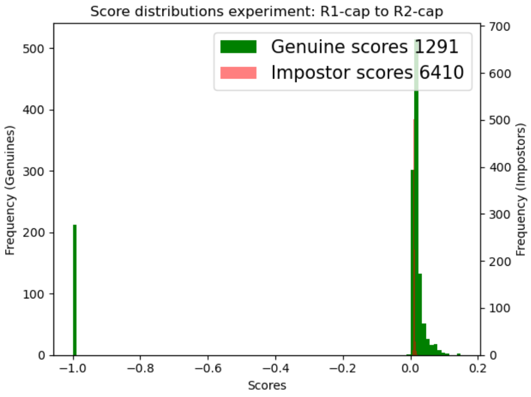


(a) R1-cap to R2-cap

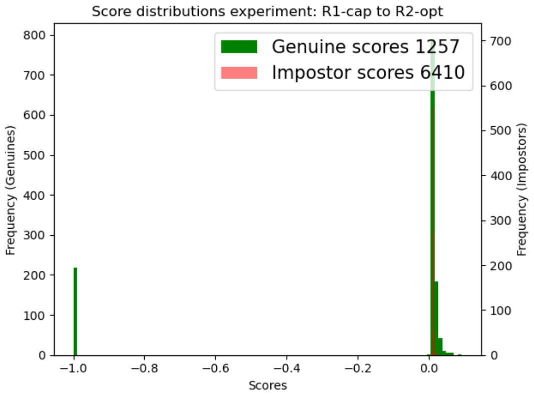


(b) R1-cap to R2-opt

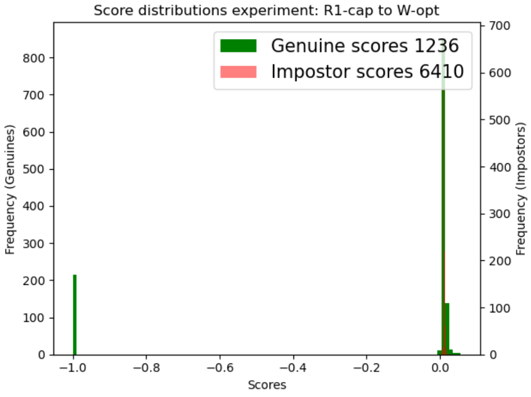


(c) R1-cap to W-opt

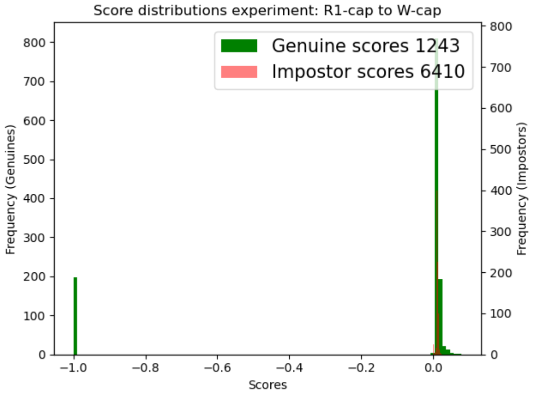


(d) R1-cap to W-cap

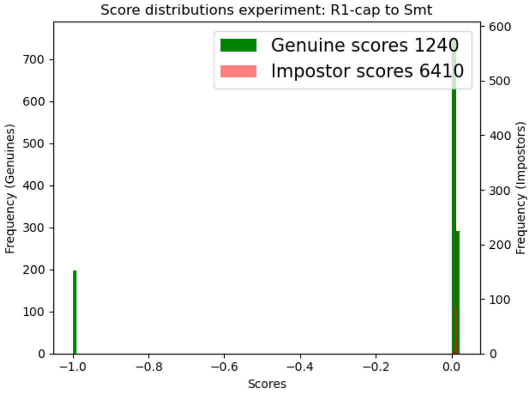


(e) R1-cap to Smt

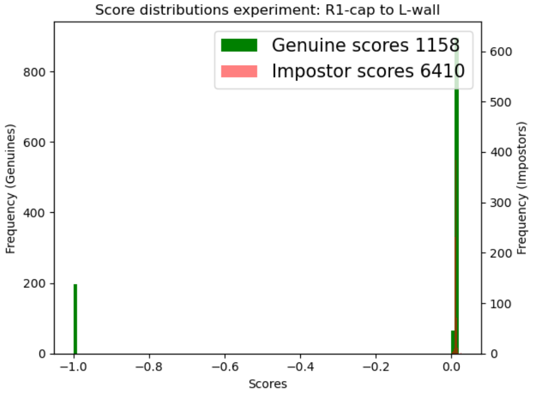


(f) R1-cap to L-wall

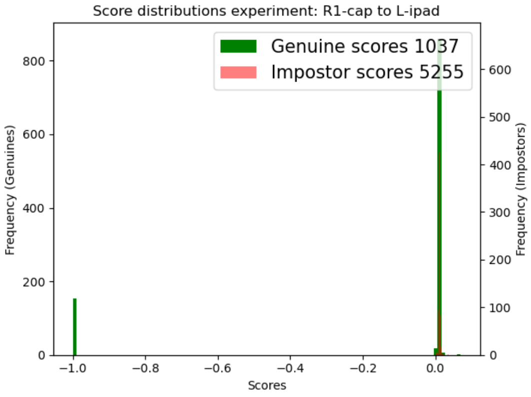


(g) R1-cap to L-ipad

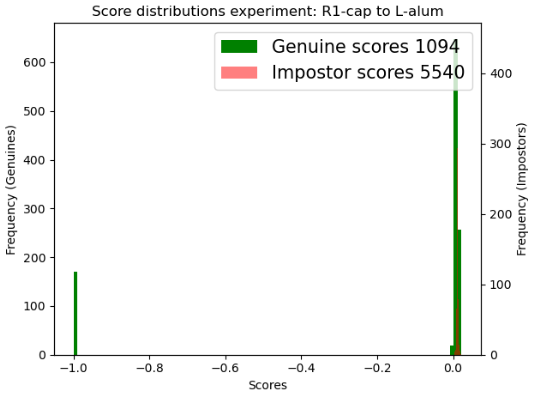


(h) R1-cap to L-alum

Fig. 49: Distributions of the MinutiaeNet-MCC (part 2/4) comparison scores in the 'Latent in the Wild' database

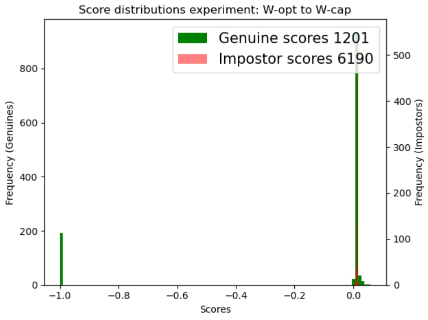


(a) W-opt to W-cap

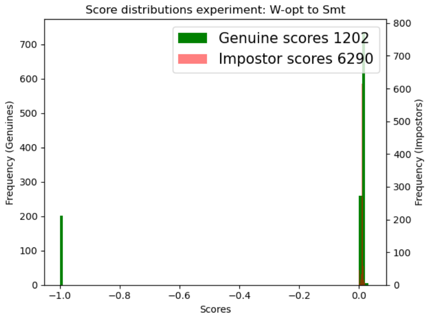


(b) W-opt to Smt

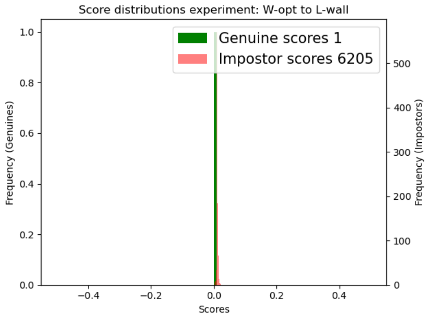


(c) W-opt to L-wall

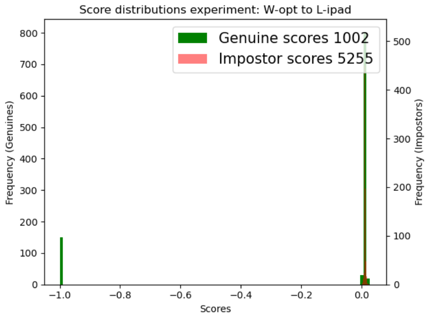


(d) W-opt to L-ipad

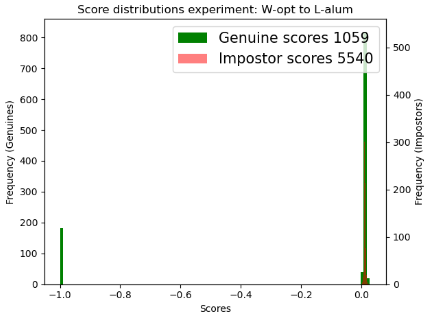


(e) W-opt to L-alum

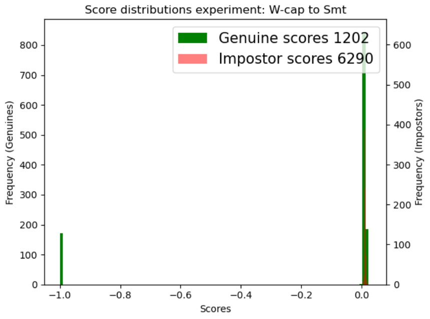


(f) W-cap to Smt

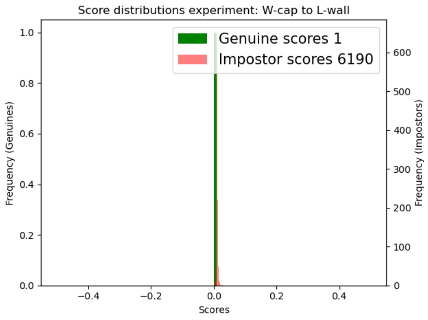


(g) W-cap to L-wall

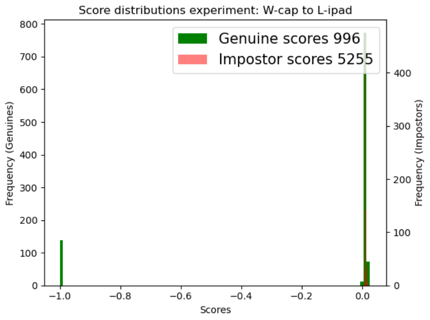


(h) W-cap to L-ipad

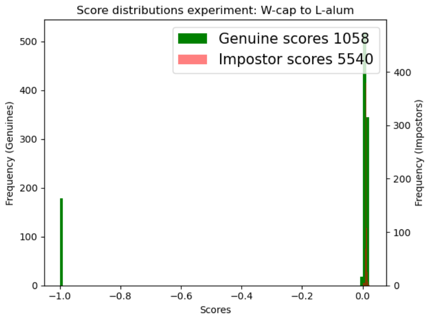


(i) W-cap to L-alum

Fig. 50: Distributions of the MinutiaeNet-MCC (part 3/4) comparison scores in the 'Latent in the Wild' database

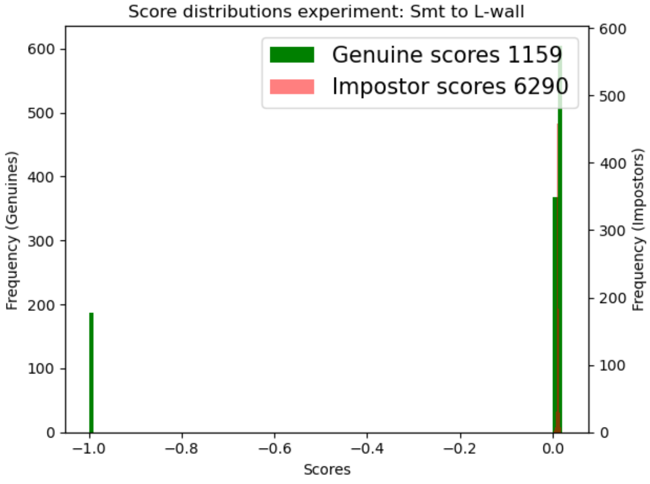


(a) Smt to L-wall

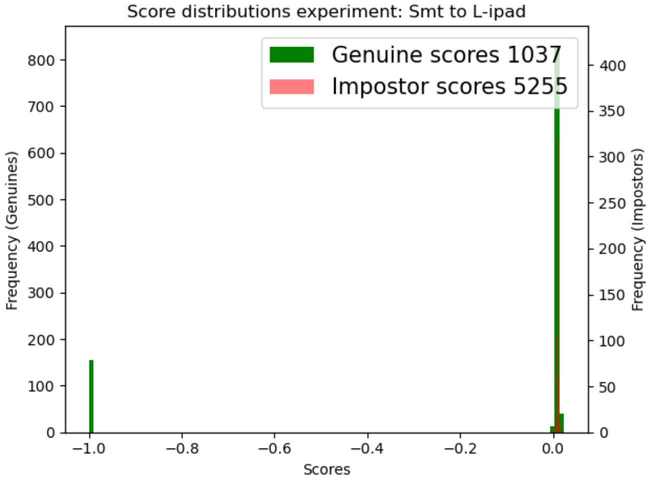


(b) Smt to L-ipad

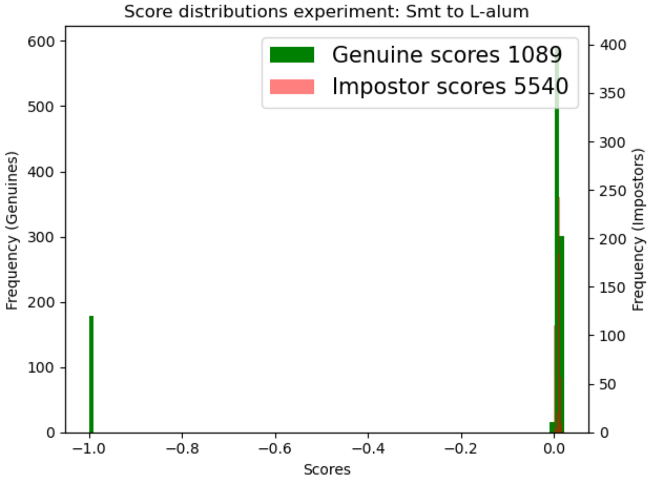


(c) Smt to L-alum

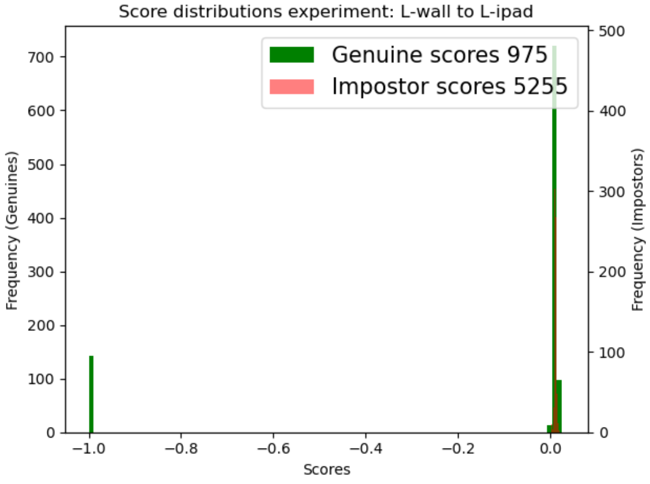


(d) L-wall to L-ipad

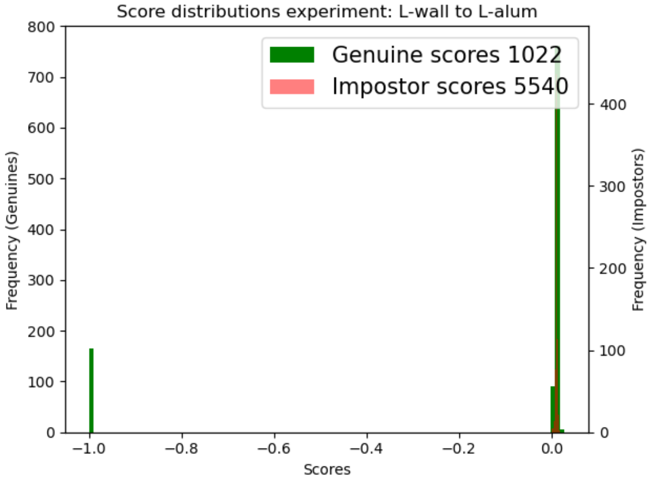


(e) L-wall to L-alum

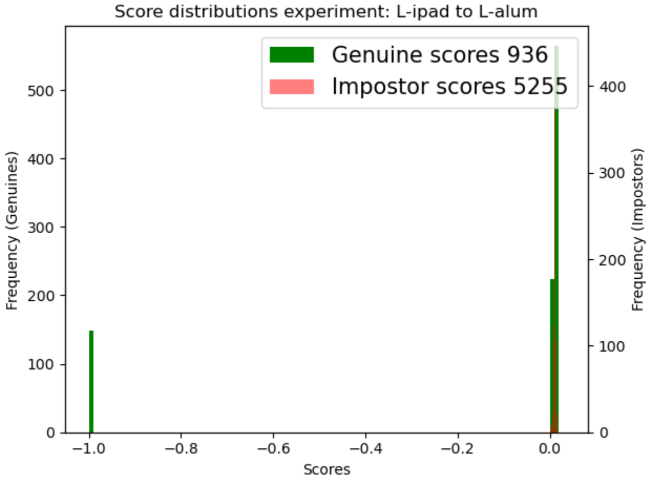


(f) L-ipad to L-alum

Fig. 51: Distributions of the MinutiaeNet-MCC (part 4/4) comparison scores in the 'Latent in the Wild' database

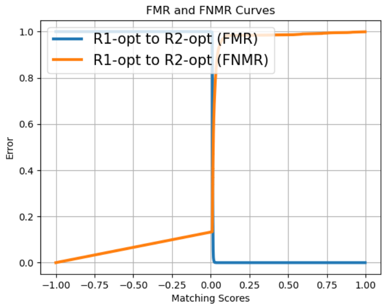


(a) R1-opt to R2-opt

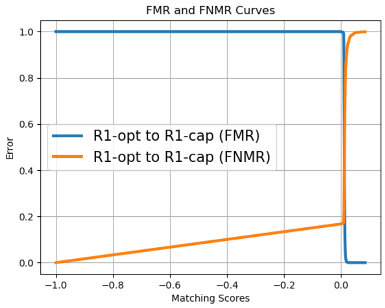


(b) R1-opt to R1-cap

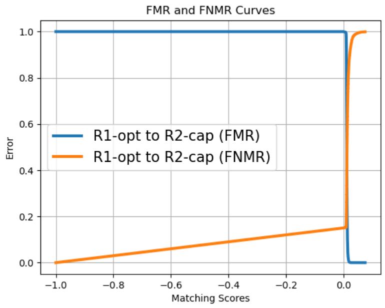


(c) R1-opt to R2-cap

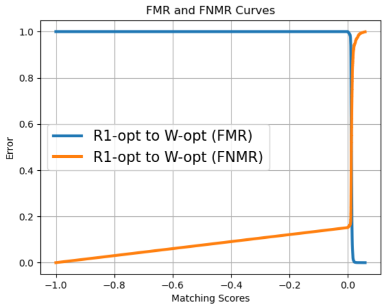


(d) R1-opt to W-opt

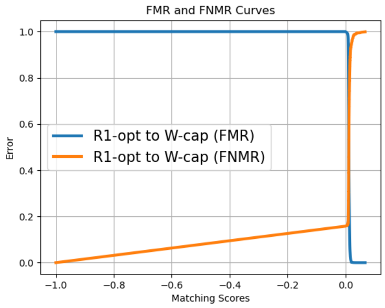


(e) R1-opt to W-cap

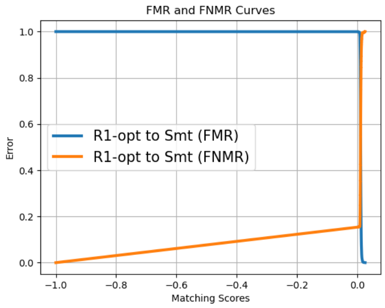


(f) R1-opt to Smt

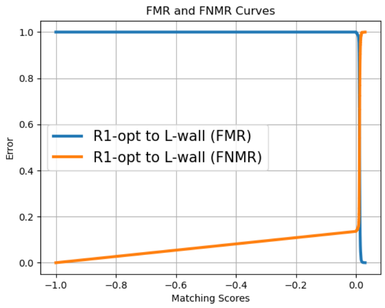


(g) R1-opt to L-wall

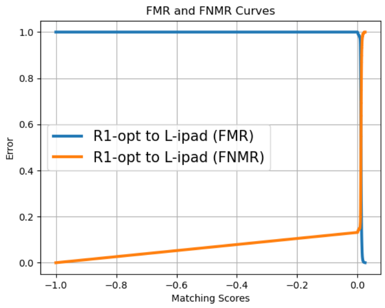


(h) R1-opt to L-ipad

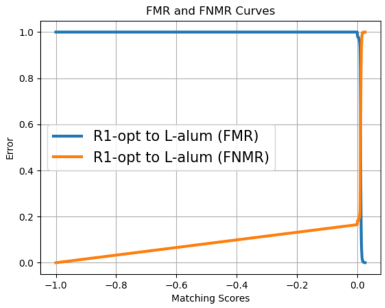


(i) R1-opt to L-alum

Fig. 52: FMR and FNMR curves of the MinutiaeNet-MCC (part 1/4) comparison scores in the 'Latent in the Wild' database

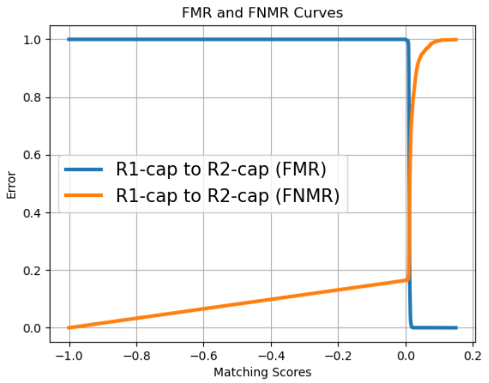


(a) R1-cap to R2-cap

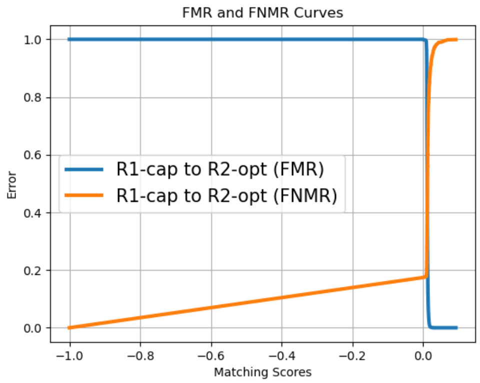


(b) R1-cap to R2-opt

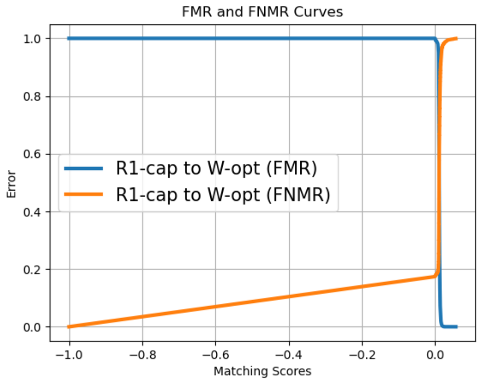


(c) R1-cap to W-opt

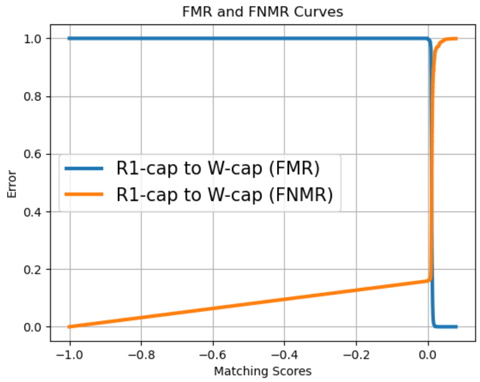


(d) R1-cap to W-cap

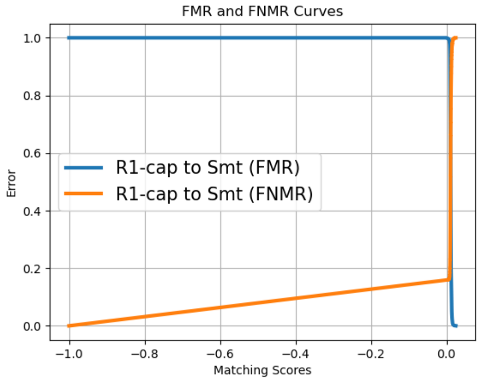


(e) R1-cap to Smt

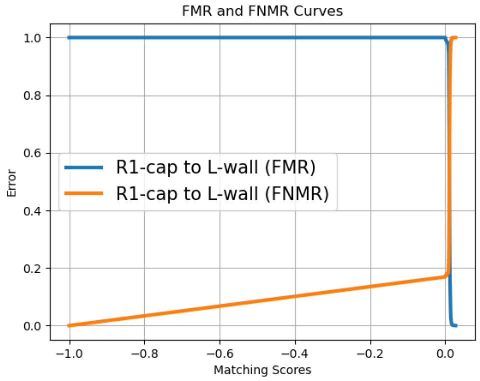


(f) R1-cap to L-wall

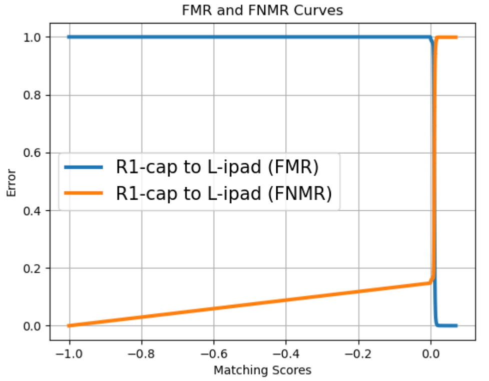


(g) R1-cap to L-ipad

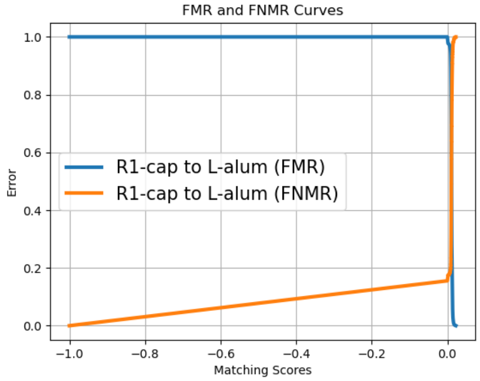


(h) R1-cap to L-alum

Fig. 53: FMR and FNMR curves of the MinutiaeNet-MCC (part 2/4) comparison scores in the 'Latent in the Wild' database

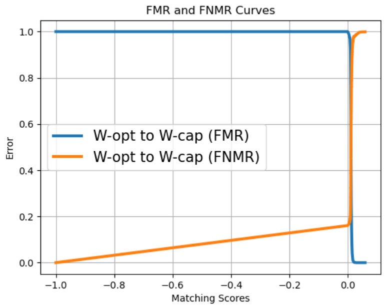


(a) W-opt to W-cap

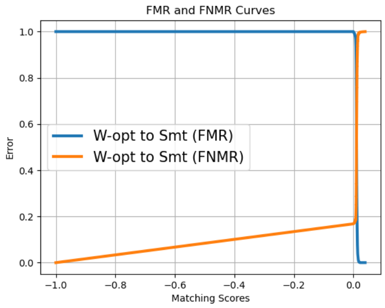


(b) W-opt to Smt

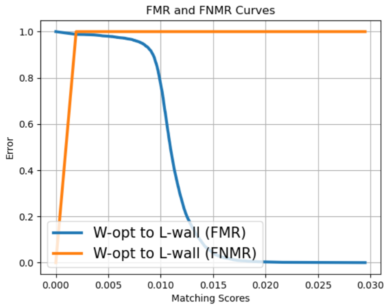


(c) W-opt to L-wall

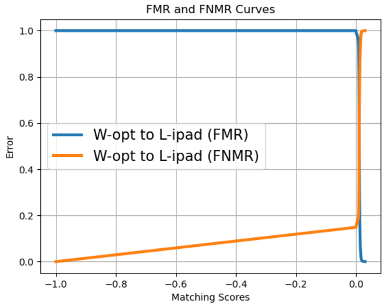


(d) W-opt to L-ipad

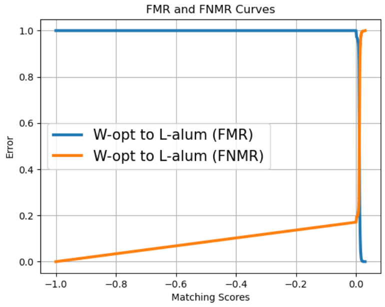


(e) W-opt to L-alum

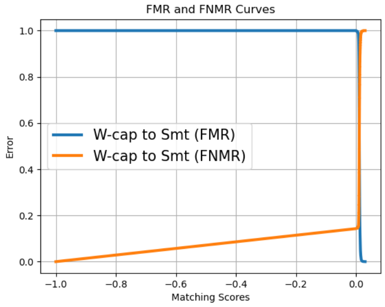


(f) W-cap to Smt

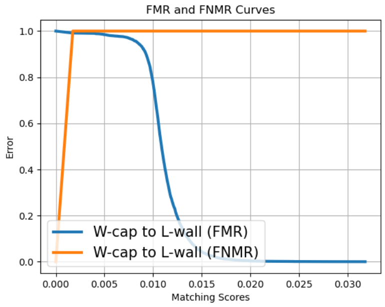


(g) W-cap to L-wall

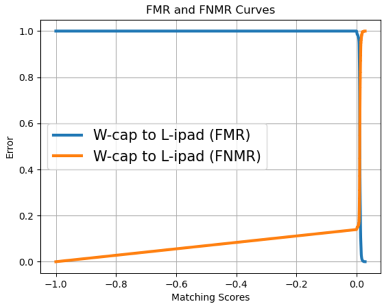


(h) W-cap to L-ipad

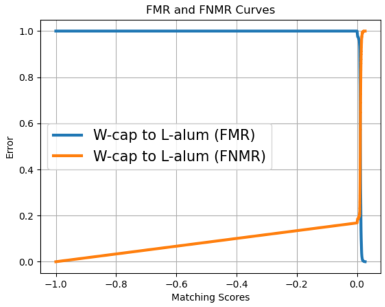


(i) W-cap to L-alum

Fig. 54: FMR and FNMR curves of the MinutiaeNet-MCC (part 3/4) comparison scores in the 'Latent in the Wild' database

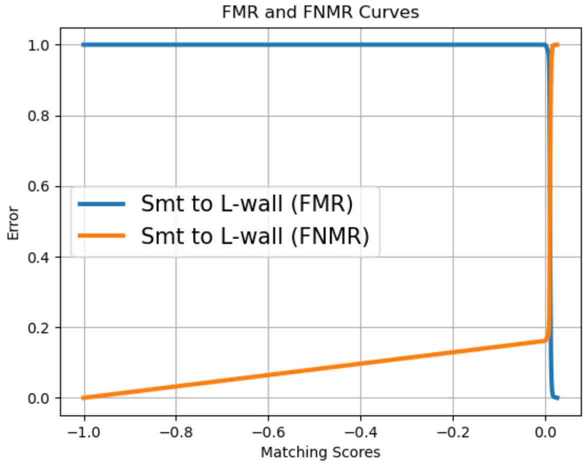


(a) Smt to L-wall

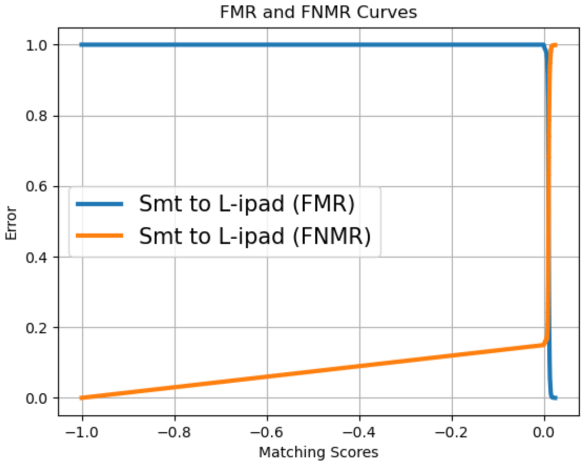


(b) Smt to L-ipad

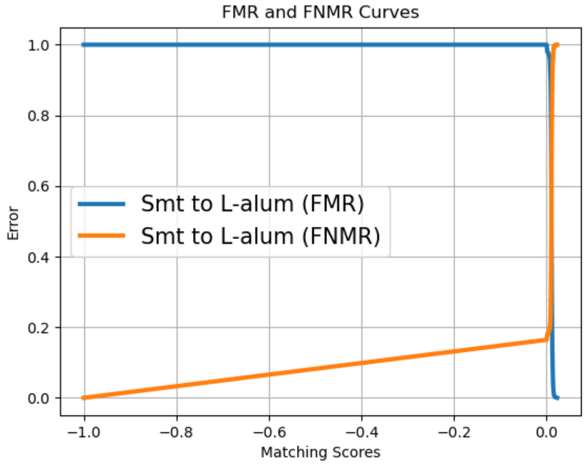


(c) Smt to L-alum

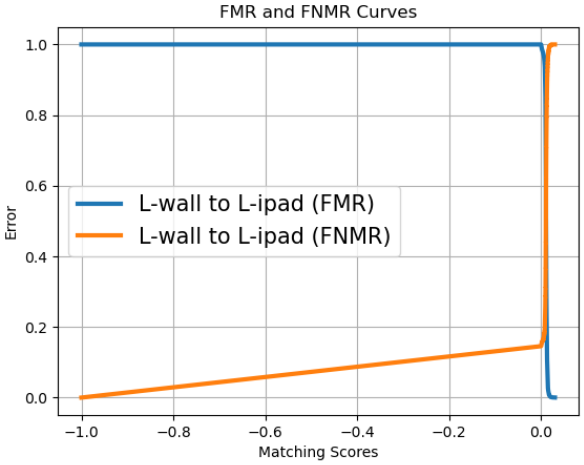


(d) L-wall to L-ipad

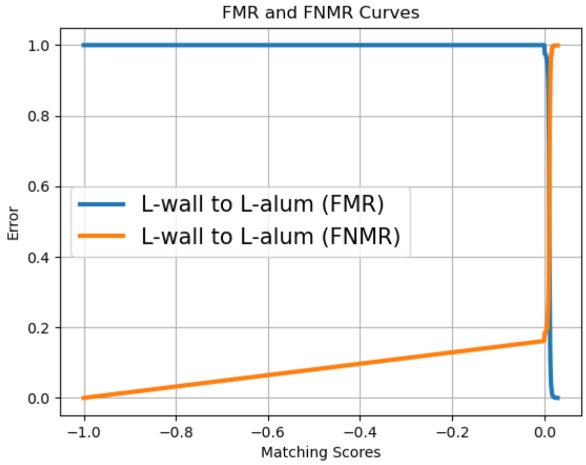


(e) L-wall to L-alum

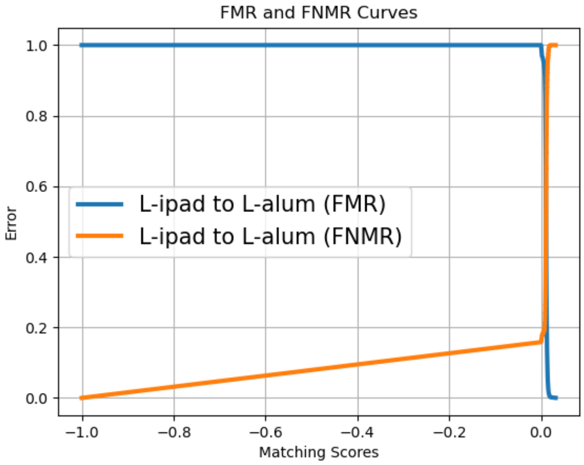


(f) L-ipad to L-alum

Fig. 55: FMR and FNMR curves of the MinutiaeNet-MCC (part 4/4) comparison scores in the 'Latent in the Wild' database

TABLE XXV: Performance indicators measured on the 'Latent in the Wild' database for the MinutiaeNet-MCC (part 1/4) comparison experiments.

| Comparison | GMean | GSTD | IMean | ISTD | SI | AUC | JI | JI_TH | MCC |
|---|---|---|---|---|---|---|---|---|---|
| R1-opt to R2-opt | -0.102 | 0.362 | 0.012 | 0.002 | 0.445 | 0.732 | 0.478 | 0.015 | 0.544 |
| R1-opt to R1-cap | -0.155 | 0.379 | 0.012 | 0.002 | 0.623 | 0.569 | 0.207 | 0.013 | 0.262 |
| R1-opt to R2-cap | -0.138 | 0.363 | 0.012 | 0.002 | 0.582 | 0.601 | 0.261 | 0.014 | 0.330 |
| R1-opt to W-opt | -0.140 | 0.364 | 0.012 | 0.002 | 0.590 | 0.513 | 0.127 | 0.014 | 0.192 |
| R1-opt to W-cap | -0.147 | 0.370 | 0.012 | 0.002 | 0.607 | 0.493 | 0.085 | 0.015 | 0.185 |
| R1-opt to Smt | -0.145 | 0.365 | 0.011 | 0.002 | 0.604 | 0.418 | 0.003 | 0.021 | 0.033 |
| R1-opt to L-wall | -0.126 | 0.347 | 0.011 | 0.002 | 0.561 | 0.430 | 0.001 | 0.018 | 0.006 |
| R1-opt to L-ipad | -0.122 | 0.342 | 0.011 | 0.002 | 0.550 | 0.441 | 0.004 | 0.020 | 0.024 |
| R1-opt to L-alum | -0.156 | 0.375 | 0.011 | 0.003 | 0.629 | 0.419 | 0.000 | 0.024 | 0.002 |
| | | | | | | | | | |
| Comparison | MCC_TH | EERL | EERH | EER | 0FMR | FMR1000 | FMR100 | FMR20 | FMR10 |
| R1-opt to R2-opt | 0.019 | 0.306 | 0.307 | 0.306 | 0.833 | 0.728 | 0.623 | 0.489 | 0.423 |
| R1-opt to R1-cap | 0.018 | 0.434 | 0.434 | 0.434 | 0.966 | 0.938 | 0.870 | 0.771 | 0.706 |
| R1-opt to R2-cap | 0.018 | 0.415 | 0.416 | 0.415 | 0.968 | 0.910 | 0.824 | 0.717 | 0.640 |
| R1-opt to W-opt | 0.024 | 0.491 | 0.491 | 0.491 | 0.980 | 0.958 | 0.922 | 0.850 | 0.780 |
| R1-opt to W-cap | 0.021 | 0.498 | 0.499 | 0.499 | 0.988 | 0.963 | 0.933 | 0.875 | 0.824 |
| R1-opt to Smt | 0.023 | 0.545 | 0.546 | 0.546 | 0.999 | 0.996 | 0.992 | 0.955 | 0.913 |
| R1-opt to L-wall | 0.027 | 0.537 | 0.538 | 0.537 | 1.000 | 0.999 | 0.991 | 0.962 | 0.909 |
| R1-opt to L-ipad | 0.020 | 0.519 | 0.519 | 0.519 | 1.000 | 1.000 | 0.989 | 0.962 | 0.926 |
| R1-opt to L-alum | 0.024 | 0.541 | 0.542 | 0.542 | 1.000 | 0.999 | 0.996 | 0.956 | 0.913 |
| | | | | | | | | | |
| Comparison | 0FNMR | EER_TH | 0FMR_TH | FMR1000_TH | FMR100_TH | FMR20_TH | FMR10_TH | 0FNMR_TH | |
| R1-opt to R2-opt | 1.000 | 0.013 | 0.034 | 0.026 | 0.020 | 0.016 | 0.015 | -1.000 | |
| R1-opt to R1-cap | 1.000 | 0.012 | 0.029 | 0.023 | 0.018 | 0.015 | 0.014 | -1.000 | |
| R1-opt to R2-cap | 1.000 | 0.012 | 0.031 | 0.022 | 0.018 | 0.015 | 0.014 | -1.000 | |
| R1-opt to W-opt | 1.000 | 0.012 | 0.034 | 0.026 | 0.019 | 0.016 | 0.015 | -1.000 | |
| R1-opt to W-cap | 1.000 | 0.012 | 0.033 | 0.023 | 0.019 | 0.016 | 0.014 | -1.000 | |
| R1-opt to Smt | 1.000 | 0.011 | 0.026 | 0.021 | 0.016 | 0.014 | 0.013 | -1.000 | |
| R1-opt to L-wall | 1.000 | 0.011 | 0.030 | 0.023 | 0.017 | 0.015 | 0.013 | -1.000 | |
| R1-opt to L-ipad | 1.000 | 0.011 | 0.025 | 0.023 | 0.018 | 0.015 | 0.014 | -1.000 | |
| R1-opt to L-alum | 1.000 | 0.011 | 0.026 | 0.023 | 0.018 | 0.015 | 0.014 | -1.000 | |

*Note:* ***GMean:*** *Genuine scores distribution mean;* ***GSTD:*** *Genuine scores distribution standard deviation;* ***IMean:*** *Impostor scores distribution mean;* ***ISTD:*** *Impostor scores distribution standard deviation;* ***AUC:*** *Area under the ROC curve;* ***SI:*** *Sensitivity Index;* ***JI:*** *Youden's J Index;* ***TH:*** *THreshold;* ***MCC:*** *Matthews Correlation Coefficient;* ***EER:*** *Equal Error Rate;* ***EERL:*** *EER low;* ***EERH:*** *EER high.*

TABLE XXVI: Performance indicators measured on the 'Latent in the Wild' database for the MinutiaeNet-MCC (part 2/4) comparison experiments.

| Comparison | GMean | GSTD | IMean | ISTD | SI | AUC | JI | JI_TH | MCC |
|---|---|---|---|---|---|---|---|---|---|
| R1-cap to R2-cap | -0.147 | 0.378 | 0.011 | 0.002 | 0.593 | 0.642 | 0.368 | 0.014 | 0.476 |
| R1-cap to R2-opt | -0.162 | 0.385 | 0.012 | 0.002 | 0.637 | 0.565 | 0.207 | 0.013 | 0.291 |
| R1-cap to W-opt | -0.164 | 0.384 | 0.011 | 0.002 | 0.645 | 0.470 | 0.072 | 0.014 | 0.129 |
| R1-cap to W-cap | -0.147 | 0.370 | 0.011 | 0.002 | 0.606 | 0.522 | 0.118 | 0.012 | 0.213 |
| R1-cap to Smt | -0.150 | 0.370 | 0.011 | 0.002 | 0.614 | 0.425 | 0.007 | 0.016 | 0.025 |
| R1-cap to L-wall | -0.160 | 0.379 | 0.011 | 0.002 | 0.638 | 0.412 | 0.000 | -1.000 | 0.000 |
| R1-cap to L-ipad | -0.138 | 0.359 | 0.011 | 0.002 | 0.588 | 0.426 | 0.005 | 0.015 | 0.028 |
| R1-cap to L-alum | -0.146 | 0.366 | 0.011 | 0.002 | 0.606 | 0.424 | 0.005 | 0.017 | 0.022 |
| | | | | | | | | | |
| Comparison | MCC_TH | EERL | EERH | EER | 0FMR | FMR1000 | FMR100 | FMR20 | FMR10 |
| R1-cap to R2-cap | 0.017 | 0.383 | 0.383 | 0.383 | 0.837 | 0.768 | 0.688 | 0.596 | 0.539 |
| R1-cap to R2-opt | 0.017 | 0.444 | 0.444 | 0.444 | 0.962 | 0.932 | 0.857 | 0.776 | 0.696 |
| R1-cap to W-opt | 0.016 | 0.518 | 0.518 | 0.518 | 0.989 | 0.981 | 0.951 | 0.882 | 0.836 |
| R1-cap to W-cap | 0.017 | 0.463 | 0.463 | 0.463 | 0.973 | 0.957 | 0.901 | 0.849 | 0.800 |
| R1-cap to Smt | 0.016 | 0.543 | 0.544 | 0.543 | 1.000 | 0.998 | 0.985 | 0.956 | 0.908 |
| R1-cap to L-wall | -1.000 | 0.552 | 0.552 | 0.552 | 1.000 | 1.000 | 0.994 | 0.962 | 0.916 |
| R1-cap to L-ipad | 0.070 | 0.547 | 0.547 | 0.547 | 0.999 | 0.999 | 0.990 | 0.959 | 0.924 |
| R1-cap to L-alum | 0.017 | 0.546 | 0.546 | 0.546 | 1.000 | 0.999 | 0.986 | 0.953 | 0.920 |
| | | | | | | | | | |
| Comparison | 0FNMR | EER_TH | 0FMR_TH | FMR1000_TH | FMR100_TH | FMR20_TH | FMR10_TH | 0FNMR_TH | |
| R1-cap to R2-cap | 1.000 | 0.011 | 0.027 | 0.021 | 0.017 | 0.014 | 0.013 | -1.000 | |
| R1-cap to R2-opt | 1.000 | 0.012 | 0.029 | 0.024 | 0.018 | 0.015 | 0.014 | -1.000 | |
| R1-cap to W-opt | 1.000 | 0.011 | 0.030 | 0.024 | 0.017 | 0.015 | 0.014 | -1.000 | |
| R1-cap to W-cap | 1.000 | 0.011 | 0.031 | 0.022 | 0.017 | 0.015 | 0.014 | -1.000 | |
| R1-cap to Smt | 1.000 | 0.011 | 0.024 | 0.020 | 0.016 | 0.014 | 0.013 | -1.000 | |
| R1-cap to L-wall | 1.000 | 0.011 | 0.027 | 0.020 | 0.016 | 0.014 | 0.013 | -1.000 | |
| R1-cap to L-ipad | 1.000 | 0.011 | 0.070 | 0.021 | 0.016 | 0.014 | 0.013 | -1.000 | |
| R1-cap to L-alum | 1.000 | 0.011 | 0.022 | 0.021 | 0.016 | 0.014 | 0.013 | -1.000 | |

*Note: **GMean:** Genuine scores distribution mean; **GSTD:** Genuine scores distribution standard deviation; **IMean:** Impostor scores distribution mean; **ISTD:** Impostor scores distribution standard deviation; **AUC:** Area under the ROC curve; **SI:** Sensitivity Index; **JI:** Youden's J Index; **TH:** THreshold; **MCC:** Matthews Correlation Coefficient; **EER:** Equal Error Rate; **EERL:** EER low; **EERH:** EER high.*

TABLE XXVII: Performance indicators measured on the 'Latent in the Wild' database for the MinutiaeNet-MCC (part 3/4) comparison experiments.

| Comparison | GMean | GSTD | IMean | ISTD | SI | AUC | JI | JI_TH | MCC |
|---|---|---|---|---|---|---|---|---|---|
| W-opt to W-cap | -0.150 | 0.372 | 0.011 | 0.002 | 0.615 | 0.482 | 0.067 | 0.012 | 0.119 |
| W-opt to Smt | -0.159 | 0.378 | 0.011 | 0.002 | 0.635 | 0.431 | 0.004 | 0.018 | 0.037 |
| W-opt to L-wall | 0.000 | 0.000 | 0.011 | 0.002 | 6.537 | 0.006 | 0.000 | 0.000 | 0.000 |
| W-opt to L-ipad | -0.139 | 0.360 | 0.011 | 0.003 | 0.591 | 0.435 | 0.017 | 0.014 | 0.022 |
| W-opt to L-alum | -0.162 | 0.381 | 0.011 | 0.003 | 0.642 | 0.418 | 0.003 | 0.020 | 0.040 |
| W-cap to Smt | -0.134 | 0.354 | 0.011 | 0.002 | 0.578 | 0.428 | 0.001 | 0.022 | 0.008 |
| W-cap to L-wall | 0.000 | 0.000 | 0.011 | 0.002 | 6.800 | 0.004 | 0.000 | 0.000 | 0.000 |
| W-cap to L-ipad | -0.130 | 0.350 | 0.011 | 0.002 | 0.569 | 0.429 | 0.004 | 0.016 | 0.019 |
| W-cap to L-alum | -0.159 | 0.378 | 0.011 | 0.003 | 0.636 | 0.425 | 0.001 | 0.017 | 0.004 |
| | | | | | | | | | |
| Comparison | MCC_TH | EERL | EERH | EER | 0FMR | FMR1000 | FMR100 | FMR20 | FMR10 |
| W-opt to W-cap | 0.025 | 0.500 | 0.500 | 0.500 | 0.984 | 0.980 | 0.959 | 0.896 | 0.848 |
| W-opt to Smt | 0.021 | 0.532 | 0.532 | 0.532 | 0.998 | 0.996 | 0.989 | 0.953 | 0.902 |
| W-opt to L-wall | 0.000 | 0.000 | 1.000 | 0.500 | 1.000 | 1.000 | 1.000 | 1.000 | 1.000 |
| W-opt to L-ipad | 0.014 | 0.535 | 0.535 | 0.535 | 1.000 | 0.999 | 0.992 | 0.944 | 0.893 |
| W-opt to L-alum | 0.024 | 0.542 | 0.543 | 0.542 | 0.997 | 0.997 | 0.988 | 0.959 | 0.921 |
| W-cap to Smt | 0.022 | 0.545 | 0.545 | 0.545 | 1.000 | 0.998 | 0.993 | 0.956 | 0.918 |
| W-cap to L-wall | 0.000 | 0.000 | 1.000 | 0.500 | 1.000 | 1.000 | 1.000 | 1.000 | 1.000 |
| W-cap to L-ipad | 0.024 | 0.542 | 0.542 | 0.542 | 1.000 | 0.998 | 0.990 | 0.958 | 0.921 |
| W-cap to L-alum | 0.017 | 0.541 | 0.541 | 0.541 | 1.000 | 1.000 | 0.991 | 0.957 | 0.907 |
| | | | | | | | | | |
| Comparison | 0FNMR | EER_TH | 0FMR_TH | FMR1000_TH | FMR100_TH | FMR20_TH | FMR10_TH | 0FNMR_TH | |
| W-opt to W-cap | 1.000 | 0.011 | 0.027 | 0.024 | 0.018 | 0.015 | 0.014 | -1.000 | |
| W-opt to Smt | 1.000 | 0.010 | 0.023 | 0.020 | 0.017 | 0.014 | 0.013 | -1.000 | |
| W-opt to L-wall | 1.000 | 0.000 | 0.030 | 0.025 | 0.017 | 0.015 | 0.014 | 0.000 | |
| W-opt to L-ipad | 1.000 | 0.011 | 0.030 | 0.024 | 0.018 | 0.015 | 0.014 | -1.000 | |
| W-opt to L-alum | 1.000 | 0.011 | 0.024 | 0.022 | 0.018 | 0.015 | 0.014 | -1.000 | |
| W-cap to Smt | 1.000 | 0.010 | 0.030 | 0.022 | 0.017 | 0.014 | 0.013 | -1.000 | |
| W-cap to L-wall | 1.000 | 0.000 | 0.032 | 0.024 | 0.018 | 0.015 | 0.014 | 0.000 | |
| W-cap to L-ipad | 1.000 | 0.011 | 0.029 | 0.024 | 0.018 | 0.015 | 0.014 | -1.000 | |
| W-cap to L-alum | 1.000 | 0.011 | 0.027 | 0.023 | 0.017 | 0.015 | 0.014 | -1.000 | |

*Note:* ***GMean:*** *Genuine scores distribution mean;* ***GSTD:*** *Genuine scores distribution standard deviation;* ***IMean:*** *Impostor scores distribution mean;* ***ISTD:*** *Impostor scores distribution standard deviation;* ***AUC:*** *Area under the ROC curve;* ***SI:*** *Sensitivity Index;* ***JI:*** *Youden's J Index;* ***TH:*** *THreshold;* ***MCC:*** *Matthews Correlation Coefficient;* ***EER:*** *Equal Error Rate;* ***EERL:*** *EER low;* ***EERH:*** *EER high.*

TABLE XXVIII: Performance indicators measured on the ’Latent in the Wild’ database for the MinutiaeNet-MCC (part 4/4) comparison experiments.

| Comparison | GMean | GSTD | IMean | ISTD | SI | AUC | JI | JI_TH | MCC |
|---|---|---|---|---|---|---|---|---|---|
| Smt to L-wall | -0.152 | 0.372 | 0.011 | 0.002 | 0.620 | 0.413 | 0.000 | 0.019 | 0.003 |
| Smt to L-ipad | -0.140 | 0.360 | 0.010 | 0.002 | 0.592 | 0.436 | 0.013 | 0.015 | 0.034 |
| Smt to L-alum | -0.156 | 0.374 | 0.010 | 0.002 | 0.627 | 0.415 | 0.000 | 0.021 | 0.006 |
| L-wall to L-ipad | -0.136 | 0.357 | 0.011 | 0.002 | 0.584 | 0.425 | 0.017 | 0.014 | 0.029 |
| L-wall to L-alum | -0.152 | 0.372 | 0.011 | 0.003 | 0.621 | 0.422 | 0.001 | 0.029 | 0.029 |
| L-ipad to L-alum | -0.149 | 0.369 | 0.011 | 0.003 | 0.612 | 0.436 | 0.003 | 0.015 | 0.005 |
| | | | | | | | | | |
| Comparison | MCC_TH | EERL | EERH | EER | 0FMR | FMR1000 | FMR100 | FMR20 | FMR10 |
| Smt to L-wall | 0.019 | 0.550 | 0.550 | 0.550 | 1.000 | 1.000 | 0.994 | 0.962 | 0.921 |
| Smt to L-ipad | 0.015 | 0.531 | 0.532 | 0.532 | 0.999 | 0.997 | 0.985 | 0.945 | 0.910 |
| Smt to L-alum | 0.021 | 0.537 | 0.538 | 0.537 | 1.000 | 0.999 | 0.991 | 0.962 | 0.935 |
| L-wall to L-ipad | 0.015 | 0.543 | 0.543 | 0.543 | 1.000 | 0.999 | 0.986 | 0.937 | 0.902 |
| L-wall to L-alum | 0.029 | 0.540 | 0.541 | 0.540 | 0.999 | 0.999 | 0.992 | 0.957 | 0.916 |
| L-ipad to L-alum | 0.015 | 0.532 | 0.533 | 0.532 | 1.000 | 1.000 | 0.994 | 0.954 | 0.910 |
| | | | | | | | | | |
| Comparison | 0FNMR | EER_TH | 0FMR_TH | FMR1000_TH | FMR100_TH | FMR20_TH | FMR10_TH | 0FNMR_TH | |
| Smt to L-wall | 1.000 | 0.010 | 0.026 | 0.022 | 0.016 | 0.014 | 0.013 | -1.000 | |
| Smt to L-ipad | 1.000 | 0.010 | 0.025 | 0.019 | 0.016 | 0.014 | 0.013 | -1.000 | |
| Smt to L-alum | 1.000 | 0.010 | 0.023 | 0.020 | 0.016 | 0.014 | 0.013 | -1.000 | |
| L-wall to L-ipad | 1.000 | 0.011 | 0.030 | 0.023 | 0.017 | 0.014 | 0.013 | -1.000 | |
| L-wall to L-alum | 1.000 | 0.011 | 0.029 | 0.023 | 0.017 | 0.015 | 0.013 | -1.000 | |
| L-ipad to L-alum | 1.000 | 0.011 | 0.032 | 0.025 | 0.017 | 0.015 | 0.014 | -1.000 | |

*Note: **GMean:** Genuine scores distribution mean; **GSTD:** Genuine scores distribution standard deviation; **IMean:** Impostor scores distribution mean; **ISTD:** Impostor scores distribution standard deviation; **AUC:** Area under the ROC curve; **SI:** Sensitivity Index; **JI:** Youden’s J Index; **TH:** THreshold; **MCC:** Matthews Correlation Coefficient; **EER:** Equal Error Rate; **EERL:** EER low; **EERH:** EER high.*

### F. Supplementary results for the MinutiaeNet-NBIS comparison experiment

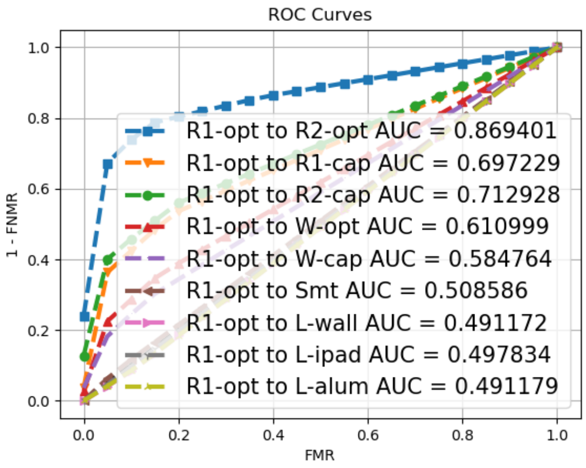


(a)

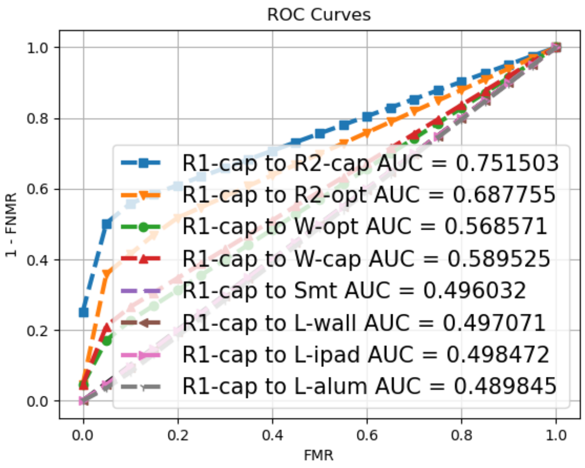


(b)

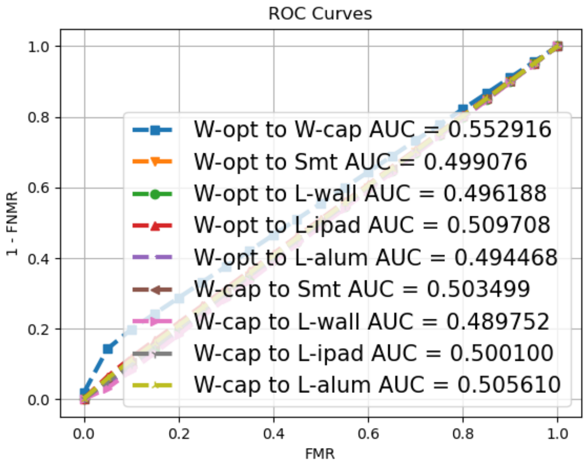


(c)

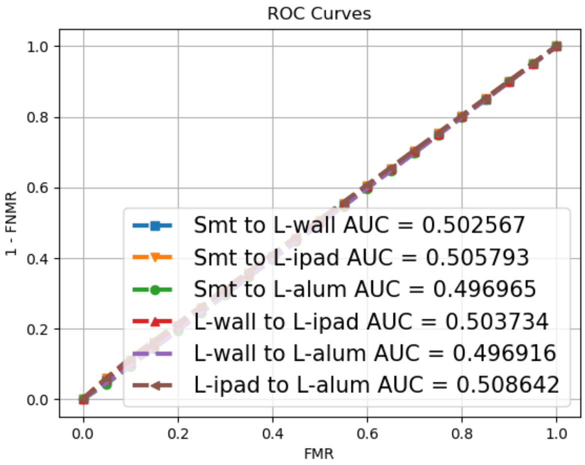


(d)

Fig. 56: ROC curve of the MinutiaeNet-NBIS comparison experiments for the 'Latent in the Wild' database

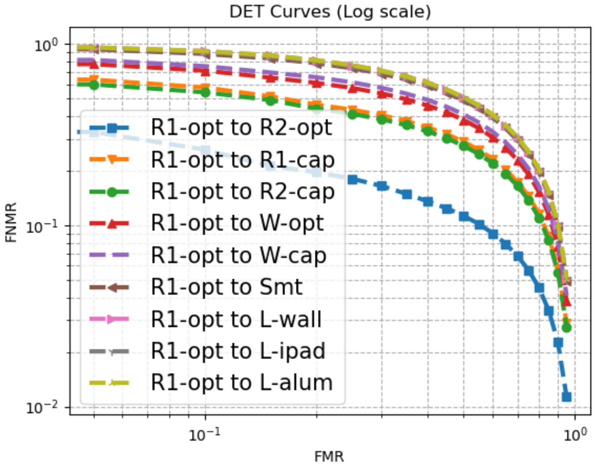


(a)

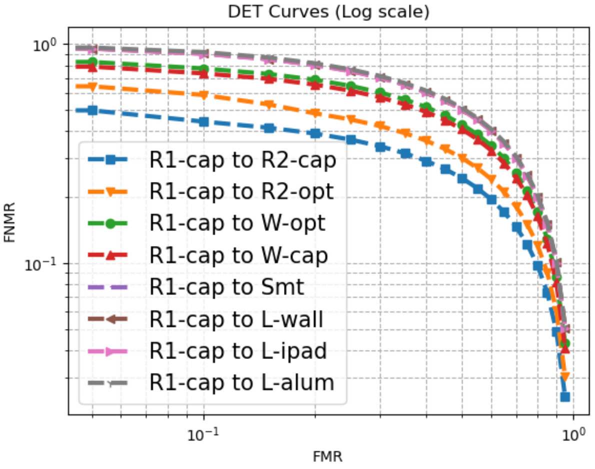


(b)

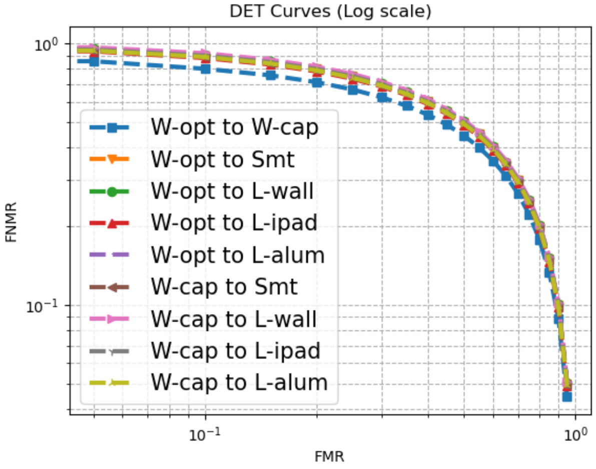


(c)

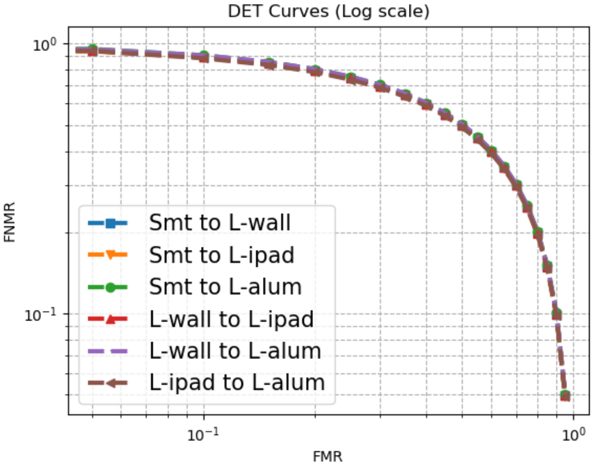


(d)

Fig. 57: DET curve of the MinutiaeNet-NBIS comparison experiments for the 'Latent in the Wild' database

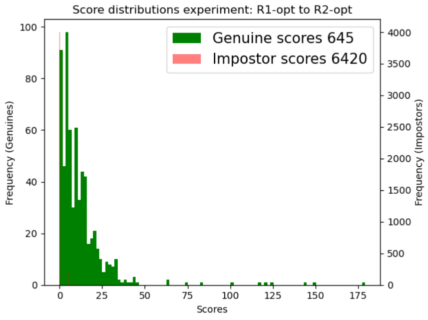


(a) R1-opt to R2-opt

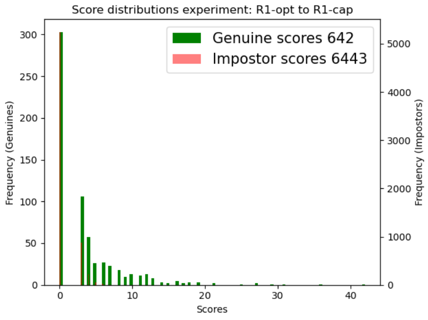


(b) R1-opt to R1-cap

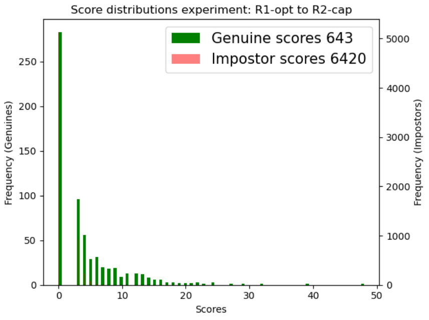


(c) R1-opt to R2-cap

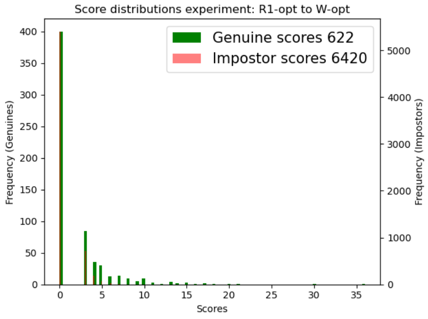


(d) R1-opt to W-opt

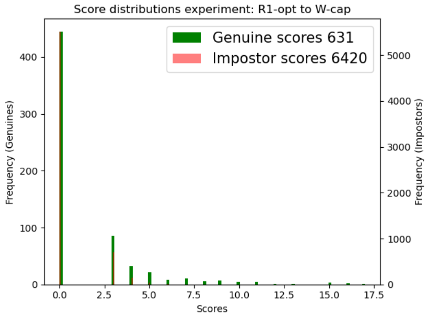


(e) R1-opt to W-cap

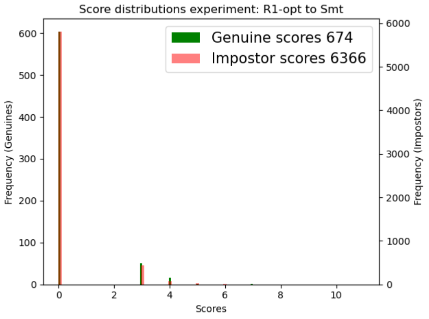


(f) R1-opt to Smt

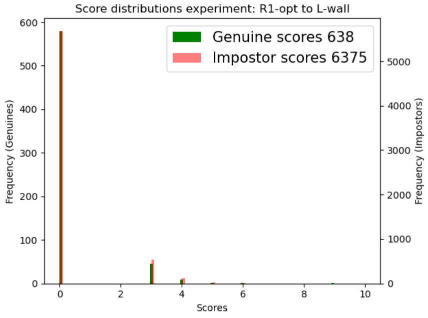


(g) R1-opt to L-wall

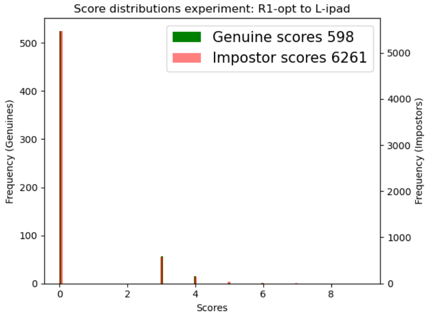


(h) R1-opt to L-ipad

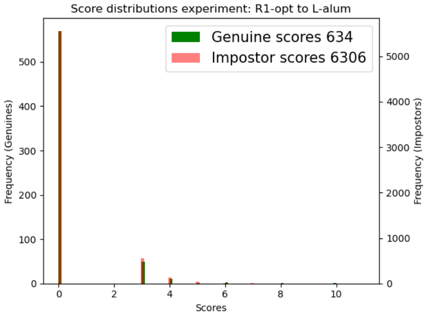


(i) R1-opt to L-alum

Fig. 58: Distributions of the MinutiaeNet-NBIS (part 1/4) comparison scores in the 'Latent in the Wild' database

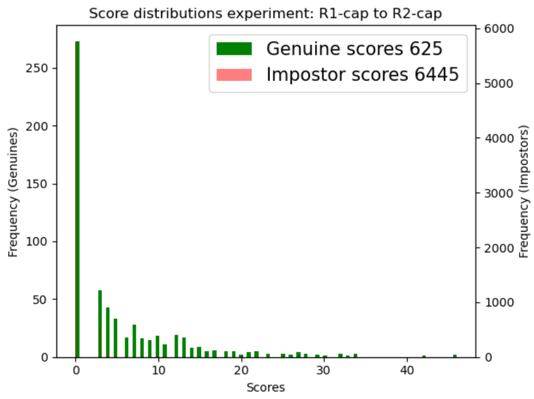


(a) R1-cap to R2-cap

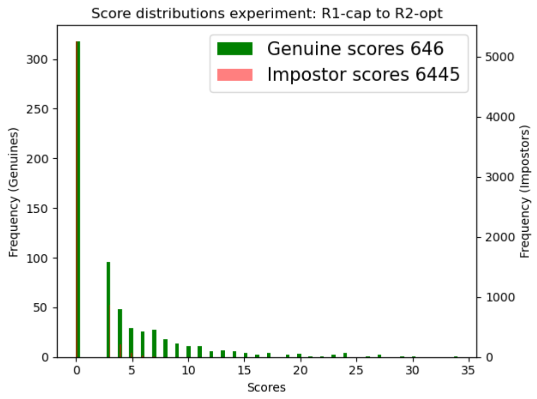


(b) R1-cap to R2-opt

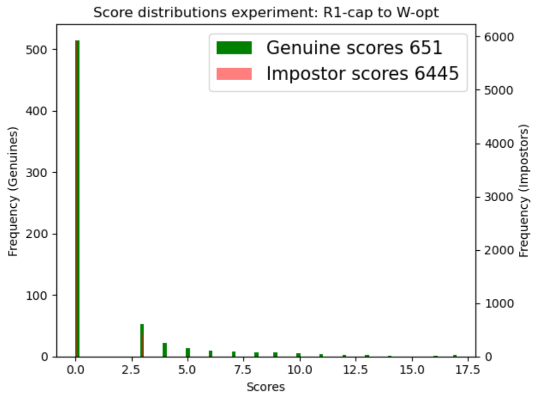


(c) R1-cap to W-opt

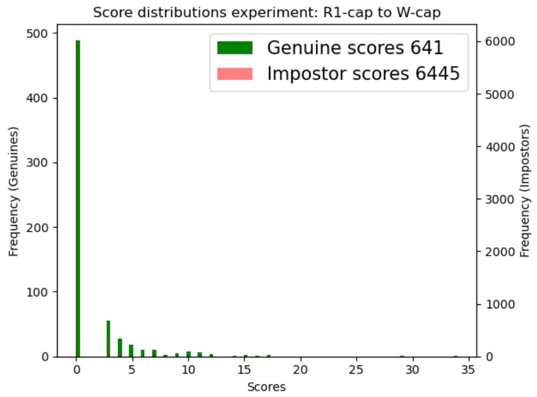


(d) R1-cap to W-cap

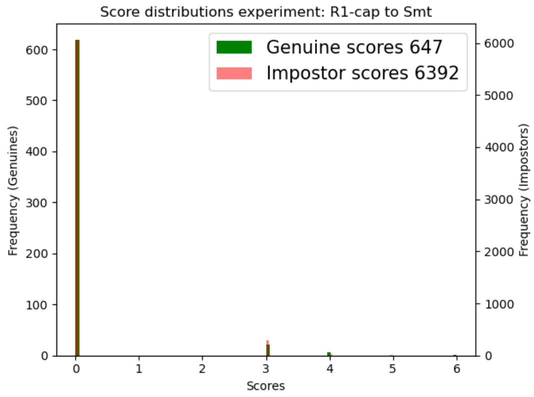


(e) R1-cap to Smt

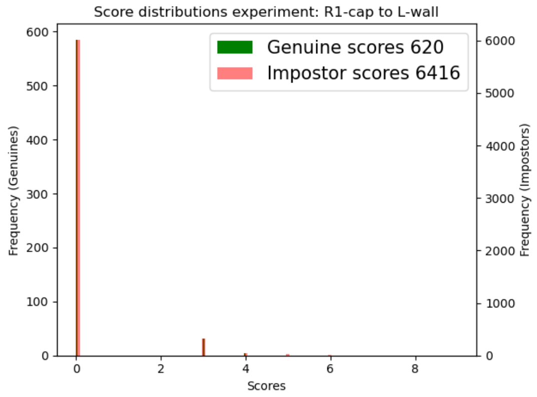


(f) R1-cap to L-wall

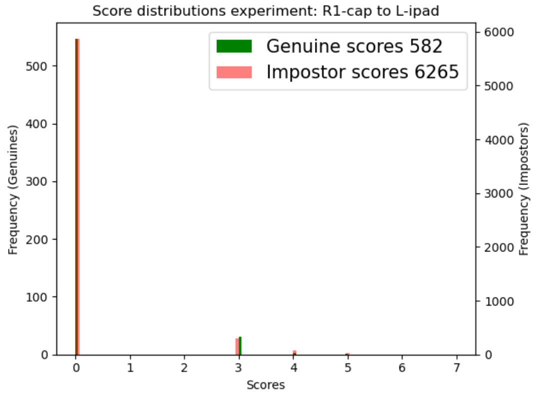


(g) R1-cap to L-ipad

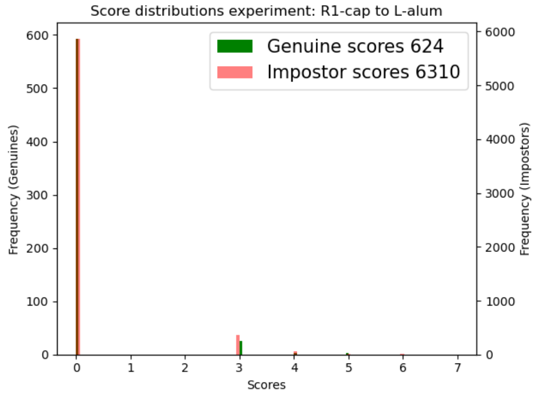


(h) R1-cap to L-alum

Fig. 59: Distributions of the MinutiaeNet-NBIS (part 2/4) comparison scores in the 'Latent in the Wild' database

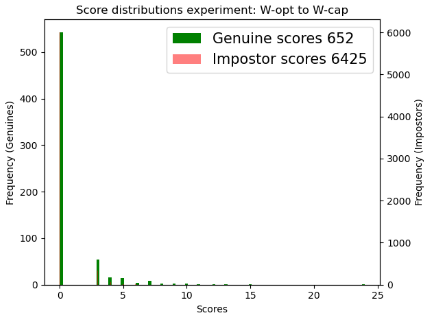


(a) W-opt to W-cap

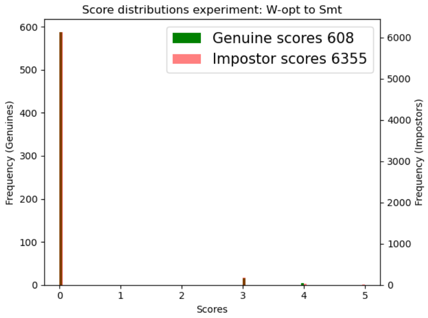


(b) W-opt to Smt

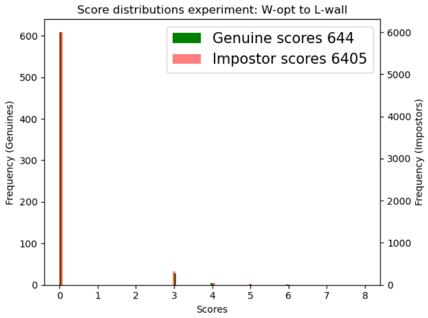


(c) W-opt to L-wall

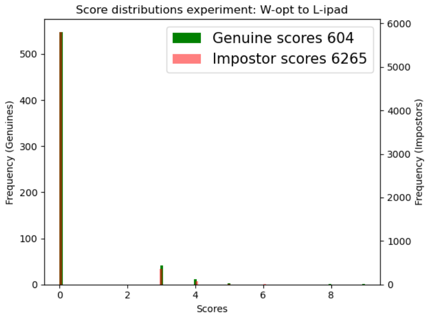


(d) W-opt to L-ipad

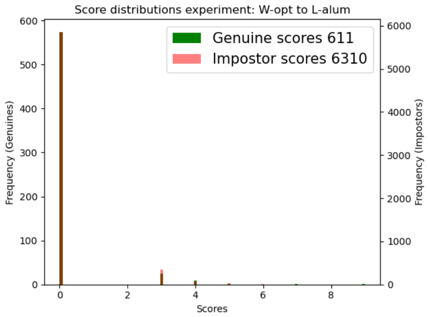


(e) W-opt to L-alum

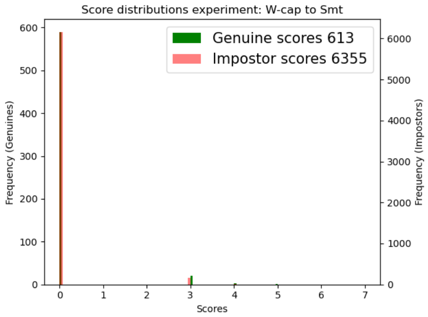


(f) W-cap to Smt

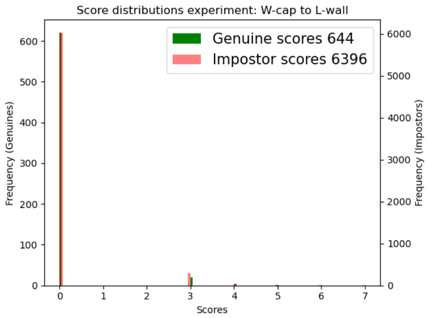


(g) W-cap to L-wall

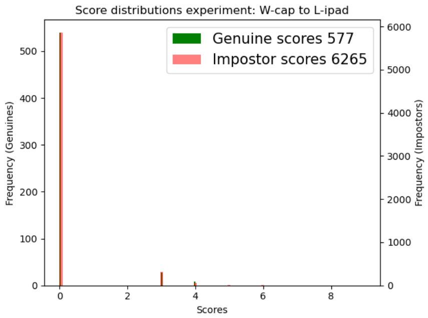


(h) W-cap to L-ipad

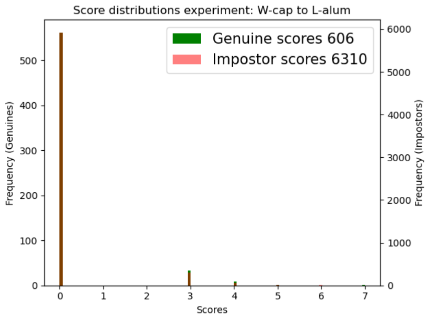


(i) W-cap to L-alum

Fig. 60: Distributions of the MinutiaeNet-NBIS (part 3/4) comparison scores in the 'Latent in the Wild' database

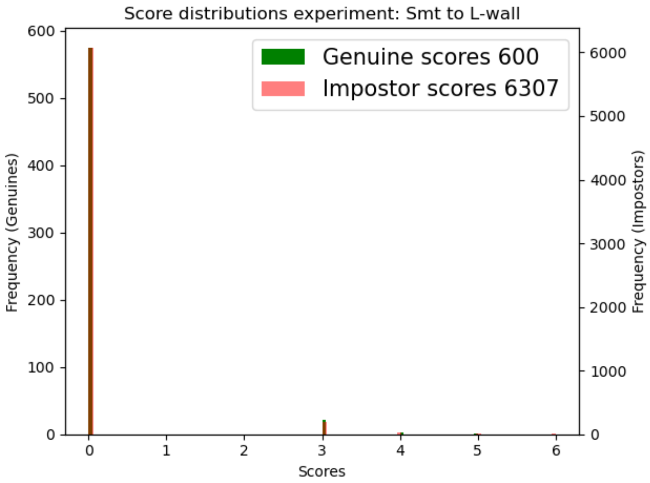


(a) Smt to L-wall

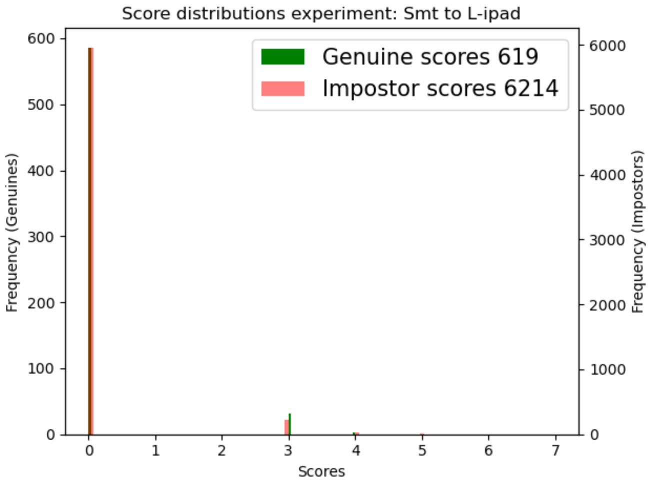


(b) Smt to L-ipad

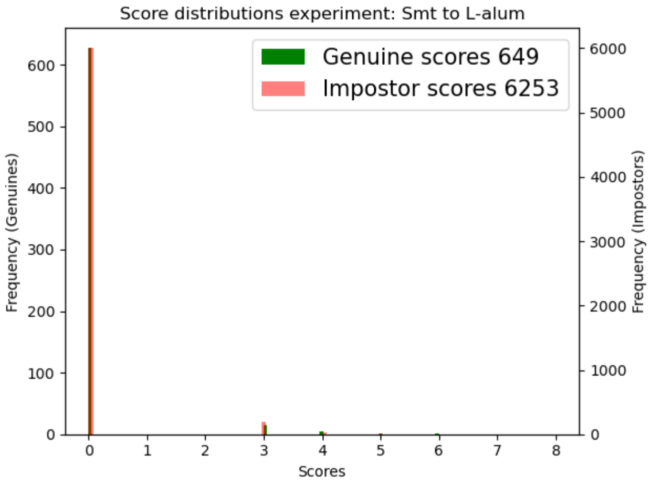


(c) Smt to L-alum

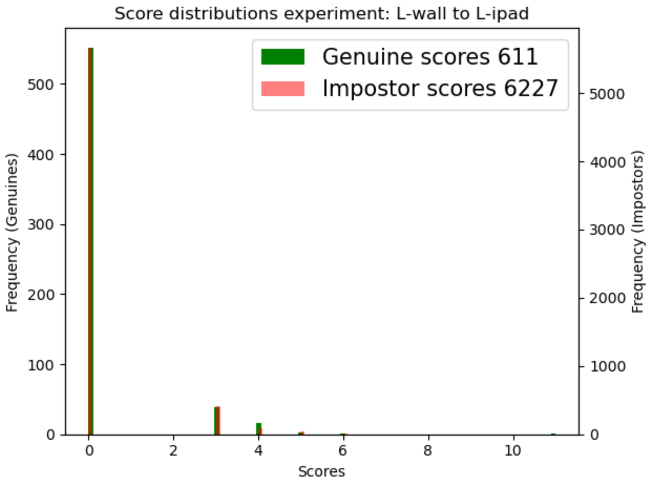


(d) L-wall to L-ipad

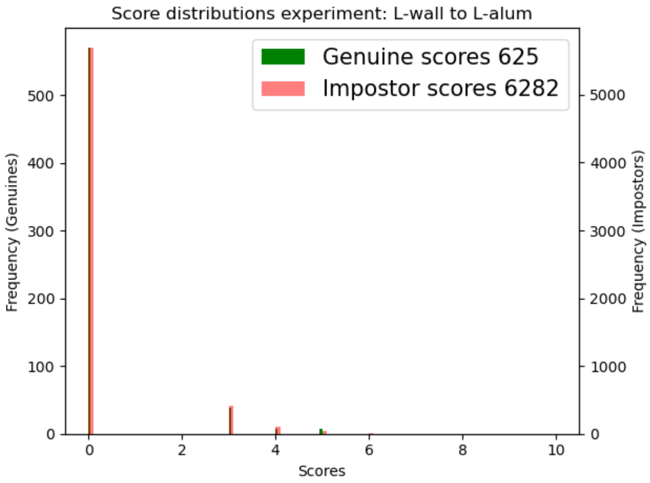


(e) L-wall to L-alum

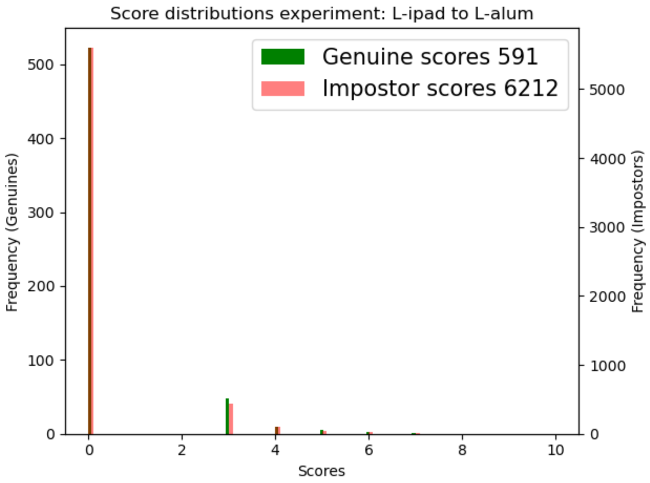


(f) L-ipad to L-alum

Fig. 61: Distributions of the MinutiaeNet-NBIS (part 4/4) comparison scores in the 'Latent in the Wild' database

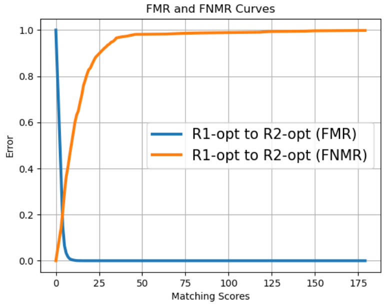


(a) R1-opt to R2-opt

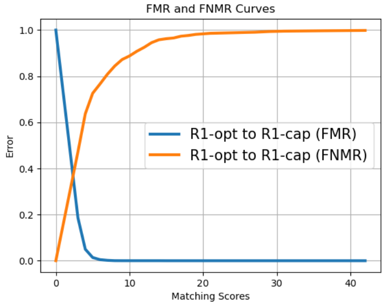


(b) R1-opt to R1-cap

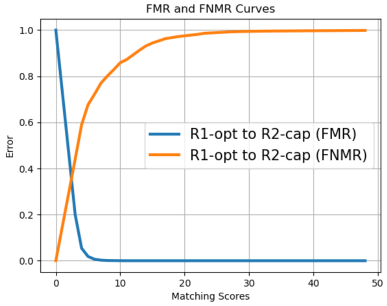


(c) R1-opt to R2-cap

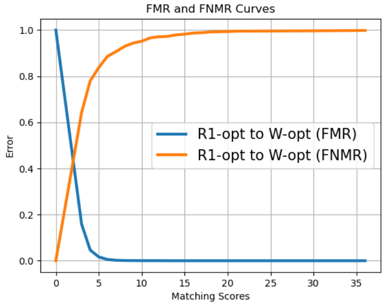


(d) R1-opt to W-opt

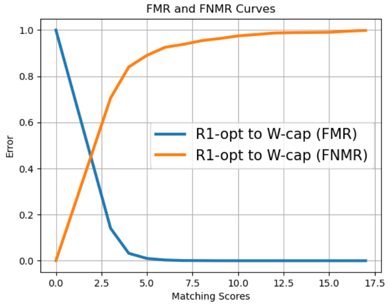


(e) R1-opt to W-cap

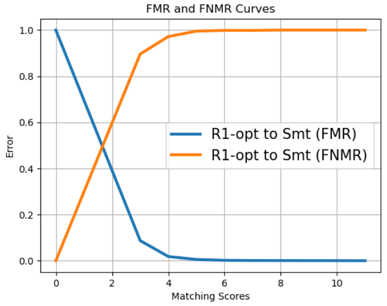


(f) R1-opt to Smt

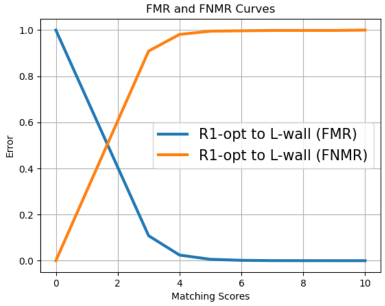


(g) R1-opt to L-wall

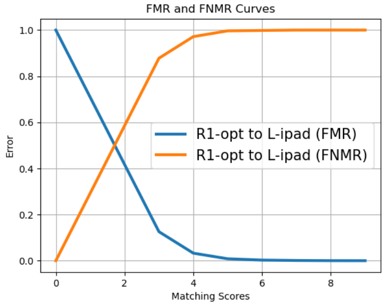


(h) R1-opt to L-ipad

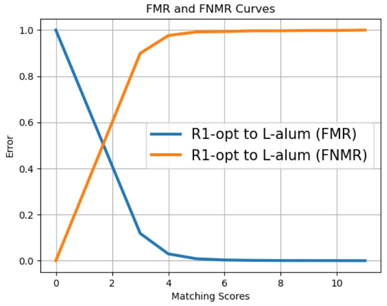


(i) R1-opt to L-alum

Fig. 62: FMR and FNMR curves of the MinutiaeNet-NBIS (part 1/4) comparison scores in the 'Latent in the Wild' database

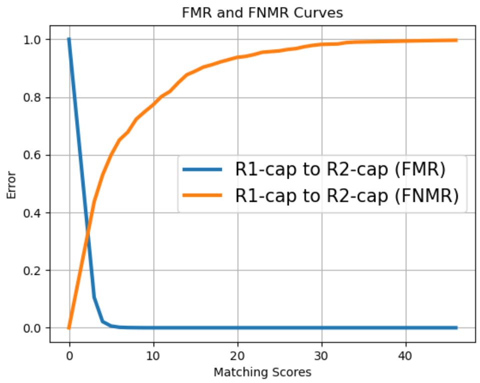


(a) R1-cap to R2-cap

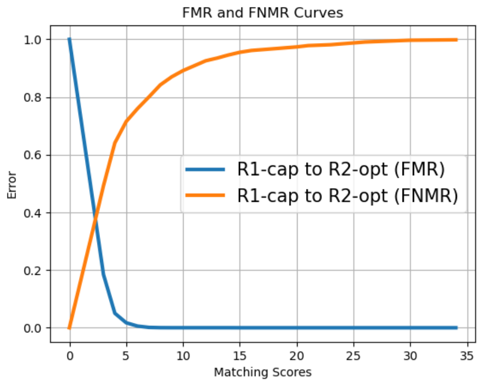


(b) R1-cap to R2-opt

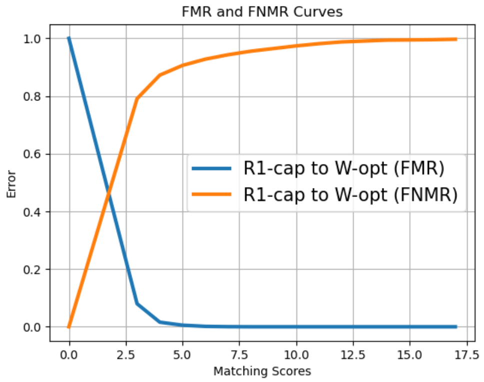


(c) R1-cap to W-opt

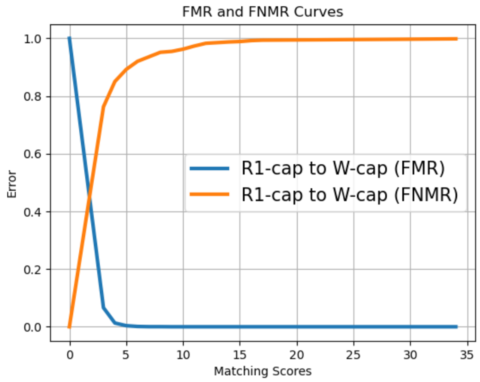


(d) R1-cap to W-cap

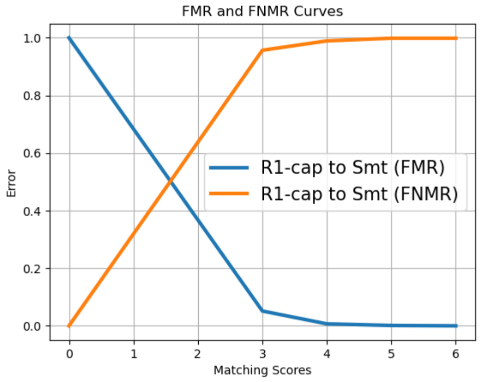


(e) R1-cap to Smt

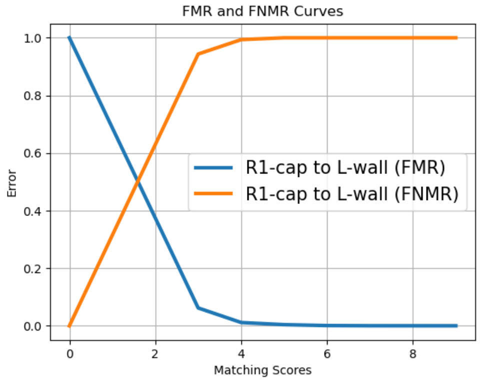


(f) R1-cap to L-wall

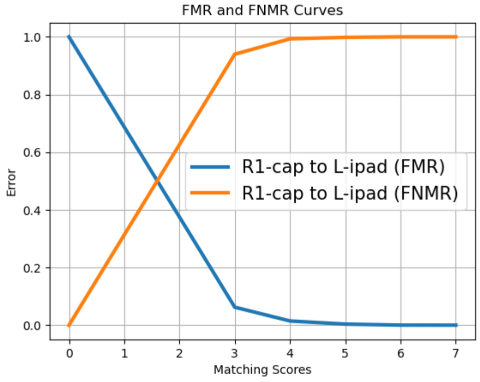


(g) R1-cap to L-ipad

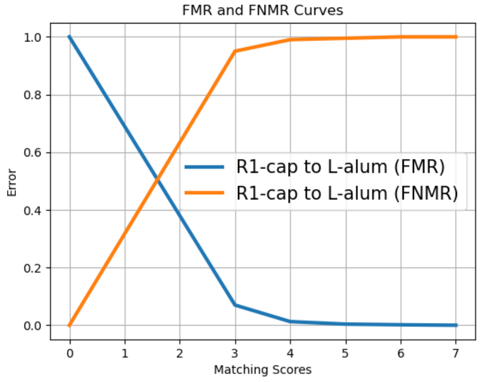


(h) R1-cap to L-alum

Fig. 63: FMR and FNMR curves of the MinutiaeNet-NBIS (part 2/4) comparison scores in the 'Latent in the Wild' database

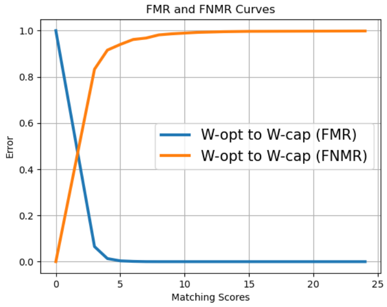


(a) W-opt to W-cap

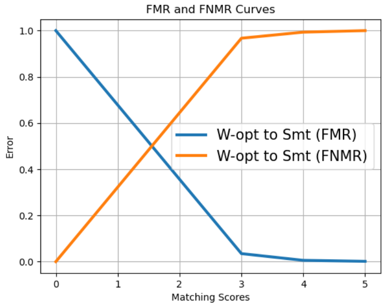


(b) W-opt to Smt

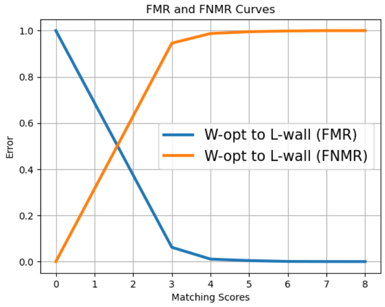


(c) W-opt to L-wall

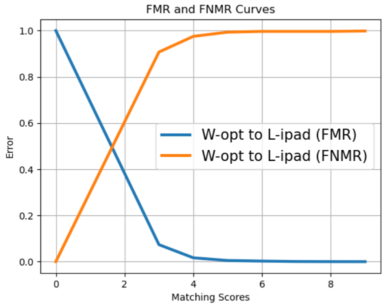


(d) W-opt to L-ipad

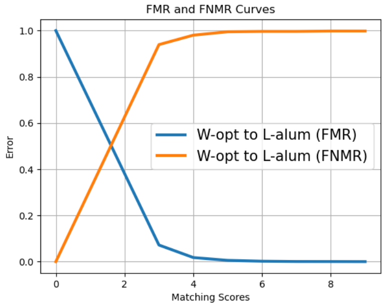


(e) W-opt to L-alum

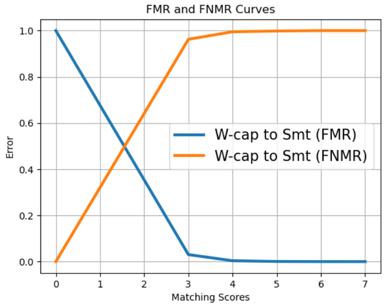


(f) W-cap to Smt

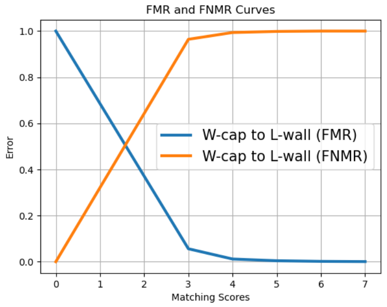


(g) W-cap to L-wall

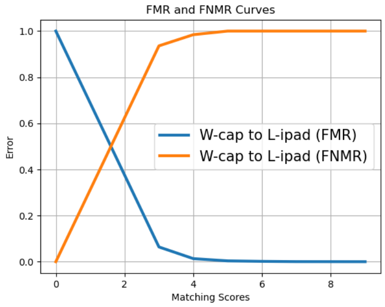


(h) W-cap to L-ipad

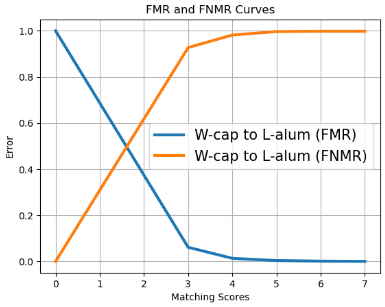


(i) W-cap to L-alum

Fig. 64: FMR and FNMR curves of the MinutiaeNet-NBIS (part 3/4) comparison scores in the 'Latent in the Wild' database

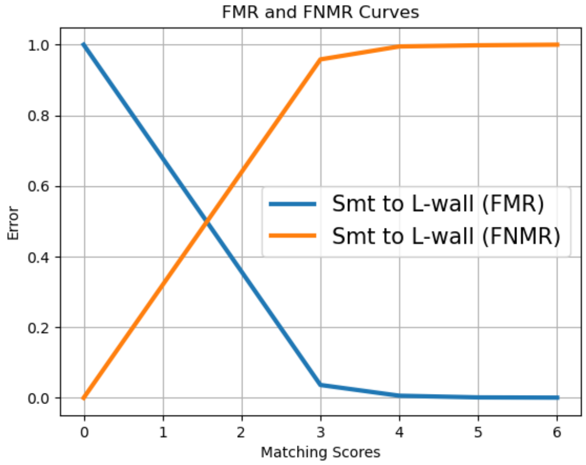


(a) Smt to L-wall

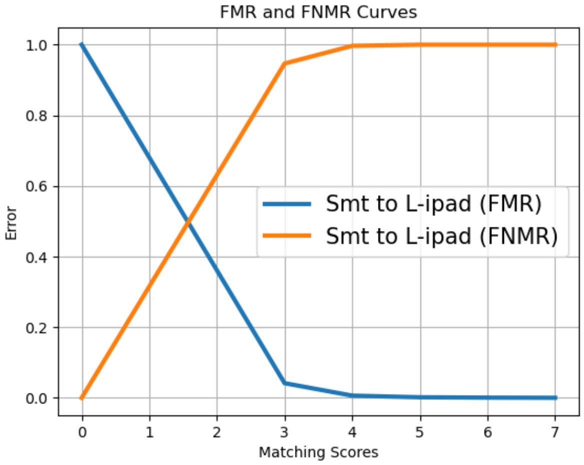


(b) Smt to L-ipad

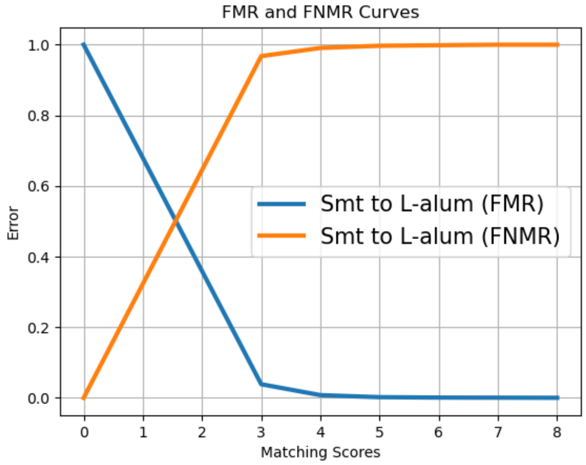


(c) Smt to L-alum

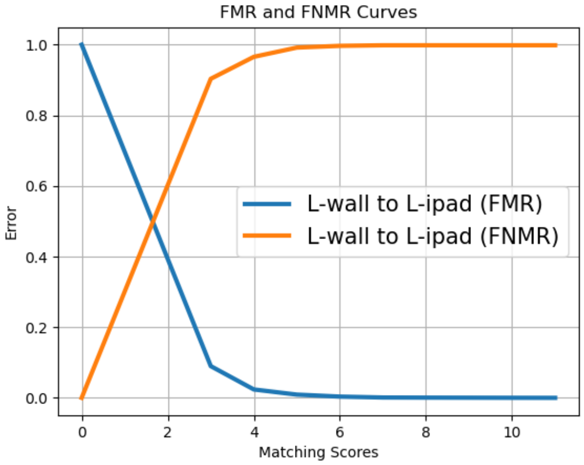


(d) L-wall to L-ipad

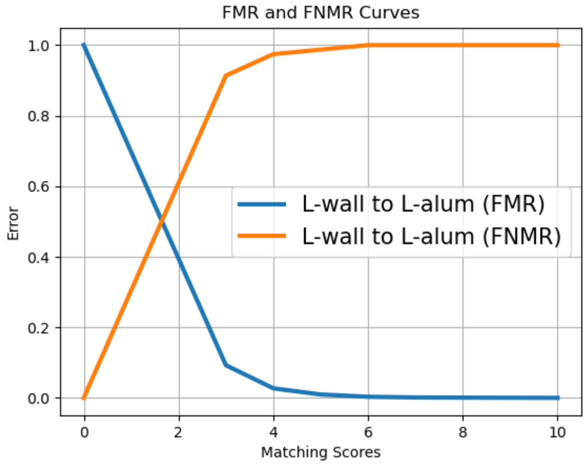


(e) L-wall to L-alum

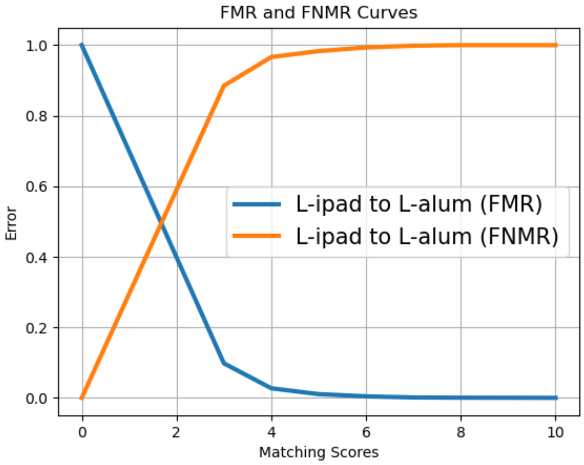


(f) L-ipad to L-alum

Fig. 65: FMR and FNMR curves of the MinutiaeNet-NBIS (part 4/4) comparison scores in the 'Latent in the Wild' database

TABLE XXIX: Performance indicators measured on the 'Latent in the Wild' database for the MinutiaeNet-NBIS (part 1/4) comparison experiments.

| Comparison | GMean | GSTD | IMean | ISTD | SI | AUC | JI | JI_TH | MCC |
|---|---|---|---|---|---|---|---|---|---|
| R1-opt to R2-opt | -0.102 | 0.362 | 0.012 | 0.002 | 0.445 | 0.732 | 0.478 | 0.015 | 0.544 |
| R1-opt to R1-cap | -0.155 | 0.379 | 0.012 | 0.002 | 0.623 | 0.569 | 0.207 | 0.013 | 0.262 |
| R1-opt to R2-cap | -0.138 | 0.363 | 0.012 | 0.002 | 0.582 | 0.601 | 0.261 | 0.014 | 0.330 |
| R1-opt to W-opt | -0.140 | 0.364 | 0.012 | 0.002 | 0.590 | 0.513 | 0.127 | 0.014 | 0.192 |
| R1-opt to W-cap | -0.147 | 0.370 | 0.012 | 0.002 | 0.607 | 0.493 | 0.085 | 0.015 | 0.185 |
| R1-opt to Smt | -0.145 | 0.365 | 0.011 | 0.002 | 0.604 | 0.418 | 0.003 | 0.021 | 0.033 |
| R1-opt to L-wall | -0.126 | 0.347 | 0.011 | 0.002 | 0.561 | 0.430 | 0.001 | 0.018 | 0.006 |
| R1-opt to L-ipad | -0.122 | 0.342 | 0.011 | 0.002 | 0.550 | 0.441 | 0.004 | 0.020 | 0.024 |
| R1-opt to L-alum | -0.156 | 0.375 | 0.011 | 0.003 | 0.629 | 0.419 | 0.000 | 0.024 | 0.002 |
| | | | | | | | | | |
| Comparison | MCC_TH | EERL | EERH | EER | 0FMR | FMR1000 | FMR100 | FMR20 | FMR10 |
| R1-opt to R2-opt | 0.019 | 0.306 | 0.307 | 0.306 | 0.833 | 0.728 | 0.623 | 0.489 | 0.423 |
| R1-opt to R1-cap | 0.018 | 0.434 | 0.434 | 0.434 | 0.966 | 0.938 | 0.870 | 0.771 | 0.706 |
| R1-opt to R2-cap | 0.018 | 0.415 | 0.416 | 0.415 | 0.968 | 0.910 | 0.824 | 0.717 | 0.640 |
| R1-opt to W-opt | 0.024 | 0.491 | 0.491 | 0.491 | 0.980 | 0.958 | 0.922 | 0.850 | 0.780 |
| R1-opt to W-cap | 0.021 | 0.498 | 0.499 | 0.499 | 0.988 | 0.963 | 0.933 | 0.875 | 0.824 |
| R1-opt to Smt | 0.023 | 0.545 | 0.546 | 0.546 | 0.999 | 0.996 | 0.992 | 0.955 | 0.913 |
| R1-opt to L-wall | 0.027 | 0.537 | 0.538 | 0.537 | 1.000 | 0.999 | 0.991 | 0.962 | 0.909 |
| R1-opt to L-ipad | 0.020 | 0.519 | 0.519 | 0.519 | 1.000 | 1.000 | 0.989 | 0.962 | 0.926 |
| R1-opt to L-alum | 0.024 | 0.541 | 0.542 | 0.542 | 1.000 | 0.999 | 0.996 | 0.956 | 0.913 |
| | | | | | | | | | |
| Comparison | 0FNMR | EER_TH | 0FMR_TH | FMR1000_TH | FMR100_TH | FMR20_TH | FMR10_TH | 0FNMR_TH | |
| R1-opt to R2-opt | 1.000 | 0.013 | 0.034 | 0.026 | 0.020 | 0.016 | 0.015 | -1.000 | |
| R1-opt to R1-cap | 1.000 | 0.012 | 0.029 | 0.023 | 0.018 | 0.015 | 0.014 | -1.000 | |
| R1-opt to R2-cap | 1.000 | 0.012 | 0.031 | 0.022 | 0.018 | 0.015 | 0.014 | -1.000 | |
| R1-opt to W-opt | 1.000 | 0.012 | 0.034 | 0.026 | 0.019 | 0.016 | 0.015 | -1.000 | |
| R1-opt to W-cap | 1.000 | 0.012 | 0.033 | 0.023 | 0.019 | 0.016 | 0.014 | -1.000 | |
| R1-opt to Smt | 1.000 | 0.011 | 0.026 | 0.021 | 0.016 | 0.014 | 0.013 | -1.000 | |
| R1-opt to L-wall | 1.000 | 0.011 | 0.030 | 0.023 | 0.017 | 0.015 | 0.013 | -1.000 | |
| R1-opt to L-ipad | 1.000 | 0.011 | 0.025 | 0.023 | 0.018 | 0.015 | 0.014 | -1.000 | |
| R1-opt to L-alum | 1.000 | 0.011 | 0.026 | 0.023 | 0.018 | 0.015 | 0.014 | -1.000 | |

*Note:* ***GMean:*** *Genuine scores distribution mean;* ***GSTD:*** *Genuine scores distribution standard deviation;* ***IMean:*** *Impostor scores distribution mean;* ***ISTD:*** *Impostor scores distribution standard deviation;* ***AUC:*** *Area under the ROC curve;* ***SI:*** *Sensitivity Index;* ***JI:*** *Youden's J Index;* ***TH:*** *THreshold;* ***MCC:*** *Matthews Correlation Coefficient;* ***EER:*** *Equal Error Rate;* ***EERL:*** *EER low;* ***EERH:*** *EER high.*

TABLE XXX: Performance indicators measured on the 'Latent in the Wild' database for the MinutiaeNet-NBIS (part 2/4) comparison experiments.

| Comparison | GMean | GSTD | IMean | ISTD | SI | AUC | JI | JI_TH | MCC |
|---|---|---|---|---|---|---|---|---|---|
| R1-cap to R2-cap | -0.147 | 0.378 | 0.011 | 0.002 | 0.593 | 0.642 | 0.368 | 0.014 | 0.476 |
| R1-cap to R2-opt | -0.162 | 0.385 | 0.012 | 0.002 | 0.637 | 0.565 | 0.207 | 0.013 | 0.291 |
| R1-cap to W-opt | -0.164 | 0.384 | 0.011 | 0.002 | 0.645 | 0.470 | 0.072 | 0.014 | 0.129 |
| R1-cap to W-cap | -0.147 | 0.370 | 0.011 | 0.002 | 0.606 | 0.522 | 0.118 | 0.012 | 0.213 |
| R1-cap to Smt | -0.150 | 0.370 | 0.011 | 0.002 | 0.614 | 0.425 | 0.007 | 0.016 | 0.025 |
| R1-cap to L-wall | -0.160 | 0.379 | 0.011 | 0.002 | 0.638 | 0.412 | 0.000 | -1.000 | 0.000 |
| R1-cap to L-ipad | -0.138 | 0.359 | 0.011 | 0.002 | 0.588 | 0.426 | 0.005 | 0.015 | 0.028 |
| R1-cap to L-alum | -0.146 | 0.366 | 0.011 | 0.002 | 0.606 | 0.424 | 0.005 | 0.017 | 0.022 |
| | | | | | | | | | |
| Comparison | MCC_TH | EERL | EERH | EER | 0FMR | FMR1000 | FMR100 | FMR20 | FMR10 |
| R1-cap to R2-cap | 0.017 | 0.383 | 0.383 | 0.383 | 0.837 | 0.768 | 0.688 | 0.596 | 0.539 |
| R1-cap to R2-opt | 0.017 | 0.444 | 0.444 | 0.444 | 0.962 | 0.932 | 0.857 | 0.776 | 0.696 |
| R1-cap to W-opt | 0.016 | 0.518 | 0.518 | 0.518 | 0.989 | 0.981 | 0.951 | 0.882 | 0.836 |
| R1-cap to W-cap | 0.017 | 0.463 | 0.463 | 0.463 | 0.973 | 0.957 | 0.901 | 0.849 | 0.800 |
| R1-cap to Smt | 0.016 | 0.543 | 0.544 | 0.543 | 1.000 | 0.998 | 0.985 | 0.956 | 0.908 |
| R1-cap to L-wall | -1.000 | 0.552 | 0.552 | 0.552 | 1.000 | 1.000 | 0.994 | 0.962 | 0.916 |
| R1-cap to L-ipad | 0.070 | 0.547 | 0.547 | 0.547 | 0.999 | 0.999 | 0.990 | 0.959 | 0.924 |
| R1-cap to L-alum | 0.017 | 0.546 | 0.546 | 0.546 | 1.000 | 0.999 | 0.986 | 0.953 | 0.920 |
| | | | | | | | | | |
| Comparison | 0FNMR | EER_TH | 0FMR_TH | FMR1000_TH | FMR100_TH | FMR20_TH | FMR10_TH | 0FNMR_TH | |
| R1-cap to R2-cap | 1.000 | 0.011 | 0.027 | 0.021 | 0.017 | 0.014 | 0.013 | -1.000 | |
| R1-cap to R2-opt | 1.000 | 0.012 | 0.029 | 0.024 | 0.018 | 0.015 | 0.014 | -1.000 | |
| R1-cap to W-opt | 1.000 | 0.011 | 0.030 | 0.024 | 0.017 | 0.015 | 0.014 | -1.000 | |
| R1-cap to W-cap | 1.000 | 0.011 | 0.031 | 0.022 | 0.017 | 0.015 | 0.014 | -1.000 | |
| R1-cap to Smt | 1.000 | 0.011 | 0.024 | 0.020 | 0.016 | 0.014 | 0.013 | -1.000 | |
| R1-cap to L-wall | 1.000 | 0.011 | 0.027 | 0.020 | 0.016 | 0.014 | 0.013 | -1.000 | |
| R1-cap to L-ipad | 1.000 | 0.011 | 0.070 | 0.021 | 0.016 | 0.014 | 0.013 | -1.000 | |
| R1-cap to L-alum | 1.000 | 0.011 | 0.022 | 0.021 | 0.016 | 0.014 | 0.013 | -1.000 | |

*Note: **GMean:** Genuine scores distribution mean; **GSTD:** Genuine scores distribution standard deviation; **IMean:** Impostor scores distribution mean; **ISTD:** Impostor scores distribution standard deviation; **AUC:** Area under the ROC curve; **SI:** Sensitivity Index; **JI:** Youden's J Index; **TH:** THreshold; **MCC:** Matthews Correlation Coefficient; **EER:** Equal Error Rate; **EERL:** EER low; **EERH:** EER high.*

TABLE XXXI: Performance indicators measured on the 'Latent in the Wild' database for the MinutiaeNet-NBIS (part 3/4) comparison experiments.

| Comparison | GMean | GSTD | IMean | ISTD | SI | AUC | JI | JI_TH | MCC |
|---|---|---|---|---|---|---|---|---|---|
| W-opt to W-cap | -0.150 | 0.372 | 0.011 | 0.002 | 0.615 | 0.482 | 0.067 | 0.012 | 0.119 |
| W-opt to Smt | -0.159 | 0.378 | 0.011 | 0.002 | 0.635 | 0.431 | 0.004 | 0.018 | 0.037 |
| W-opt to L-wall | 0.000 | 0.000 | 0.011 | 0.002 | 6.537 | 0.006 | 0.000 | 0.000 | 0.000 |
| W-opt to L-ipad | -0.139 | 0.360 | 0.011 | 0.003 | 0.591 | 0.435 | 0.017 | 0.014 | 0.022 |
| W-opt to L-alum | -0.162 | 0.381 | 0.011 | 0.003 | 0.642 | 0.418 | 0.003 | 0.020 | 0.040 |
| W-cap to Smt | -0.134 | 0.354 | 0.011 | 0.002 | 0.578 | 0.428 | 0.001 | 0.022 | 0.008 |
| W-cap to L-wall | 0.000 | 0.000 | 0.011 | 0.002 | 6.800 | 0.004 | 0.000 | 0.000 | 0.000 |
| W-cap to L-ipad | -0.130 | 0.350 | 0.011 | 0.002 | 0.569 | 0.429 | 0.004 | 0.016 | 0.019 |
| W-cap to L-alum | -0.159 | 0.378 | 0.011 | 0.003 | 0.636 | 0.425 | 0.001 | 0.017 | 0.004 |
| | | | | | | | | | |
| Comparison | MCC_TH | EERL | EERH | EER | 0FMR | FMR1000 | FMR100 | FMR20 | FMR10 |
| W-opt to W-cap | 0.025 | 0.500 | 0.500 | 0.500 | 0.984 | 0.980 | 0.959 | 0.896 | 0.848 |
| W-opt to Smt | 0.021 | 0.532 | 0.532 | 0.532 | 0.998 | 0.996 | 0.989 | 0.953 | 0.902 |
| W-opt to L-wall | 0.000 | 0.000 | 1.000 | 0.500 | 1.000 | 1.000 | 1.000 | 1.000 | 1.000 |
| W-opt to L-ipad | 0.014 | 0.535 | 0.535 | 0.535 | 1.000 | 0.999 | 0.992 | 0.944 | 0.893 |
| W-opt to L-alum | 0.024 | 0.542 | 0.543 | 0.542 | 0.997 | 0.997 | 0.988 | 0.959 | 0.921 |
| W-cap to Smt | 0.022 | 0.545 | 0.545 | 0.545 | 1.000 | 0.998 | 0.993 | 0.956 | 0.918 |
| W-cap to L-wall | 0.000 | 0.000 | 1.000 | 0.500 | 1.000 | 1.000 | 1.000 | 1.000 | 1.000 |
| W-cap to L-ipad | 0.024 | 0.542 | 0.542 | 0.542 | 1.000 | 0.998 | 0.990 | 0.958 | 0.921 |
| W-cap to L-alum | 0.017 | 0.541 | 0.541 | 0.541 | 1.000 | 1.000 | 0.991 | 0.957 | 0.907 |
| | | | | | | | | | |
| Comparison | 0FNMR | EER_TH | 0FMR_TH | FMR1000_TH | FMR100_TH | FMR20_TH | FMR10_TH | 0FNMR_TH | |
| W-opt to W-cap | 1.000 | 0.011 | 0.027 | 0.024 | 0.018 | 0.015 | 0.014 | -1.000 | |
| W-opt to Smt | 1.000 | 0.010 | 0.023 | 0.020 | 0.017 | 0.014 | 0.013 | -1.000 | |
| W-opt to L-wall | 1.000 | 0.000 | 0.030 | 0.025 | 0.017 | 0.015 | 0.014 | 0.000 | |
| W-opt to L-ipad | 1.000 | 0.011 | 0.030 | 0.024 | 0.018 | 0.015 | 0.014 | -1.000 | |
| W-opt to L-alum | 1.000 | 0.011 | 0.024 | 0.022 | 0.018 | 0.015 | 0.014 | -1.000 | |
| W-cap to Smt | 1.000 | 0.010 | 0.030 | 0.022 | 0.017 | 0.014 | 0.013 | -1.000 | |
| W-cap to L-wall | 1.000 | 0.000 | 0.032 | 0.024 | 0.018 | 0.015 | 0.014 | 0.000 | |
| W-cap to L-ipad | 1.000 | 0.011 | 0.029 | 0.024 | 0.018 | 0.015 | 0.014 | -1.000 | |
| W-cap to L-alum | 1.000 | 0.011 | 0.027 | 0.023 | 0.017 | 0.015 | 0.014 | -1.000 | |

*Note: **GMean:** Genuine scores distribution mean; **GSTD:** Genuine scores distribution standard deviation; **IMean:** Impostor scores distribution mean; **ISTD:** Impostor scores distribution standard deviation; **AUC:** Area under the ROC curve; **SI:** Sensitivity Index; **JI:** Youden's J Index; **TH:** THreshold; **MCC:** Matthews Correlation Coefficient; **EER:** Equal Error Rate; **EERL:** EER low; **EERH:** EER high.*

TABLE XXXII: Performance indicators measured on the 'Latent in the Wild' database for the MinutiaeNet-NBIS (part 4/4) comparison experiments.

| Comparison | GMean | GSTD | IMean | ISTD | SI | AUC | JI | JI_TH | MCC |
|---|---|---|---|---|---|---|---|---|---|
| Smt to L-wall | -0.152 | 0.372 | 0.011 | 0.002 | 0.620 | 0.413 | 0.000 | 0.019 | 0.003 |
| Smt to L-ipad | -0.140 | 0.360 | 0.010 | 0.002 | 0.592 | 0.436 | 0.013 | 0.015 | 0.034 |
| Smt to L-alum | -0.156 | 0.374 | 0.010 | 0.002 | 0.627 | 0.415 | 0.000 | 0.021 | 0.006 |
| L-wall to L-ipad | -0.136 | 0.357 | 0.011 | 0.002 | 0.584 | 0.425 | 0.017 | 0.014 | 0.029 |
| L-wall to L-alum | -0.152 | 0.372 | 0.011 | 0.003 | 0.621 | 0.422 | 0.001 | 0.029 | 0.029 |
| L-ipad to L-alum | -0.149 | 0.369 | 0.011 | 0.003 | 0.612 | 0.436 | 0.003 | 0.015 | 0.005 |
| | | | | | | | | | |
| Comparison | MCC_TH | EERL | EERH | EER | 0FMR | FMR1000 | FMR100 | FMR20 | FMR10 |
| Smt to L-wall | 0.019 | 0.550 | 0.550 | 0.550 | 1.000 | 1.000 | 0.994 | 0.962 | 0.921 |
| Smt to L-ipad | 0.015 | 0.531 | 0.532 | 0.532 | 0.999 | 0.997 | 0.985 | 0.945 | 0.910 |
| Smt to L-alum | 0.021 | 0.537 | 0.538 | 0.537 | 1.000 | 0.999 | 0.991 | 0.962 | 0.935 |
| L-wall to L-ipad | 0.015 | 0.543 | 0.543 | 0.543 | 1.000 | 0.999 | 0.986 | 0.937 | 0.902 |
| L-wall to L-alum | 0.029 | 0.540 | 0.541 | 0.540 | 0.999 | 0.999 | 0.992 | 0.957 | 0.916 |
| L-ipad to L-alum | 0.015 | 0.532 | 0.533 | 0.532 | 1.000 | 1.000 | 0.994 | 0.954 | 0.910 |
| | | | | | | | | | |
| Comparison | 0FNMR | EER_TH | 0FMR_TH | FMR1000_TH | FMR100_TH | FMR20_TH | FMR10_TH | 0FNMR_TH | |
| Smt to L-wall | 1.000 | 0.010 | 0.026 | 0.022 | 0.016 | 0.014 | 0.013 | -1.000 | |
| Smt to L-ipad | 1.000 | 0.010 | 0.025 | 0.019 | 0.016 | 0.014 | 0.013 | -1.000 | |
| Smt to L-alum | 1.000 | 0.010 | 0.023 | 0.020 | 0.016 | 0.014 | 0.013 | -1.000 | |
| L-wall to L-ipad | 1.000 | 0.011 | 0.030 | 0.023 | 0.017 | 0.014 | 0.013 | -1.000 | |
| L-wall to L-alum | 1.000 | 0.011 | 0.029 | 0.023 | 0.017 | 0.015 | 0.013 | -1.000 | |
| L-ipad to L-alum | 1.000 | 0.011 | 0.032 | 0.025 | 0.017 | 0.015 | 0.014 | -1.000 | |

*Note:* ***GMean:*** *Genuine scores distribution mean;* ***GSTD:*** *Genuine scores distribution standard deviation;* ***IMean:*** *Impostor scores distribution mean;* ***ISTD:*** *Impostor scores distribution standard deviation;* ***AUC:*** *Area under the ROC curve;* ***SI:*** *Sensitivity Index;* ***JI:*** *Youden's J Index;* ***TH:*** *THreshold;* ***MCC:*** *Matthews Correlation Coefficient;* ***EER:*** *Equal Error Rate;* ***EERL:*** *EER low;* ***EERH:*** *EER high.*

### G. Supplementary results for the MSU-LAFIS comparison experiment

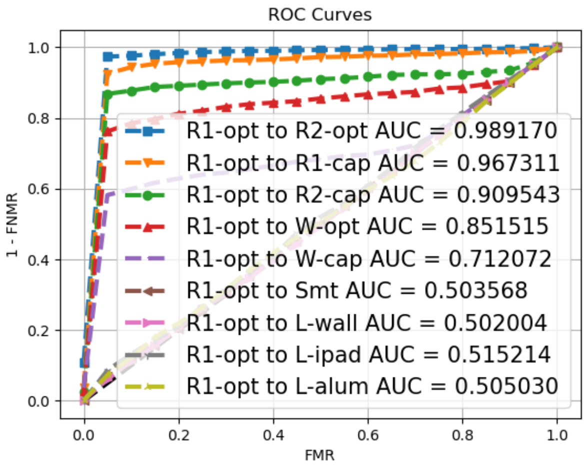


(a)

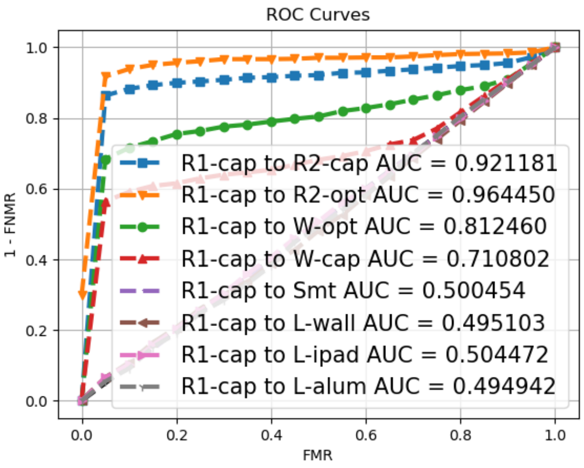


(b)

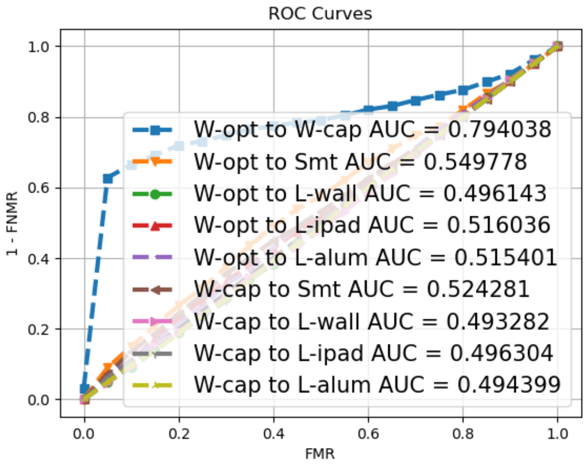


(c)

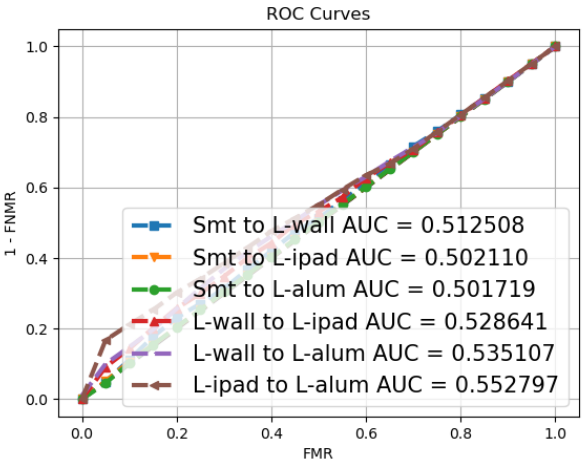


(d)

Fig. 66: ROC curve of the MSU-LAFIS comparison experiments for the 'Latent in the Wild' database

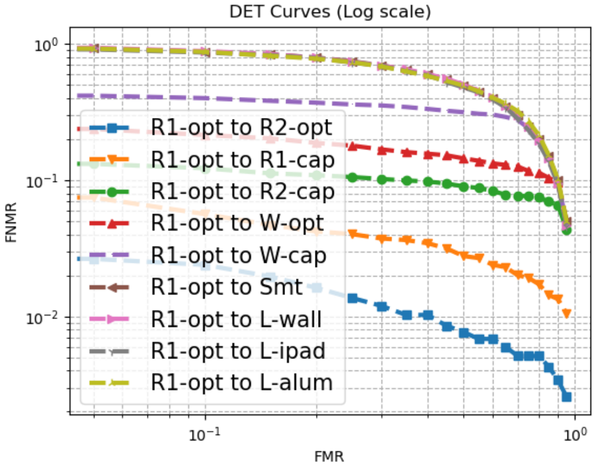


(a)

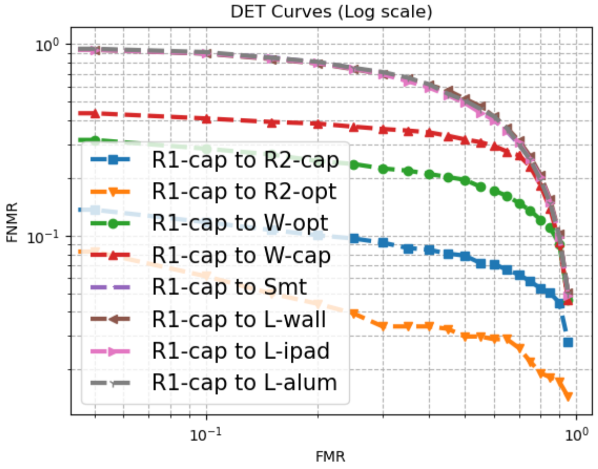


(b)

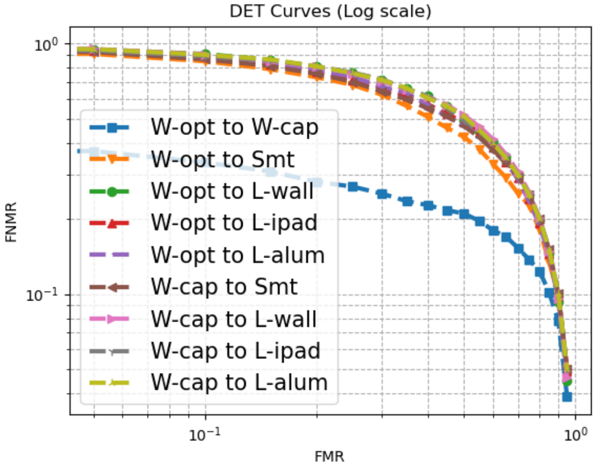


(c)

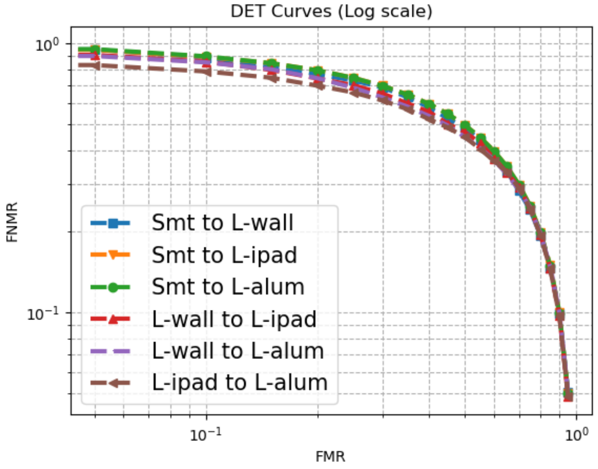


(d)

Fig. 67: DET curve of the MSU-LAFIS comparison experiments for the 'Latent in the Wild' database

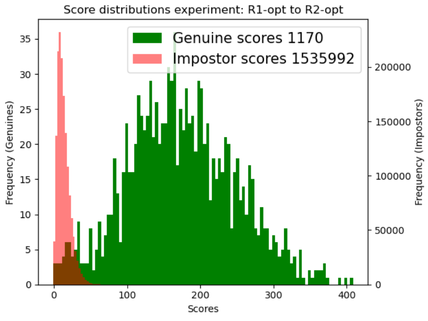


(a) R1-opt to R2-opt

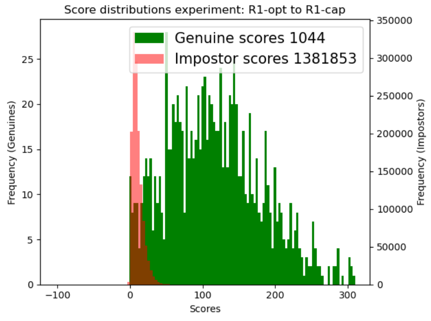


(b) R1-opt to R1-cap

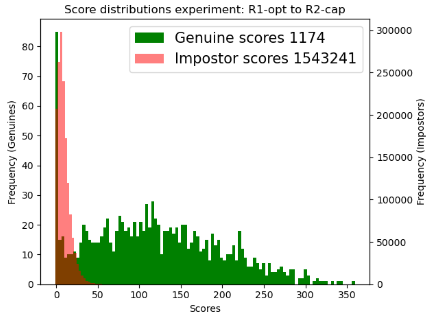


(c) R1-opt to R2-cap

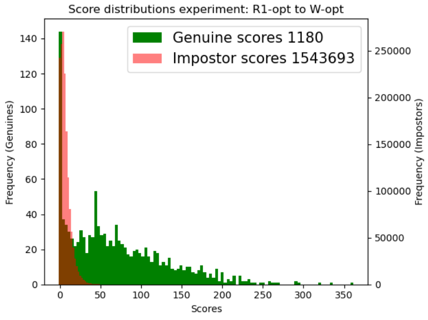


(d) R1-opt to W-opt

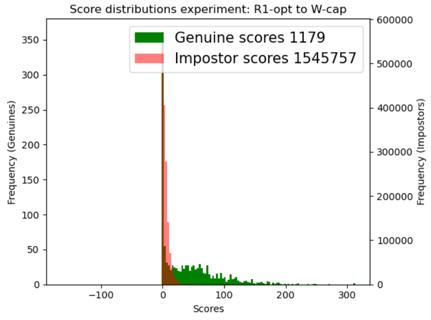


(e) R1-opt to W-cap

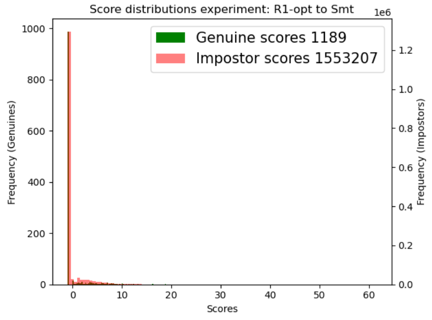


(f) R1-opt to Smt

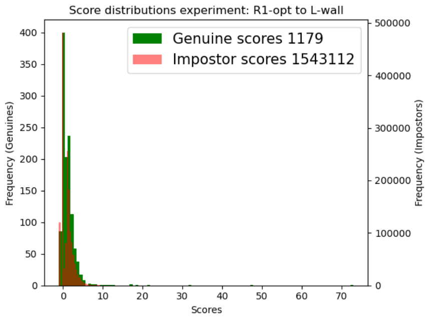


(g) R1-opt to L-wall

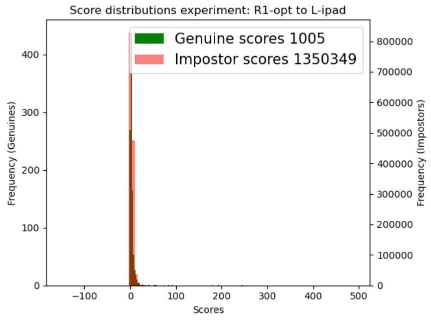


(h) R1-opt to L-ipad

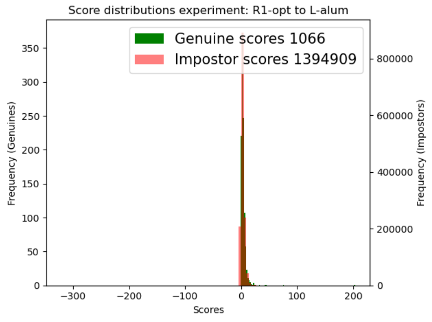


(i) R1-opt to L-alum

Fig. 68: Distributions of the MSU-LAFIS (part 1/4) comparison scores in the 'Latent in the Wild' database

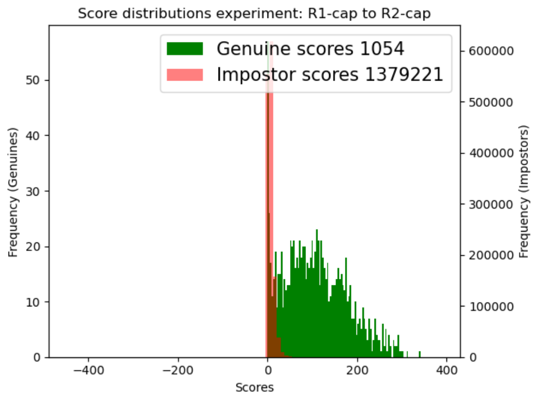


(a) R1-cap to R2-cap

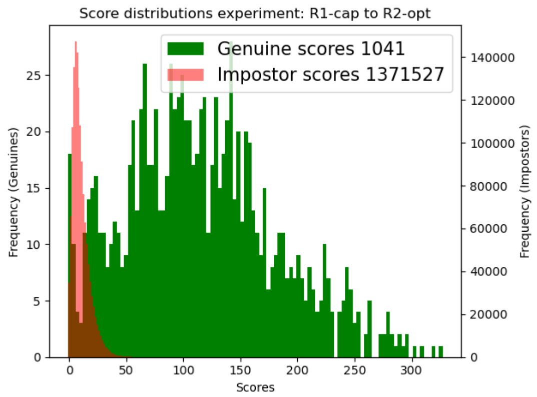


(b) R1-cap to R2-opt

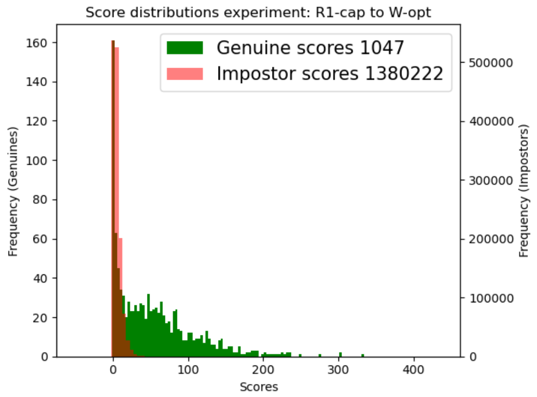


(c) R1-cap to W-opt

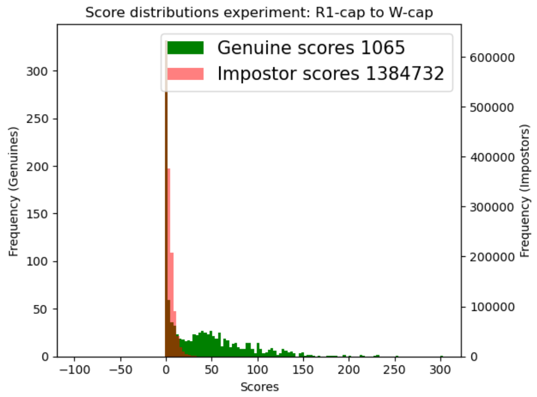


(d) R1-cap to W-cap

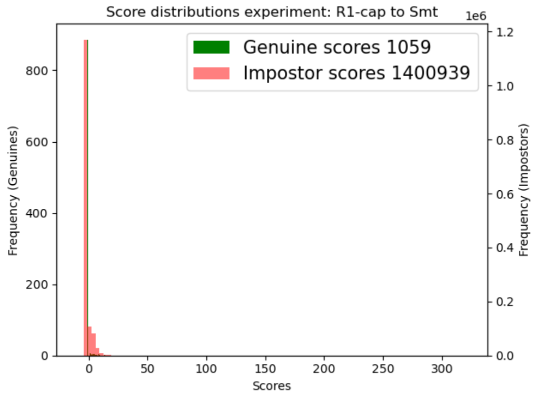


(e) R1-cap to Smt

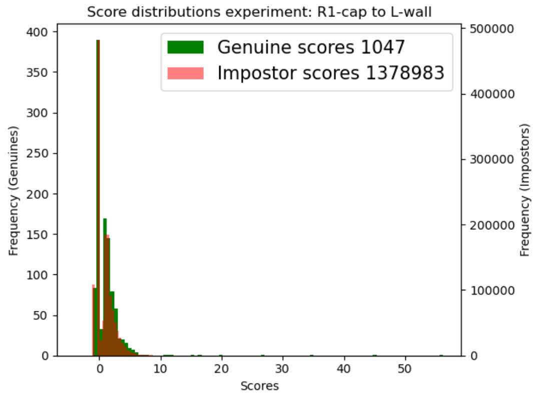


(f) R1-cap to L-wall

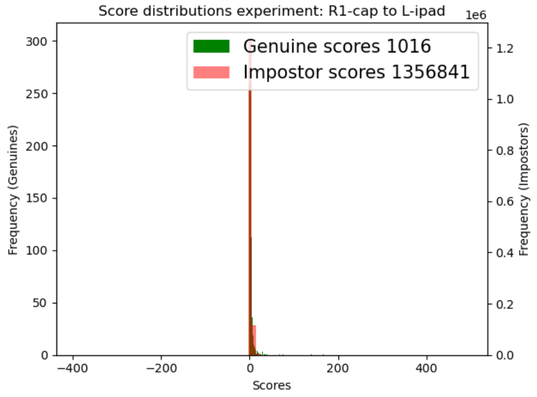


(g) R1-cap to L-ipad

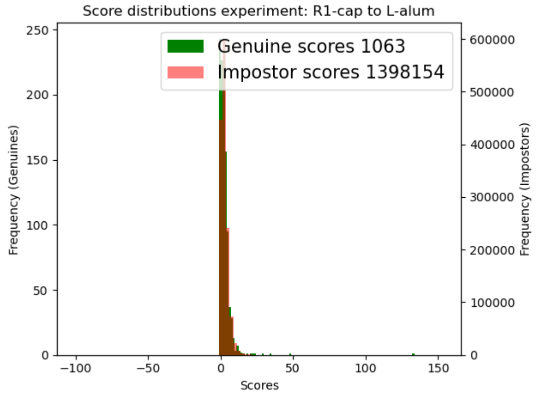


(h) R1-cap to L-alum

Fig. 69: Distributions of the MSU-LAFIS (part 2/4) comparison scores in the 'Latent in the Wild' database

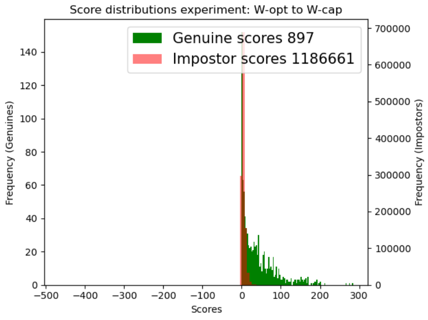


(a) W-opt to W-cap

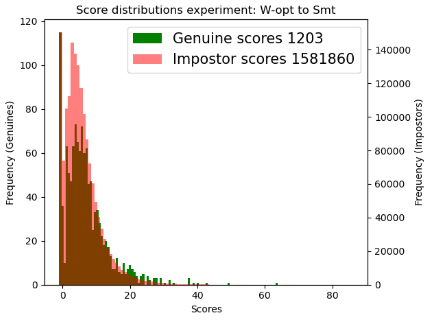


(b) W-opt to Smt

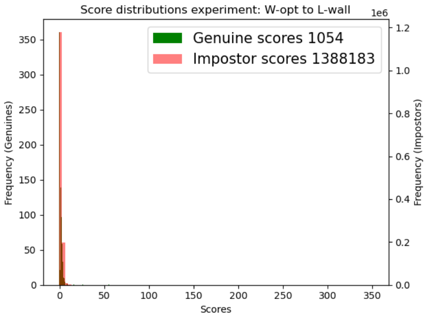


(c) W-opt to L-wall

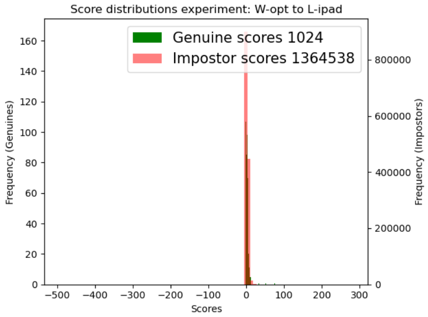


(d) W-opt to L-ipad

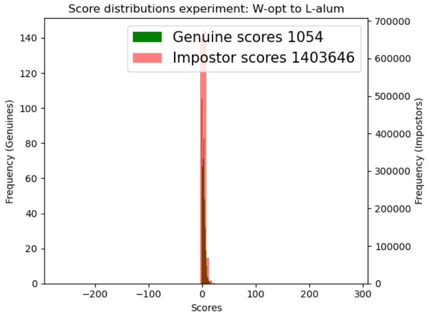


(e) W-opt to L-alum

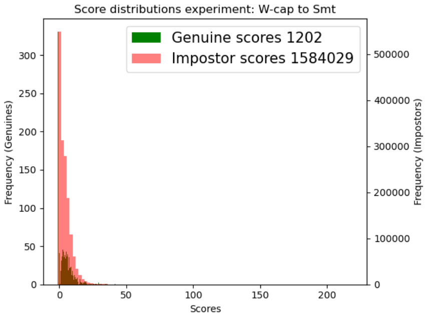


(f) W-cap to Smt

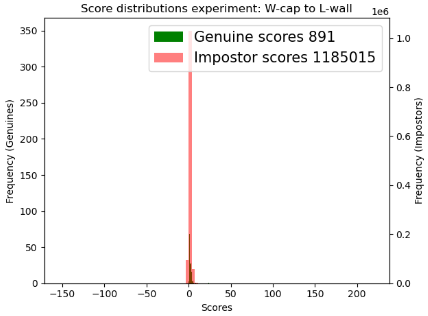


(g) W-cap to L-wall

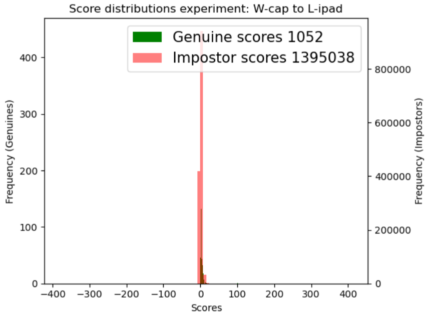


(h) W-cap to L-ipad

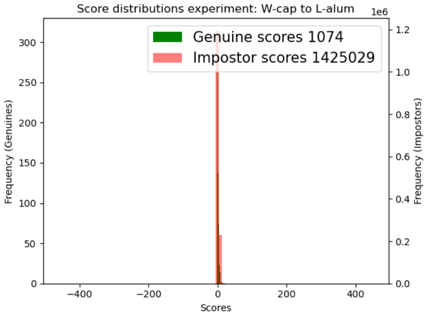


(i) W-cap to L-alum

Fig. 70: Distributions of the MSU-LAFIS (part 3/4) comparison scores in the 'Latent in the Wild' database

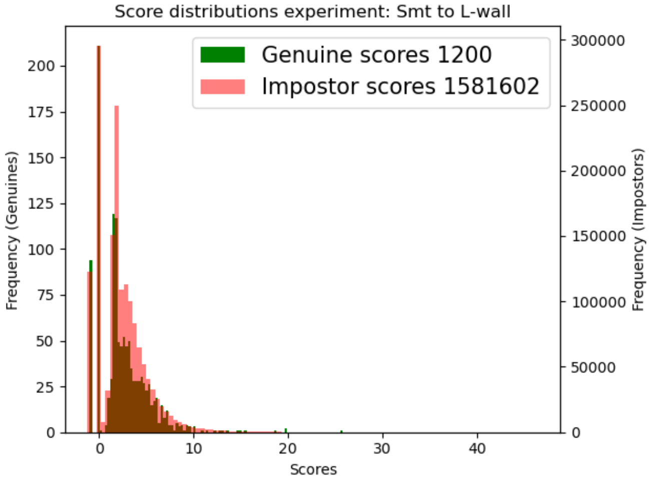


(a) Smt to L-wall

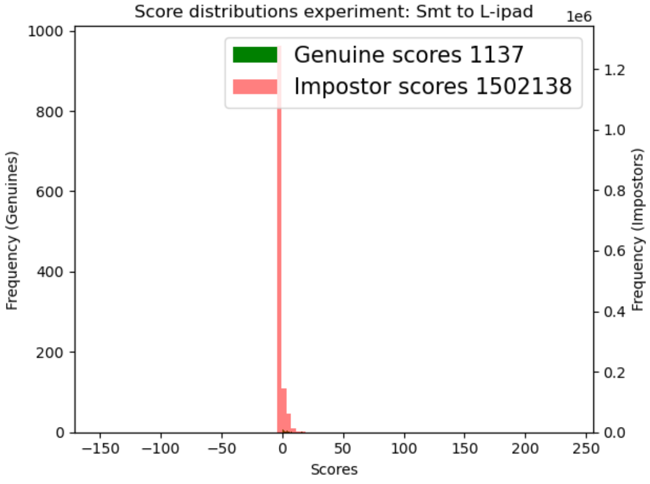


(b) Smt to L-ipad

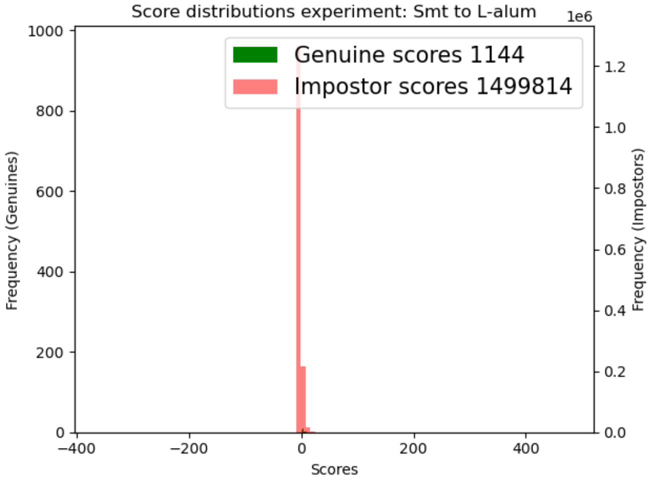


(c) Smt to L-alum

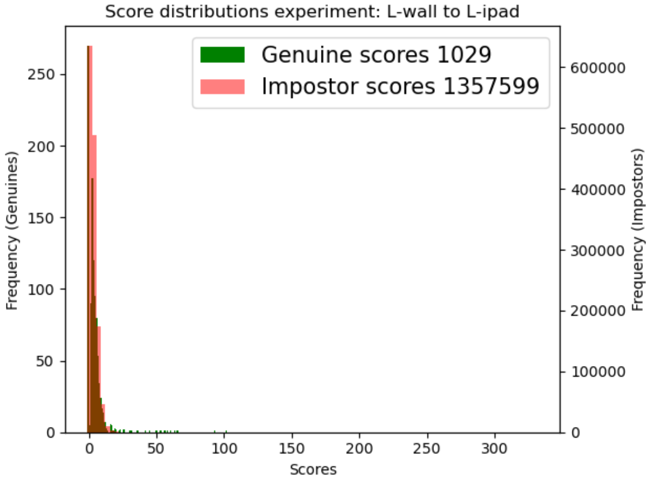


(d) L-wall to L-ipad

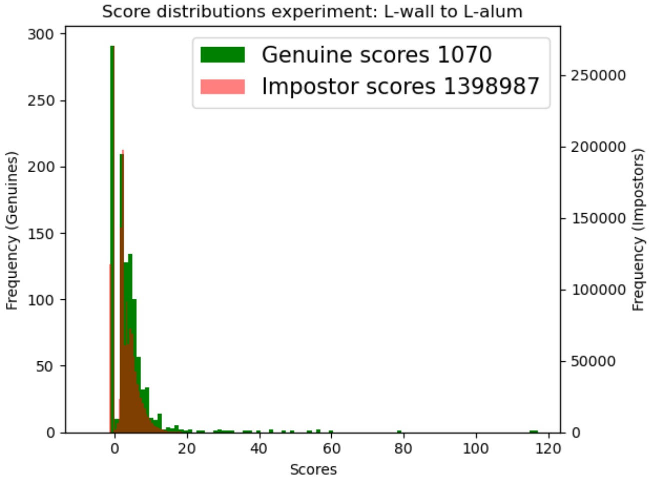


(e) L-wall to L-alum

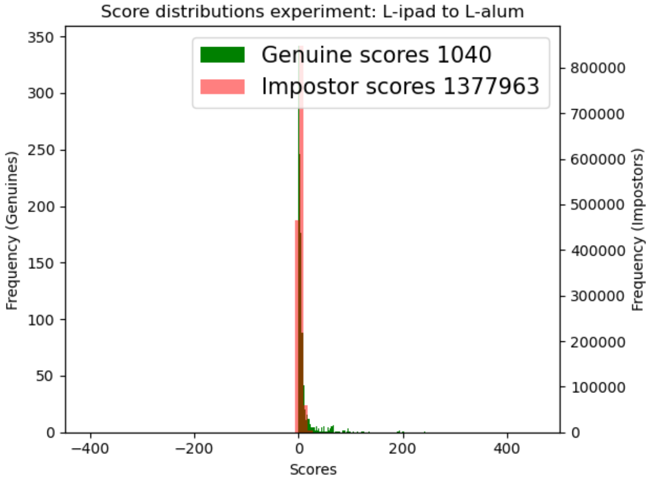


(f) L-ipad to L-alum

Fig. 71: Distributions of the MSU-LAFIS (part 4/4) comparison scores in the 'Latent in the Wild' database

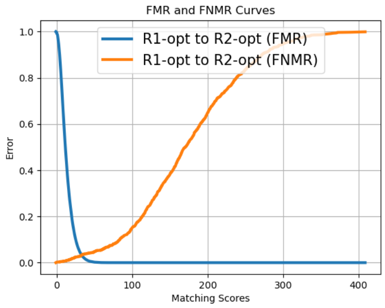


(a) R1-opt to R2-opt

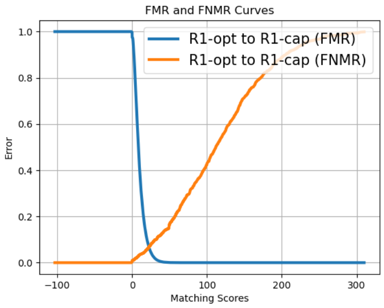


(b) R1-opt to R1-cap

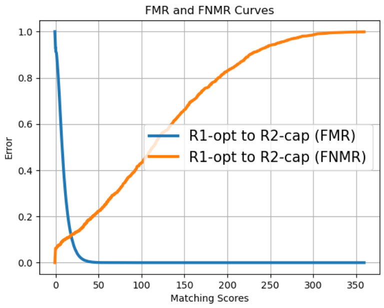


(c) R1-opt to R2-cap

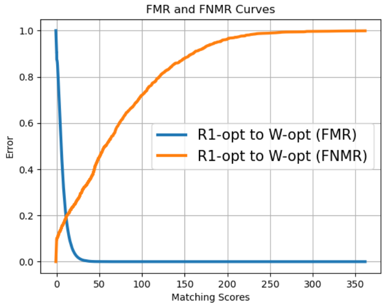


(d) R1-opt to W-opt

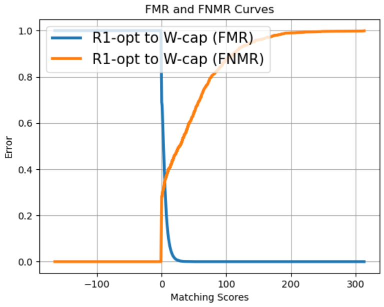


(e) R1-opt to W-cap

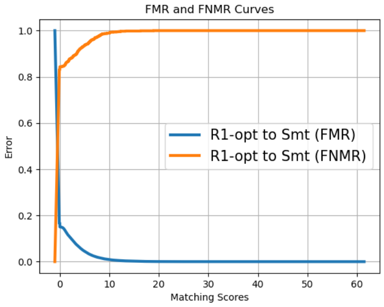


(f) R1-opt to Smt

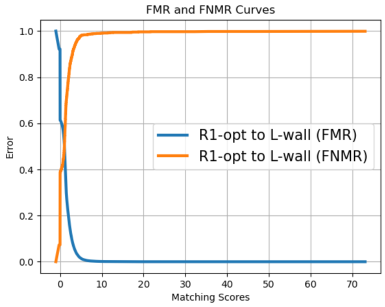


(g) R1-opt to L-wall

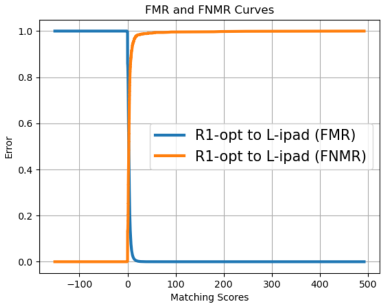


(h) R1-opt to L-ipad

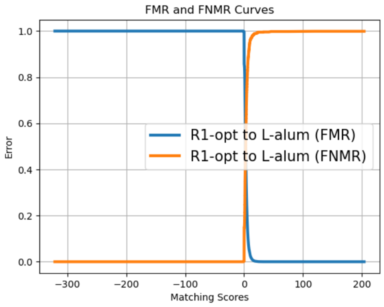


(i) R1-opt to L-alum

Fig. 72: FMR and FNMR curves of the MSU-LAFIS (part 1/4) comparison scores in the 'Latent in the Wild' database

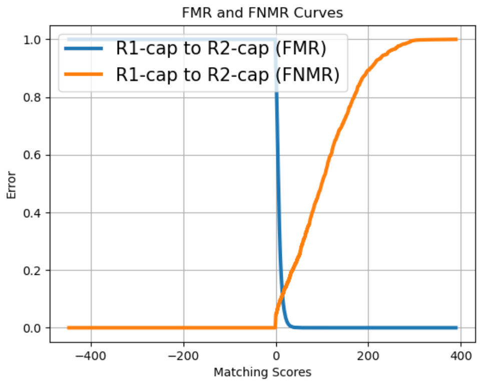


(a) R1-cap to R2-cap

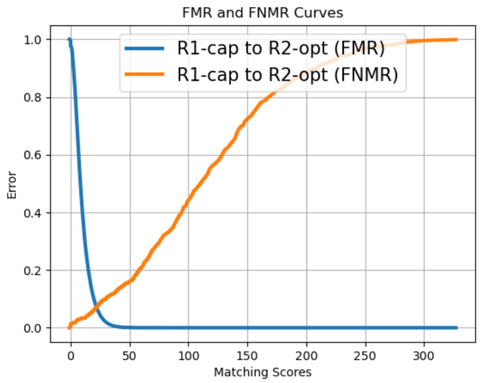


(b) R1-cap to R2-opt

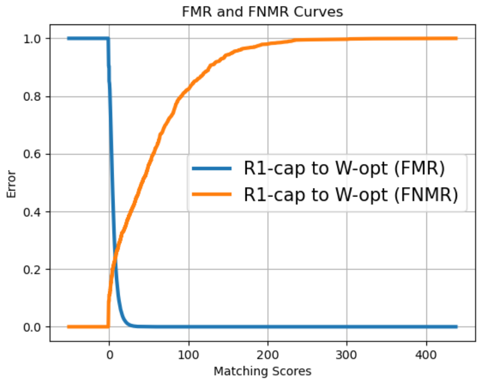


(c) R1-cap to W-opt

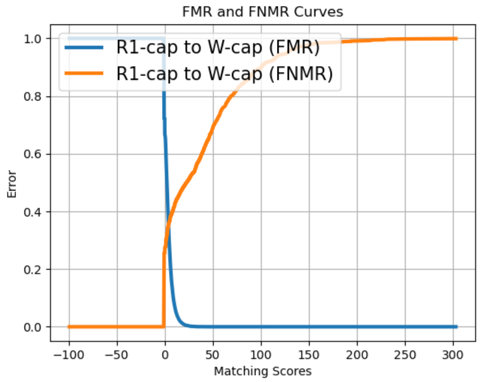


(d) R1-cap to W-cap

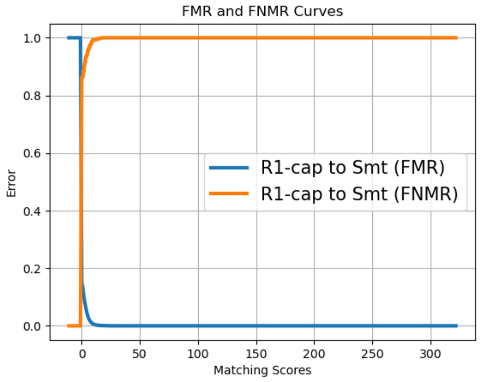


(e) R1-cap to Smt

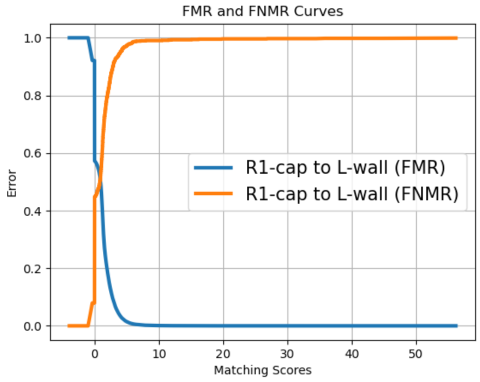


(f) R1-cap to L-wall

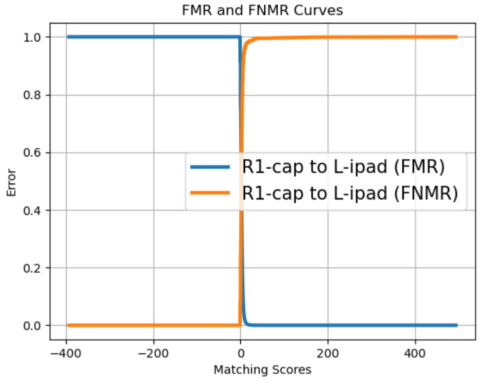


(g) R1-cap to L-ipad

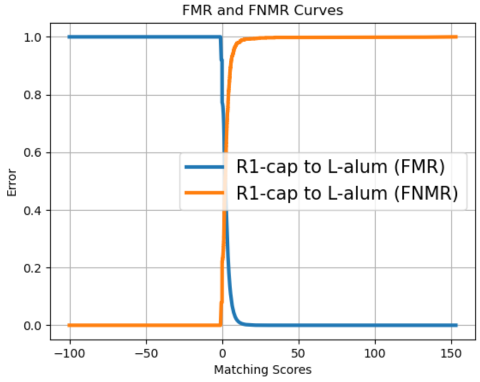


(h) R1-cap to L-alum

Fig. 73: FMR and FNMR curves of the MSU-LAFIS (part 2/4) comparison scores in the 'Latent in the Wild' database

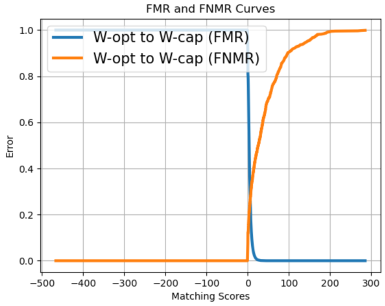


(a) W-opt to W-cap

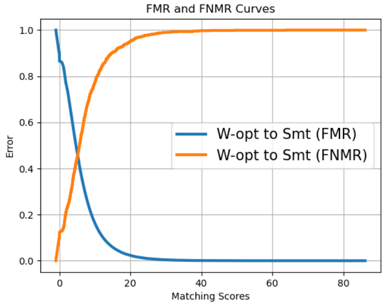


(b) W-opt to Smt

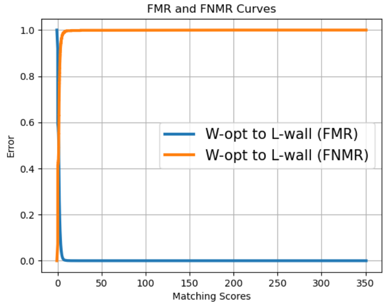


(c) W-opt to L-wall

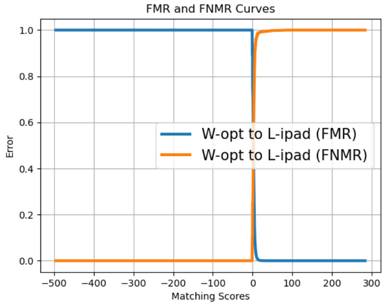


(d) W-opt to L-ipad

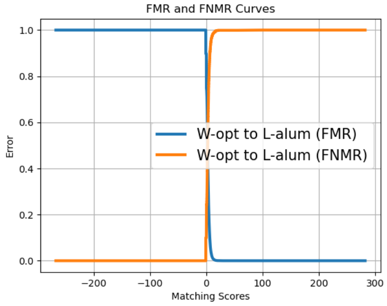


(e) W-opt to L-alum

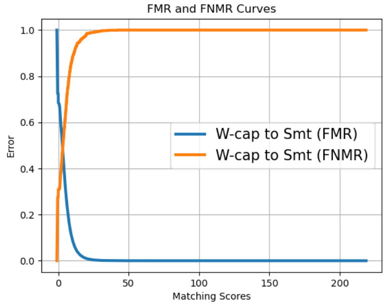


(f) W-cap to Smt

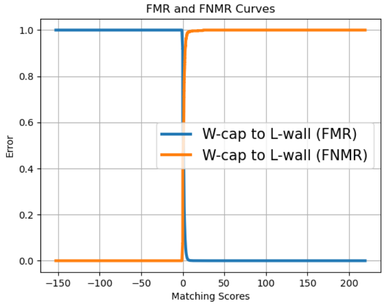


(g) W-cap to L-wall

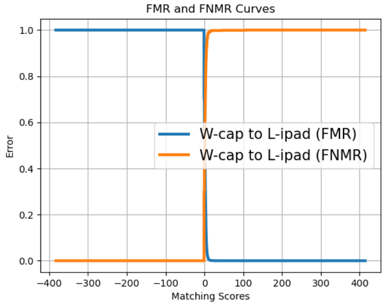


(h) W-cap to L-ipad

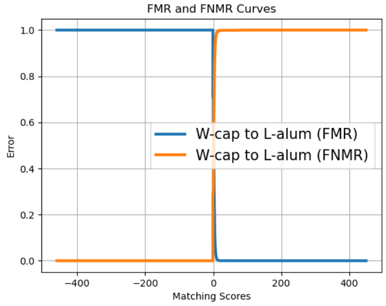


(i) W-cap to L-alum

Fig. 74: FMR and FNMR curves of the MSU-LAFIS (part 3/4) comparison scores in the 'Latent in the Wild' database

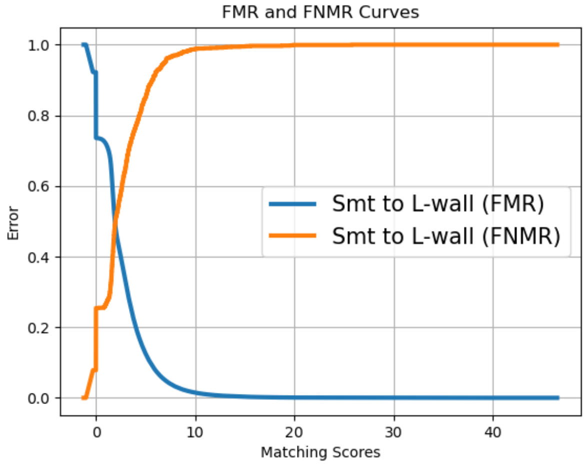


(a) Smt to L-wall

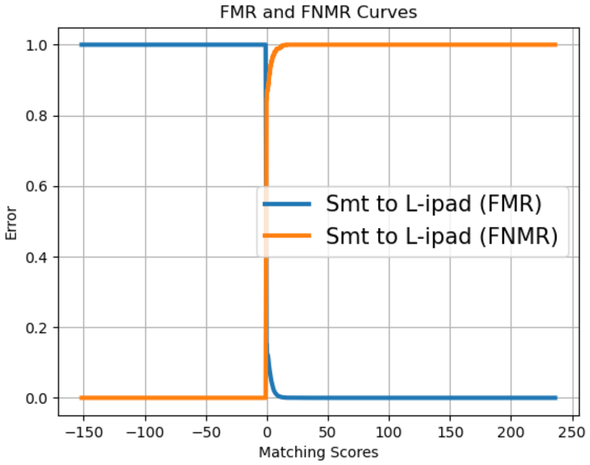


(b) Smt to L-ipad

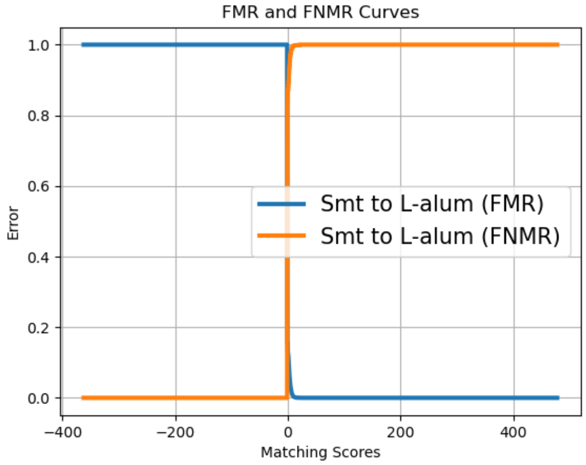


(c) Smt to L-alum

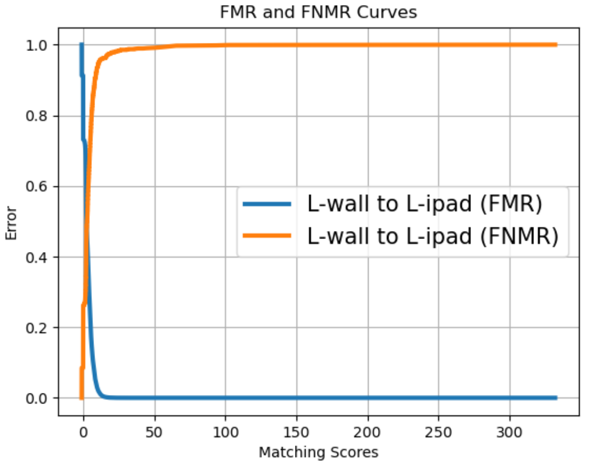


(d) L-wall to L-ipad

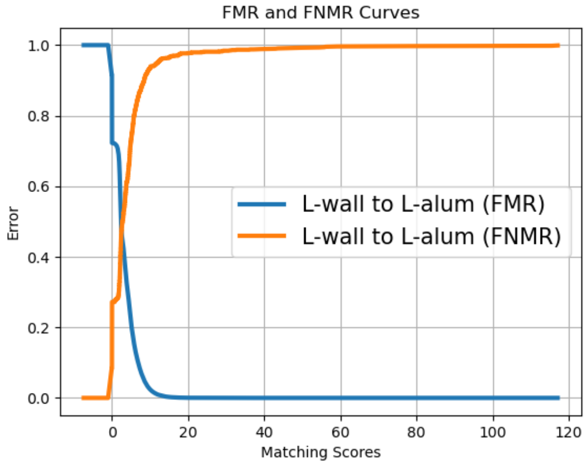


(e) L-wall to L-alum

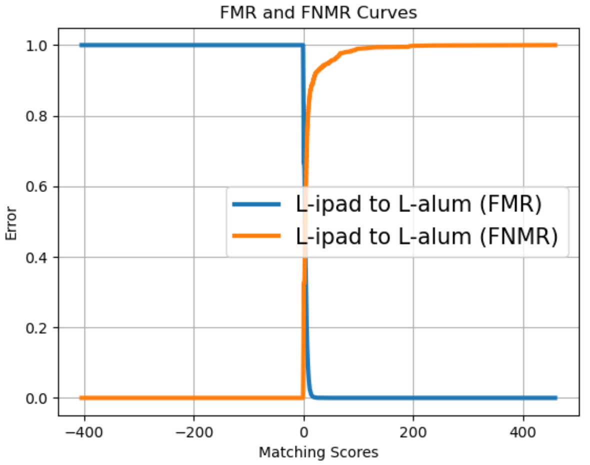


(f) L-ipad to L-alum

Fig. 75: FMR and FNMR curves of the MSU-LAFIS (part 4/4) comparison scores in the 'Latent in the Wild' database

TABLE XXXIII: Performance indicators measured on the 'Latent in the Wild' database for the MSU-LAFIS (part 1/4) comparison experiments.

| Comparison | GMean | GSTD | IMean | ISTD | SI | AUC | JI | JI_TH | MCC |
|---|---|---|---|---|---|---|---|---|---|
| R1-opt to R2-opt | 174.647 | 74.060 | 13.424 | 8.756 | 3.057 | 0.989 | 0.953 | 45.352 | 0.945 |
| R1-opt to R1-cap | 116.106 | 64.991 | 10.079 | 7.332 | 2.293 | 0.967 | 0.886 | 32.018 | 0.842 |
| R1-opt to R2-cap | 118.713 | 78.595 | 9.053 | 7.561 | 1.964 | 0.910 | 0.835 | 27.697 | 0.819 |
| R1-opt to W-opt | 70.624 | 61.247 | 6.679 | 6.371 | 1.469 | 0.852 | 0.719 | 21.850 | 0.670 |
| R1-opt to W-cap | 42.008 | 49.410 | 3.972 | 5.293 | 1.082 | 0.712 | 0.537 | 14.870 | 0.545 |
| R1-opt to Smt | -0.080 | 2.434 | -0.209 | 2.241 | 0.055 | 0.504 | 0.028 | 3.332 | 0.003 |
| R1-opt to L-wall | 1.279 | 3.210 | 1.071 | 1.428 | 0.084 | 0.502 | 0.016 | 2.910 | 0.041 |
| R1-opt to L-ipad | 4.545 | 12.952 | 3.166 | 3.072 | 0.146 | 0.515 | 0.040 | 9.334 | 0.071 |
| R1-opt to L-alum | 3.767 | 7.569 | 3.236 | 2.923 | 0.093 | 0.505 | 0.031 | 5.868 | 0.043 |
| | | | | | | | | | |
| Comparison | MCC_TH | EERL | EERH | EER | 0FMR | FMR1000 | FMR100 | FMR20 | FMR10 |
| R1-opt to R2-opt | 77.790 | 0.032 | 0.032 | 0.032 | 0.891 | 0.053 | 0.040 | 0.026 | 0.024 |
| R1-opt to R1-cap | 68.984 | 0.067 | 0.068 | 0.068 | 0.962 | 0.144 | 0.109 | 0.075 | 0.057 |
| R1-opt to R2-cap | 72.073 | 0.119 | 0.119 | 0.119 | 0.974 | 0.215 | 0.167 | 0.132 | 0.123 |
| R1-opt to W-opt | 63.570 | 0.192 | 0.192 | 0.192 | 0.971 | 0.370 | 0.296 | 0.238 | 0.215 |
| R1-opt to W-cap | 51.622 | 0.346 | 0.346 | 0.346 | 0.964 | 0.540 | 0.470 | 0.418 | 0.401 |
| R1-opt to Smt | 5.693 | 0.166 | 0.831 | 0.499 | 1.000 | 0.999 | 0.989 | 0.930 | 0.881 |
| R1-opt to L-wall | 47.148 | 0.503 | 0.503 | 0.503 | 0.998 | 0.992 | 0.983 | 0.940 | 0.889 |
| R1-opt to L-ipad | 74.223 | 0.491 | 0.491 | 0.491 | 0.994 | 0.985 | 0.967 | 0.914 | 0.868 |
| R1-opt to L-alum | 42.401 | 0.498 | 0.499 | 0.498 | 0.999 | 0.991 | 0.977 | 0.928 | 0.878 |
| | | | | | | | | | |
| Comparison | 0FNMR | EER_TH | 0FMR_TH | FMR1000_TH | FMR100_TH | FMR20_TH | FMR10_TH | 0FNMR_TH | |
| R1-opt to R2-opt | 1.000 | 33.199 | 268.675 | 54.212 | 40.753 | 30.241 | 25.300 | -1.000 | |
| R1-opt to R1-cap | 1.000 | 22.439 | 242.301 | 46.716 | 34.046 | 24.398 | 19.906 | -1.000 | |
| R1-opt to R2-cap | 1.000 | 17.824 | 282.658 | 47.507 | 33.848 | 23.606 | 19.016 | -1.000 | |
| R1-opt to W-opt | 1.000 | 11.056 | 210.913 | 41.376 | 28.403 | 19.023 | 14.916 | -1.000 | |
| R1-opt to W-cap | 1.000 | 4.813 | 156.060 | 34.188 | 22.217 | 14.128 | 10.710 | -1.000 | |
| R1-opt to Smt | 1.000 | -0.096 | 61.428 | 17.332 | 9.588 | 4.649 | 2.268 | -1.000 | |
| R1-opt to L-wall | 1.000 | 1.049 | 47.148 | 10.271 | 5.476 | 3.581 | 2.795 | -1.000 | |
| R1-opt to L-ipad | 1.000 | 2.622 | 74.223 | 26.357 | 14.531 | 8.465 | 6.479 | -1.000 | |
| R1-opt to L-alum | 1.000 | 2.689 | 203.951 | 21.807 | 13.642 | 8.597 | 6.704 | -1.000 | |

*Note: **GMean:** Genuine scores distribution mean; **GSTD:** Genuine scores distribution standard deviation; **IMean:** Impostor scores distribution mean; **ISTD:** Impostor scores distribution standard deviation; **AUC:** Area under the ROC curve; **SI:** Sensitivity Index; **JI:** Youden's J Index; **TH:** THreshold; **MCC:** Matthews Correlation Coefficient; **EER:** Equal Error Rate; **EERL:** EER low; **EERH:** EER high.*

TABLE XXXIV: Performance indicators measured on the 'Latent in the Wild' database for the MSU-LAFIS (part 2/4) comparison experiments.

| Comparison | GMean | GSTD | IMean | ISTD | SI | AUC | JI | JI_TH | MCC |
|---|---|---|---|---|---|---|---|---|---|
| R1-cap to R2-cap | 105.554 | 71.835 | 7.137 | 6.383 | 1.930 | 0.921 | 0.829 | 23.428 | 0.813 |
| R1-cap to R2-opt | 115.531 | 65.607 | 10.033 | 7.287 | 2.260 | 0.964 | 0.881 | 29.873 | 0.848 |
| R1-cap to W-opt | 53.689 | 53.097 | 5.327 | 5.323 | 1.282 | 0.812 | 0.639 | 18.814 | 0.622 |
| R1-cap to W-cap | 37.226 | 44.767 | 3.255 | 4.551 | 1.068 | 0.711 | 0.521 | 13.613 | 0.548 |
| R1-cap to Smt | -0.194 | 2.305 | -0.277 | 2.075 | 0.038 | 0.500 | 0.017 | 4.653 | 0.003 |
| R1-cap to L-wall | 1.199 | 3.067 | 1.006 | 1.421 | 0.081 | 0.495 | 0.018 | 3.733 | 0.046 |
| R1-cap to L-ipad | 3.276 | 8.878 | 2.474 | 2.810 | 0.122 | 0.504 | 0.023 | 10.089 | 0.055 |
| R1-cap to L-alum | 2.735 | 5.232 | 2.538 | 2.658 | 0.047 | 0.495 | 0.010 | 11.649 | 0.035 |
| | | | | | | | | | |
| Comparison | MCC_TH | EERL | EERH | EER | 0FMR | FMR1000 | FMR100 | FMR20 | FMR10 |
| R1-cap to R2-cap | 62.358 | 0.115 | 0.115 | 0.115 | 0.726 | 0.216 | 0.168 | 0.137 | 0.118 |
| R1-cap to R2-opt | 65.265 | 0.072 | 0.072 | 0.072 | 0.700 | 0.154 | 0.114 | 0.083 | 0.061 |
| R1-cap to W-opt | 52.410 | 0.240 | 0.240 | 0.240 | 0.904 | 0.456 | 0.373 | 0.316 | 0.285 |
| R1-cap to W-cap | 46.267 | 0.352 | 0.352 | 0.352 | 0.994 | 0.534 | 0.482 | 0.436 | 0.409 |
| R1-cap to Smt | 6.608 | 0.000 | 1.000 | 0.500 | 1.000 | 0.997 | 0.985 | 0.940 | 0.893 |
| R1-cap to L-wall | 34.465 | 0.508 | 0.508 | 0.508 | 0.998 | 0.990 | 0.979 | 0.934 | 0.892 |
| R1-cap to L-ipad | 68.060 | 0.496 | 0.496 | 0.496 | 1.000 | 0.986 | 0.970 | 0.934 | 0.897 |
| R1-cap to L-alum | 48.119 | 0.503 | 0.503 | 0.503 | 0.998 | 0.993 | 0.981 | 0.945 | 0.909 |
| | | | | | | | | | |
| Comparison | 0FNMR | EER_TH | 0FMR_TH | FMR1000_TH | FMR100_TH | FMR20_TH | FMR10_TH | 0FNMR_TH | |
| R1-cap to R2-cap | 1.000 | 14.551 | 150.095 | 41.703 | 28.723 | 19.399 | 15.365 | -1.000 | |
| R1-cap to R2-opt | 1.000 | 21.925 | 145.334 | 46.844 | 33.994 | 24.275 | 19.776 | -1.000 | |
| R1-cap to W-opt | 1.000 | 7.794 | 127.529 | 35.586 | 23.741 | 15.515 | 12.046 | -1.000 | |
| R1-cap to W-cap | 1.000 | 3.951 | 216.601 | 29.893 | 19.056 | 11.872 | 8.971 | -1.000 | |
| R1-cap to Smt | 1.000 | -1.000 | 321.815 | 15.705 | 8.723 | 4.220 | 1.964 | -1.000 | |
| R1-cap to L-wall | 1.000 | 0.903 | 44.905 | 9.634 | 5.456 | 3.577 | 2.774 | -1.000 | |
| R1-cap to L-ipad | 1.000 | 2.047 | 493.180 | 21.103 | 11.848 | 7.192 | 5.601 | -1.000 | |
| R1-cap to L-alum | 1.000 | 2.081 | 48.119 | 18.245 | 11.378 | 7.346 | 5.791 | -1.000 | |

*Note: **GMean:** Genuine scores distribution mean; **GSTD:** Genuine scores distribution standard deviation; **IMean:** Impostor scores distribution mean; **ISTD:** Impostor scores distribution standard deviation; **AUC:** Area under the ROC curve; **SI:** Sensitivity Index; **JI:** Youden's J Index; **TH:** THreshold; **MCC:** Matthews Correlation Coefficient; **EER:** Equal Error Rate; **EERL:** EER low; **EERH:** EER high.*

TABLE XXXV: Performance indicators measured on the 'Latent in the Wild' database for the MSU-LAFIS (part 3/4) comparison experiments.

| Comparison | GMean | GSTD | IMean | ISTD | SI | AUC | JI | JI_TH | MCC |
|---|---|---|---|---|---|---|---|---|---|
| W-opt to W-cap | 39.720 | 45.643 | 4.050 | 4.431 | 1.100 | 0.794 | 0.580 | 11.350 | 0.533 |
| W-opt to Smt | 6.898 | 6.705 | 5.702 | 5.403 | 0.196 | 0.550 | 0.092 | 5.274 | 0.007 |
| W-opt to L-wall | 1.202 | 2.410 | 1.131 | 1.543 | 0.035 | 0.496 | 0.008 | 7.601 | 0.018 |
| W-opt to L-ipad | 2.922 | 4.724 | 2.475 | 2.864 | 0.114 | 0.516 | 0.039 | 3.127 | 0.033 |
| W-opt to L-alum | 2.808 | 3.383 | 2.571 | 2.815 | 0.076 | 0.515 | 0.043 | 2.586 | 0.011 |
| W-cap to Smt | 4.337 | 5.605 | 3.702 | 4.793 | 0.122 | 0.524 | 0.058 | 4.829 | 0.004 |
| W-cap to L-wall | 1.058 | 1.913 | 1.014 | 1.459 | 0.026 | 0.493 | 0.007 | 4.659 | 0.020 |
| W-cap to L-ipad | 1.648 | 4.286 | 1.508 | 2.717 | 0.039 | 0.496 | 0.015 | 5.856 | 0.014 |
| W-cap to L-alum | 1.608 | 3.318 | 1.583 | 2.745 | 0.008 | 0.494 | 0.005 | 9.935 | 0.011 |
| | | | | | | | | | |
| Comparison | MCC_TH | EERL | EERH | EER | 0FMR | FMR1000 | FMR100 | FMR20 | FMR10 |
| W-opt to W-cap | 44.591 | 0.265 | 0.265 | 0.265 | 0.968 | 0.543 | 0.453 | 0.372 | 0.336 |
| W-opt to Smt | 63.754 | 0.455 | 0.456 | 0.455 | 1.000 | 0.994 | 0.978 | 0.910 | 0.851 |
| W-opt to L-wall | 55.498 | 0.498 | 0.498 | 0.498 | 1.000 | 0.995 | 0.983 | 0.951 | 0.910 |
| W-opt to L-ipad | 45.678 | 0.494 | 0.494 | 0.494 | 1.000 | 0.990 | 0.978 | 0.938 | 0.893 |
| W-opt to L-alum | 55.225 | 0.488 | 0.488 | 0.488 | 1.000 | 0.997 | 0.982 | 0.935 | 0.889 |
| W-cap to Smt | 18.280 | 0.483 | 0.484 | 0.484 | 1.000 | 0.998 | 0.978 | 0.928 | 0.866 |
| W-cap to L-wall | 23.994 | 0.510 | 0.510 | 0.510 | 1.000 | 0.994 | 0.987 | 0.953 | 0.907 |
| W-cap to L-ipad | 42.913 | 0.497 | 0.497 | 0.497 | 1.000 | 0.996 | 0.984 | 0.939 | 0.892 |
| W-cap to L-alum | 66.530 | 0.506 | 0.507 | 0.506 | 1.000 | 0.996 | 0.985 | 0.952 | 0.903 |
| | | | | | | | | | |
| Comparison | 0FNMR | EER_TH | 0FMR_TH | FMR1000_TH | FMR100_TH | FMR20_TH | FMR10_TH | 0FNMR_TH | |
| W-opt to W-cap | 1.000 | 5.648 | 160.441 | 30.432 | 19.618 | 12.397 | 9.489 | -1.000 | |
| W-opt to Smt | 1.000 | 5.152 | 86.175 | 37.593 | 24.570 | 15.823 | 12.321 | -1.000 | |
| W-opt to L-wall | 1.000 | 1.109 | 350.659 | 9.859 | 5.808 | 3.841 | 3.013 | -1.000 | |
| W-opt to L-ipad | 1.000 | 2.045 | 283.476 | 19.429 | 11.482 | 7.327 | 5.796 | -1.000 | |
| W-opt to L-alum | 1.000 | 2.190 | 281.964 | 17.970 | 11.538 | 7.597 | 6.043 | -1.000 | |
| W-cap to Smt | 1.000 | 3.090 | 218.794 | 31.756 | 19.878 | 12.521 | 9.674 | -1.000 | |
| W-cap to L-wall | 1.000 | 0.803 | 219.494 | 9.008 | 5.516 | 3.657 | 2.847 | -1.000 | |
| W-cap to L-ipad | 1.000 | 1.223 | 414.251 | 16.462 | 9.695 | 6.166 | 4.785 | -1.000 | |
| W-cap to L-alum | 1.000 | 1.233 | 449.250 | 15.664 | 9.826 | 6.372 | 4.979 | -1.000 | |

*Note:* ***GMean:*** *Genuine scores distribution mean;* ***GSTD:*** *Genuine scores distribution standard deviation;* ***IMean:*** *Impostor scores distribution mean;* ***ISTD:*** *Impostor scores distribution standard deviation;* ***AUC:*** *Area under the ROC curve;* ***SI:*** *Sensitivity Index;* ***JI:*** *Youden's J Index;* ***TH:*** *THreshold;* ***MCC:*** *Matthews Correlation Coefficient;* ***EER:*** *Equal Error Rate;* ***EERL:*** *EER low;* ***EERH:*** *EER high.*

TABLE XXXVI: Performance indicators measured on the ’Latent in the Wild’ database for the MSU-LAFIS (part 4/4) comparison experiments.

| Comparison | GMean | GSTD | IMean | ISTD | SI | AUC | JI | JI_TH | MCC |
|---|---|---|---|---|---|---|---|---|---|
| Smt to L-wall | 2.517 | 2.674 | 2.403 | 2.589 | 0.043 | 0.513 | 0.035 | 4.139 | 0.003 |
| Smt to L-ipad | -0.332 | 2.023 | -0.391 | 1.859 | 0.030 | 0.502 | 0.009 | 1.607 | 0.003 |
| Smt to L-alum | -0.369 | 1.875 | -0.366 | 1.947 | 0.002 | 0.502 | 0.008 | 1.885 | 0.002 |
| L-wall to L-ipad | 4.278 | 7.680 | 3.053 | 3.045 | 0.210 | 0.529 | 0.059 | 5.452 | 0.101 |
| L-wall to L-alum | 4.308 | 8.112 | 2.982 | 2.971 | 0.217 | 0.535 | 0.074 | 4.117 | 0.107 |
| L-ipad to L-alum | 8.483 | 21.256 | 3.022 | 3.601 | 0.358 | 0.553 | 0.120 | 10.077 | 0.220 |
| | | | | | | | | | |
| Comparison | MCC_TH | EERL | EERH | EER | 0FMR | FMR1000 | FMR100 | FMR20 | FMR10 |
| Smt to L-wall | 4.520 | 0.493 | 0.494 | 0.494 | 1.000 | 0.998 | 0.990 | 0.951 | 0.888 |
| Smt to L-ipad | 10.286 | 0.149 | 0.847 | 0.498 | 1.000 | 0.999 | 0.985 | 0.949 | 0.894 |
| Smt to L-alum | 21.920 | 0.155 | 0.841 | 0.498 | 1.000 | 0.998 | 0.991 | 0.955 | 0.898 |
| L-wall to L-ipad | 36.078 | 0.480 | 0.481 | 0.481 | 0.989 | 0.974 | 0.958 | 0.909 | 0.857 |
| L-wall to L-alum | 36.070 | 0.473 | 0.473 | 0.473 | 0.990 | 0.972 | 0.949 | 0.900 | 0.852 |
| L-ipad to L-alum | 44.393 | 0.470 | 0.470 | 0.470 | 0.971 | 0.916 | 0.882 | 0.833 | 0.788 |
| | | | | | | | | | |
| Comparison | 0FNMR | EER_TH | 0FMR_TH | FMR1000_TH | FMR100_TH | FMR20_TH | FMR10_TH | 0FNMR_TH | |
| Smt to L-wall | 1.000 | 1.939 | 46.490 | 19.243 | 11.129 | 6.977 | 5.479 | -1.000 | |
| Smt to L-ipad | 1.000 | -0.295 | 236.112 | 14.257 | 7.667 | 3.584 | 1.508 | -1.000 | |
| Smt to L-alum | 1.000 | -0.473 | 477.941 | 14.254 | 7.885 | 3.726 | 1.603 | -1.000 | |
| L-wall to L-ipad | 1.000 | 2.523 | 42.156 | 17.916 | 12.262 | 8.661 | 7.037 | -1.000 | |
| L-wall to L-alum | 1.000 | 2.508 | 42.987 | 17.399 | 11.950 | 8.467 | 6.894 | -1.000 | |
| L-ipad to L-alum | 1.000 | 2.598 | 64.323 | 21.263 | 13.844 | 9.474 | 7.660 | -1.000 | |

*Note: **GMean:** Genuine scores distribution mean; **GSTD:** Genuine scores distribution standard deviation; **IMean:** Impostor scores distribution mean; **ISTD:** Impostor scores distribution standard deviation; **AUC:** Area under the ROC curve; **SI:** Sensitivity Index; **JI:** Youden’s J Index; **TH:** THreshold; **MCC:** Matthews Correlation Coefficient; **EER:** Equal Error Rate; **EERL:** EER low; **EERH:** EER high.*
